# Supplementary material for: Benchmark for Anonymous Video Analytics
Source: arXiv:2009.14684 source file (2021-10-03)
Supplement: Supplementary file 1 [file appendix.tex]

\section*{Appendix A: Localization results per video}
\label{appendix:localization_results}

Localization results per video in
System 1-GPU in Table~\ref{tab:detection_results_S1gpu},
System 1-CPU in Table~\ref{tab:detection_results_S1cpu},
System 2-GPU in Table~\ref{tab:detection_results_S2gpu},
System 2-CPU in Table~\ref{tab:detection_results_S2cpu},
System 3 in Table~\ref{tab:detection_results_S3}, and
System 4 in Table~\ref{tab:detection_results_S4}.

% SYSTEM 1 - GPU
%=====================
\begin{table}[!t]
    \centering
    \footnotesize
    \setlength{\tabcolsep}{1pt}
    \caption{Localization results per video running algorithms in \textbf{System 1} with \textbf{GPU}. KEY -- Ax: algorithm x; P: precision; R: recall; F: F1-Score.}
    \label{tab:detection_results_S1gpu}
    \resizebox{\columnwidth}{!}{
        \begin{tabular}{lc|ccc|cc|ccc|c}
        \specialrule{1.2pt}{0.2pt}{1pt}
        \multicolumn{1}{c}{\multirow{2}{*}{Video}} & \multicolumn{1}{c|}{\multirow{2}{*}{Alg.}} & \multicolumn{1}{c}{\multirow{2}{*}{P}} & \multicolumn{1}{c}{\multirow{2}{*}{R}} & \multicolumn{1}{c|}{\multirow{2}{*}{F}} & \multicolumn{2}{c|}{Recall distance} &
        \multicolumn{3}{c|}{Recall occlusion} &
        \multicolumn{1}{|c}{\multirow{2}{*}{\begin{tabular}[c]{@{}c@{}}Speed\\ {[}seconds/frame{]}\end{tabular}}} \\
         &  &  &  &  & \multicolumn{1}{c}{Close}  & \multicolumn{1}{c|}{Far} & \multicolumn{1}{c}{No}  & \multicolumn{1}{c}{Partial}  & \multicolumn{1}{c|}{Heavy} & \\
        \specialrule{1.2pt}{0.2pt}{1pt}
        \multirow{4}{*}{Airport-1} & A1 &0.75 &0.84 &0.79 &0.99 &0.70 &0.85 &0.40 &0.13 &0.0414$\pm$0.0129 \\ 
        & A2 &0.88 &0.62 &0.72 &0.77 &0.46 &0.62 &0.06 &0.00 &0.0277$\pm$0.0030 \\ 
        & A3 &1.00 &0.80 &0.89 &0.98 &0.62 &0.86 &0.30 &0.75 &0.0845$\pm$0.0130 \\ 
        & A4 &0.98 &0.85 &0.91 &0.97 &0.72 &0.92 &0.28 &0.60 &0.0800$\pm$0.0006 \\ \hline 
        \multirow{4}{*}{Airport-2} & A1 &0.63 &0.99 &0.77 &0.99 &0.99 &1.00 &0.94 &0.56 &0.1728$\pm$0.0195 \\ 
        & A2 &0.99 &0.50 &0.67 &0.72 &0.29 &0.51 &0.03 &0.01 &0.0274$\pm$0.0049 \\ 
        & A3 &1.00 &0.82 &0.90 &0.97 &0.66 &0.90 &0.20 &0.64 &0.0828$\pm$0.0128 \\ 
        & A4 &0.99 &0.89 &0.93 &0.97 &0.81 &0.97 &0.55 &0.41 &0.0805$\pm$0.0009 \\ \hline 
        \multirow{4}{*}{Airport-3} & A1 &0.87 &0.80 &0.83 &0.95 &0.65 &0.84 &0.54 &0.15 &0.0408$\pm$0.0099 \\ 
        & A2 &0.98 &0.47 &0.64 &0.58 &0.37 &0.51 &0.06 &0.01 &0.0279$\pm$0.0037 \\ 
        & A3 &0.99 &0.71 &0.83 &0.95 &0.48 &0.88 &0.37 &0.48 &0.0876$\pm$0.0138 \\ 
        & A4 &0.98 &0.71 &0.82 &0.96 &0.45 &0.89 &0.26 &0.36 &0.0804$\pm$0.0008 \\ \hline 
        \multirow{4}{*}{Airport-4} & A1 &0.76 &0.79 &0.77 &0.92 &0.65 &0.81 &0.27 &0.20 &0.0416$\pm$0.0129 \\ 
        & A2 &0.96 &0.44 &0.61 &0.63 &0.26 &0.46 &0.06 &0.00 &0.0282$\pm$0.0057 \\ 
        & A3 &0.97 &0.77 &0.86 &0.94 &0.61 &0.92 &0.39 &0.54 &0.0835$\pm$0.0128 \\ 
        & A4 &0.94 &0.82 &0.88 &0.95 &0.68 &0.97 &0.51 &0.51 &0.0810$\pm$0.0008 \\ \hline \hline 
        \multirow{4}{*}{Mall-1} & A1 &0.67 &0.30 &0.42 &0.56 &0.03 &0.32 &0.07 &- &0.0413$\pm$0.0134 \\ 
        & A2 &0.81 &0.18 &0.30 &0.35 &0.01 &0.19 &0.02 &- &0.0393$\pm$0.0036 \\ 
        & A3 &0.84 &0.38 &0.52 &0.69 &0.07 &0.54 &0.16 &- &0.0923$\pm$0.0138 \\ 
        & A4 &0.71 &0.42 &0.53 &0.72 &0.12 &0.62 &0.14 &- &0.0814$\pm$0.0005 \\ \hline 
        \multirow{4}{*}{Mall-2} & A1 &0.27 &0.98 &0.43 &0.99 &0.97 &0.99 &0.89 &0.83 &0.1735$\pm$0.0235 \\ 
        & A2 &0.92 &0.15 &0.26 &0.30 &0.01 &0.16 &0.01 &0.00 &0.0391$\pm$0.0047 \\ 
        & A3 &0.86 &0.41 &0.56 &0.75 &0.09 &0.59 &0.18 &0.41 &0.0965$\pm$0.0146 \\ 
        & A4 &0.77 &0.45 &0.57 &0.80 &0.12 &0.65 &0.20 &0.22 &0.0815$\pm$0.0007 \\ \hline 
        \multirow{4}{*}{Mall-3} & A1 &0.32 &0.97 &0.49 &0.99 &0.95 &0.98 &0.89 &0.63 &0.1739$\pm$0.0192 \\ 
        & A2 &0.91 &0.52 &0.66 &0.83 &0.21 &0.54 &0.07 &0.00 &0.0446$\pm$0.0128 \\ 
        & A3 &0.90 &0.68 &0.77 &0.92 &0.44 &0.82 &0.34 &0.30 &0.0822$\pm$0.0126 \\ 
        & A4 &0.91 &0.76 &0.83 &0.93 &0.58 &0.91 &0.54 &0.23 &0.0809$\pm$0.0009 \\ \hline 
        \multirow{4}{*}{Mall-4} & A1 &0.44 &0.91 &0.59 &0.90 &0.92 &0.92 &0.78 &0.64 &0.1728$\pm$0.0183 \\ 
        & A2 &0.95 &0.27 &0.42 &0.38 &0.16 &0.28 &0.07 &0.00 &0.0465$\pm$0.0101 \\ 
        & A3 &0.93 &0.62 &0.74 &0.63 &0.62 &0.68 &0.28 &0.31 &0.0849$\pm$0.0121 \\ 
        & A4 &0.86 &0.68 &0.76 &0.61 &0.75 &0.75 &0.34 &0.36 &0.0805$\pm$0.0005 \\ \hline \hline 
        \multirow{4}{*}{Pedestrian-1} & A1 &0.76 &0.52 &0.61 &0.88 &0.15 &0.53 &0.05 &- &0.0419$\pm$0.0122 \\ 
        & A2 &0.97 &0.38 &0.55 &0.66 &0.11 &0.40 &0.00 &- &0.0505$\pm$0.0047 \\ 
        & A3 &0.99 &0.75 &0.86 &0.92 &0.59 &0.80 &0.34 &- &0.0828$\pm$0.0117 \\ 
        & A4 &0.98 &0.74 &0.84 &0.73 &0.75 &0.79 &0.33 &- &0.0811$\pm$0.0019 \\ \hline 
        \multirow{4}{*}{Pedestrian-2} & A1 &0.62 &0.51 &0.56 &0.81 &0.20 &0.55 &0.05 &0.05 &0.0421$\pm$0.0108 \\ 
        & A2 &0.93 &0.35 &0.51 &0.58 &0.13 &0.38 &0.01 &0.00 &0.0571$\pm$0.0032 \\ 
        & A3 &0.88 &0.55 &0.68 &0.75 &0.36 &0.70 &0.23 &0.18 &0.0839$\pm$0.0124 \\ 
        & A4 &0.86 &0.66 &0.75 &0.77 &0.55 &0.84 &0.28 &0.11 &0.0813$\pm$0.0007 \\ \hline 
        \multirow{4}{*}{Pedestrian-3} & A1 &0.39 &0.95 &0.55 &0.97 &0.94 &0.96 &0.88 &0.45 &0.1736$\pm$0.0187 \\ 
        & A2 &0.93 &0.36 &0.52 &0.58 &0.14 &0.37 &0.01 &0.00 &0.0522$\pm$0.0067 \\ 
        & A3 &1.00 &0.87 &0.93 &0.97 &0.78 &0.92 &0.57 &0.63 &0.0835$\pm$0.0138 \\ 
        & A4 &0.99 &0.90 &0.94 &0.95 &0.85 &0.96 &0.53 &0.43 &0.0808$\pm$0.0010 \\ \hline 
        \multirow{4}{*}{Pedestrian-4} & A1 &0.38 &0.94 &0.54 &0.99 &0.90 &0.96 &0.84 &0.45 &0.1755$\pm$0.0203 \\ 
        & A2 &0.60 &0.55 &0.57 &0.77 &0.33 &0.58 &0.04 &0.00 &0.0837$\pm$0.0059 \\ 
        & A3 &0.87 &0.72 &0.79 &0.83 &0.63 &0.81 &0.43 &0.53 &0.0871$\pm$0.0128 \\ 
        & A4 &0.86 &0.62 &0.72 &0.58 &0.67 &0.71 &0.26 &0.13 &0.0808$\pm$0.0007 \\ \hline 
        \multirow{4}{*}{Pedestrian-5} & A1 &0.88 &0.40 &0.55 &0.74 &0.05 &0.41 &0.25 &0.13 &0.0401$\pm$0.0162 \\ 
        & A2 &0.98 &0.22 &0.36 &0.42 &0.03 &0.25 &0.00 &0.00 &0.0699$\pm$0.0076 \\ 
        & A3 &0.99 &0.72 &0.84 &0.85 &0.59 &0.78 &0.41 &0.47 &0.0814$\pm$0.0118 \\ 
        & A4 &0.99 &0.84 &0.91 &0.93 &0.75 &0.91 &0.43 &0.53 &0.0813$\pm$0.0008 \\ \hline \hline 
        \multirow{4}{*}{Subway-1} & A1 &0.84 &0.74 &0.78 &0.94 &0.54 &0.78 &0.64 &0.39 &0.0414$\pm$0.0160 \\ 
        & A2 &0.97 &0.32 &0.48 &0.42 &0.21 &0.36 &0.09 &0.00 &0.0416$\pm$0.0045 \\ 
        & A3 &0.98 &0.70 &0.82 &0.92 &0.51 &0.82 &0.40 &0.45 &0.0901$\pm$0.0143 \\ 
        & A4 &0.85 &0.74 &0.79 &0.92 &0.57 &0.89 &0.35 &0.25 &0.0809$\pm$0.0006 \\ \hline 
        \multirow{4}{*}{Subway-2} & A1 &0.55 &0.96 &0.70 &0.99 &0.94 &0.97 &0.89 &0.65 &0.1753$\pm$0.0278 \\ 
        & A2 &0.99 &0.33 &0.50 &0.45 &0.22 &0.35 &0.05 &0.01 &0.0428$\pm$0.0034 \\ 
        & A3 &0.99 &0.58 &0.73 &0.85 &0.33 &0.70 &0.20 &0.41 &0.0930$\pm$0.0150 \\ 
        & A4 &0.96 &0.64 &0.77 &0.88 &0.41 &0.78 &0.21 &0.34 &0.0809$\pm$0.0006 \\ \hline 
        \multirow{4}{*}{Subway-3} & A1 &0.68 &0.72 &0.70 &0.87 &0.56 &0.77 &0.52 &0.29 &0.0459$\pm$0.0128 \\ 
        & A2 &0.95 &0.22 &0.36 &0.25 &0.20 &0.24 &0.13 &0.08 &0.0435$\pm$0.0049 \\ 
        & A3 &0.98 &0.61 &0.75 &0.90 &0.40 &0.74 &0.48 &0.61 &0.0888$\pm$0.0141 \\ 
        & A4 &0.97 &0.68 &0.80 &0.90 &0.50 &0.84 &0.49 &0.59 &0.0813$\pm$0.0009 \\ 
        \specialrule{1.2pt}{0.2pt}{1pt}
        \multirow{4}{*}{Overall} &A1 &0.61$\pm$0.19 &0.77$\pm$0.22 &0.63$\pm$0.13 &0.91$\pm$0.11 &0.63$\pm$0.34 &0.79$\pm$0.21 &0.56$\pm$0.32 &-$\pm$- &0.0996$\pm$0.0655 \\ 
        &A2 &0.92$\pm$0.10 &0.37$\pm$0.13 &0.51$\pm$0.13 &0.54$\pm$0.18 &0.20$\pm$0.12 &0.39$\pm$0.14 &0.04$\pm$0.04 &-$\pm$- &0.0451$\pm$0.0150 \\ 
        &A3 &0.95$\pm$0.06 &0.67$\pm$0.13 &0.78$\pm$0.11 &0.86$\pm$0.11 &0.49$\pm$0.19 &0.78$\pm$0.11 &0.33$\pm$0.11 &-$\pm$- &0.0866$\pm$0.0043 \\ 
        &A4 &0.91$\pm$0.08 &0.71$\pm$0.13 &0.80$\pm$0.11 &0.85$\pm$0.13 &0.58$\pm$0.21 &0.84$\pm$0.11 &0.36$\pm$0.13 &-$\pm$- &0.0809$\pm$0.0004 \\
        \specialrule{1.2pt}{0.2pt}{1pt}
        \end{tabular}
        }%
\end{table}
%=====================

% SYSTEM 1 - CPU
%=====================
\begin{table}[!t]
    \centering
    \footnotesize
    \setlength{\tabcolsep}{1pt}
    \caption{Localization results per video running algorithms in \textbf{System 1} with \textbf{CPU}. KEY -- Ax: algorithm x; P: precision; R: recall; F: F1-Score.}
    \label{tab:detection_results_S1cpu}
    \resizebox{\columnwidth}{!}{
        \begin{tabular}{lc|ccc|cc|ccc|c}
        \specialrule{1.2pt}{0.2pt}{1pt}
        \multicolumn{1}{c}{\multirow{2}{*}{Video}} & \multicolumn{1}{c|}{\multirow{2}{*}{Alg.}} & \multicolumn{1}{c}{\multirow{2}{*}{P}} & \multicolumn{1}{c}{\multirow{2}{*}{R}} & \multicolumn{1}{c|}{\multirow{2}{*}{F}} &
        \multicolumn{2}{c|}{Recall distance} &
        \multicolumn{3}{c|}{Recall occlusion} &
        \multicolumn{1}{|c}{\multirow{2}{*}{\begin{tabular}[c]{@{}c@{}}Speed\\ {[}seconds/frame{]}\end{tabular}}} \\
        &  &  &  &  & \multicolumn{1}{c}{Close}  & \multicolumn{1}{c|}{Far} & \multicolumn{1}{c}{No}  & \multicolumn{1}{c}{Partial}  & \multicolumn{1}{c|}{Heavy} & \\
        \specialrule{1.2pt}{0.2pt}{1pt}
        \multirow{4}{*}{Airport-1} & A1 &0.50 &0.88 &0.63 &0.99 &0.76 &0.88 &0.52 &0.19 &0.3925$\pm$0.1227 \\ 
        & A2 &0.88 &0.62 &0.73 &0.77 &0.46 &0.62 &0.05 &0.00 &0.1663$\pm$0.0160 \\ 
        & A3 &1.00 &0.79 &0.88 &0.98 &0.60 &0.85 &0.28 &0.73 &0.3335$\pm$0.0631 \\ 
        & A4 &0.98 &0.85 &0.91 &0.97 &0.72 &0.92 &0.28 &0.60 &2.0116$\pm$0.3191 \\ \hline 
        \multirow{4}{*}{Airport-2} & A1 &0.66 &0.83 &0.74 &0.99 &0.68 &0.85 &0.43 &0.14 &0.3637$\pm$0.0636 \\ 
        & A2 &0.99 &0.50 &0.67 &0.72 &0.29 &0.51 &0.03 &0.01 &0.1738$\pm$0.0218 \\ 
        & A3 &1.00 &0.81 &0.89 &0.97 &0.65 &0.90 &0.18 &0.57 &0.3368$\pm$0.0685 \\ 
        & A4 &0.99 &0.89 &0.93 &0.97 &0.81 &0.97 &0.55 &0.41 &2.0941$\pm$0.3358 \\ \hline 
        \multirow{4}{*}{Airport-3} & A1 &0.76 &0.84 &0.80 &0.96 &0.71 &0.88 &0.64 &0.21 &0.3457$\pm$0.0636 \\ 
        & A2 &0.98 &0.47 &0.64 &0.58 &0.37 &0.51 &0.06 &0.01 &0.1657$\pm$0.0208 \\ 
        & A3 &1.00 &0.69 &0.82 &0.95 &0.43 &0.86 &0.30 &0.45 &0.3336$\pm$0.0675 \\ 
        & A4 &0.98 &0.71 &0.82 &0.96 &0.45 &0.89 &0.26 &0.36 &2.4219$\pm$0.2964 \\ \hline 
        \multirow{4}{*}{Airport-4} & A1 &0.59 &0.83 &0.69 &0.94 &0.73 &0.86 &0.35 &0.25 &0.3759$\pm$0.0717 \\ 
        & A2 &0.96 &0.44 &0.61 &0.63 &0.25 &0.46 &0.06 &0.00 &0.1655$\pm$0.0191 \\ 
        & A3 &0.99 &0.75 &0.85 &0.94 &0.56 &0.91 &0.31 &0.47 &0.3715$\pm$0.0828 \\ 
        & A4 &0.94 &0.82 &0.88 &0.95 &0.68 &0.97 &0.51 &0.51 &2.1414$\pm$0.2992 \\ \hline \hline 
        \multirow{4}{*}{Mall-1} & A1 &0.46 &0.39 &0.43 &0.69 &0.08 &0.41 &0.13 &- &0.3488$\pm$0.0621 \\ 
        & A2 &0.81 &0.18 &0.30 &0.34 &0.01 &0.19 &0.02 &- &0.1830$\pm$0.0168 \\ 
        & A3 &0.87 &0.33 &0.48 &0.63 &0.03 &0.48 &0.10 &- &0.3812$\pm$0.0775 \\ 
        & A4 &0.71 &0.42 &0.53 &0.72 &0.12 &0.62 &0.14 &- &1.9623$\pm$0.3049 \\ \hline 
        \multirow{4}{*}{Mall-2} & A1 &0.35 &0.36 &0.36 &0.59 &0.13 &0.37 &0.12 &0.06 &0.3499$\pm$0.0618 \\ 
        & A2 &0.92 &0.15 &0.26 &0.30 &0.01 &0.16 &0.01 &0.00 &0.2113$\pm$0.0169 \\ 
        & A3 &0.89 &0.37 &0.52 &0.70 &0.05 &0.54 &0.12 &0.29 &0.4109$\pm$0.0970 \\ 
        & A4 &0.77 &0.45 &0.57 &0.80 &0.12 &0.65 &0.20 &0.22 &2.1933$\pm$0.2926 \\ \hline 
        \multirow{4}{*}{Mall-3} & A1 &0.74 &0.60 &0.67 &0.96 &0.25 &0.62 &0.22 &0.05 &0.3507$\pm$0.0621 \\ 
        & A2 &0.91 &0.52 &0.66 &0.83 &0.21 &0.54 &0.07 &0.00 &0.2292$\pm$0.0341 \\ 
        & A3 &0.97 &0.67 &0.79 &0.92 &0.41 &0.81 &0.30 &0.28 &0.3489$\pm$0.0718 \\ 
        & A4 &0.91 &0.76 &0.83 &0.93 &0.58 &0.91 &0.54 &0.23 &1.9104$\pm$0.2890 \\ \hline 
        \multirow{4}{*}{Mall-4} & A1 &0.66 &0.43 &0.52 &0.55 &0.30 &0.44 &0.25 &0.08 &0.3500$\pm$0.0622 \\ 
        & A2 &0.95 &0.27 &0.42 &0.38 &0.15 &0.28 &0.07 &0.00 &0.2354$\pm$0.0281 \\ 
        & A3 &0.98 &0.60 &0.74 &0.62 &0.58 &0.66 &0.24 &0.30 &0.3459$\pm$0.0690 \\ 
        & A4 &0.86 &0.68 &0.76 &0.61 &0.75 &0.75 &0.34 &0.36 &1.9705$\pm$0.3084 \\ \hline \hline 
        \multirow{4}{*}{Pedestrian-1} & A1 &0.51 &0.61 &0.55 &0.93 &0.27 &0.62 &0.10 &- &0.3639$\pm$0.0640 \\ 
        & A2 &0.98 &0.38 &0.55 &0.66 &0.10 &0.39 &0.00 &- &0.2038$\pm$0.0194 \\ 
        & A3 &1.00 &0.70 &0.82 &0.88 &0.53 &0.74 &0.32 &- &0.3392$\pm$0.0709 \\ 
        & A4 &0.98 &0.74 &0.84 &0.73 &0.75 &0.79 &0.33 &- &1.9328$\pm$0.2986 \\ \hline 
        \multirow{4}{*}{Pedestrian-2} & A1 &0.42 &0.58 &0.49 &0.84 &0.31 &0.62 &0.09 &0.09 &0.3584$\pm$0.0642 \\ 
        & A2 &0.94 &0.35 &0.51 &0.58 &0.13 &0.38 &0.01 &0.00 &0.2135$\pm$0.0177 \\ 
        & A3 &0.96 &0.55 &0.70 &0.76 &0.34 &0.70 &0.21 &0.16 &0.3635$\pm$0.0737 \\ 
        & A4 &0.86 &0.66 &0.75 &0.77 &0.55 &0.84 &0.28 &0.11 &2.4119$\pm$0.2963 \\ \hline 
        \multirow{4}{*}{Pedestrian-3} & A1 &0.55 &0.65 &0.60 &0.83 &0.47 &0.66 &0.32 &0.13 &0.3518$\pm$0.0622 \\ 
        & A2 &0.94 &0.36 &0.52 &0.58 &0.14 &0.37 &0.01 &0.00 &0.2386$\pm$0.0158 \\ 
        & A3 &1.00 &0.88 &0.93 &0.97 &0.78 &0.93 &0.57 &0.62 &0.3506$\pm$0.0677 \\ 
        & A4 &0.99 &0.90 &0.94 &0.95 &0.85 &0.96 &0.53 &0.43 &2.3447$\pm$0.3042 \\ \hline 
        \multirow{4}{*}{Pedestrian-4} & A1 &0.56 &0.74 &0.64 &0.95 &0.53 &0.76 &0.49 &0.31 &0.3464$\pm$0.0623 \\ 
        & A2 &0.60 &0.55 &0.57 &0.77 &0.33 &0.58 &0.04 &0.00 &0.3219$\pm$0.0184 \\ 
        & A3 &0.95 &0.64 &0.76 &0.70 &0.59 &0.72 &0.34 &0.32 &0.3512$\pm$0.0689 \\ 
        & A4 &0.86 &0.62 &0.72 &0.58 &0.67 &0.71 &0.26 &0.13 &2.4137$\pm$0.2887 \\ \hline 
        \multirow{4}{*}{Pedestrian-5} & A1 &0.58 &0.47 &0.52 &0.82 &0.11 &0.49 &0.33 &0.20 &0.4089$\pm$0.0741 \\ 
        & A2 &0.98 &0.22 &0.36 &0.41 &0.03 &0.24 &0.00 &0.00 &0.2371$\pm$0.0231 \\ 
        & A3 &1.00 &0.67 &0.80 &0.80 &0.54 &0.73 &0.35 &0.42 &0.3497$\pm$0.0666 \\ 
        & A4 &0.99 &0.84 &0.91 &0.93 &0.75 &0.91 &0.43 &0.53 &1.9676$\pm$0.3057 \\ \hline \hline 
        \multirow{4}{*}{Subway-1} & A1 &0.66 &0.78 &0.72 &0.95 &0.61 &0.81 &0.74 &0.52 &0.3444$\pm$0.0625 \\ 
        & A2 &0.97 &0.32 &0.48 &0.42 &0.21 &0.36 &0.09 &0.00 &0.1887$\pm$0.0144 \\ 
        & A3 &0.99 &0.70 &0.82 &0.92 &0.52 &0.82 &0.42 &0.49 &0.4354$\pm$0.1147 \\ 
        & A4 &0.85 &0.74 &0.79 &0.92 &0.57 &0.89 &0.35 &0.25 &1.9687$\pm$0.3078 \\ \hline 
        \multirow{4}{*}{Subway-2} & A1 &0.63 &0.61 &0.62 &0.88 &0.33 &0.63 &0.33 &0.20 &0.3437$\pm$0.0626 \\ 
        & A2 &0.99 &0.33 &0.50 &0.45 &0.21 &0.35 &0.05 &0.00 &0.2219$\pm$0.0112 \\ 
        & A3 &1.00 &0.58 &0.73 &0.86 &0.32 &0.71 &0.20 &0.43 &0.4505$\pm$0.1067 \\ 
        & A4 &0.96 &0.64 &0.77 &0.88 &0.41 &0.78 &0.21 &0.34 &2.2229$\pm$0.2957 \\ \hline 
        \multirow{4}{*}{Subway-3} & A1 &0.50 &0.77 &0.60 &0.90 &0.63 &0.82 &0.62 &0.38 &0.4373$\pm$0.0795 \\ 
        & A2 &0.96 &0.22 &0.36 &0.25 &0.20 &0.24 &0.13 &0.08 &0.1914$\pm$0.0176 \\ 
        & A3 &0.97 &0.61 &0.75 &0.89 &0.40 &0.74 &0.47 &0.65 &0.4573$\pm$0.1079 \\ 
        & A4 &0.97 &0.68 &0.80 &0.90 &0.50 &0.84 &0.49 &0.59 &2.0628$\pm$0.3074 \\ \hline 
        \specialrule{1.2pt}{0.2pt}{1pt}
        \multirow{4}{*}{Overall} &A1 &0.57$\pm$0.11 &0.65$\pm$0.16 &0.60$\pm$0.11 &0.86$\pm$0.13 &0.43$\pm$0.23 &0.67$\pm$0.17 &0.35$\pm$0.20 &-$\pm$- &0.3645$\pm$0.0259 \\ 
         &A2 &0.92$\pm$0.09 &0.37$\pm$0.13 &0.51$\pm$0.13 &0.54$\pm$0.18 &0.19$\pm$0.12 &0.39$\pm$0.14 &0.04$\pm$0.04 &-$\pm$- &0.2092$\pm$0.0387 \\ 
         &A3 &0.97$\pm$0.04 &0.65$\pm$0.14 &0.77$\pm$0.12 &0.84$\pm$0.12 &0.46$\pm$0.20 &0.76$\pm$0.12 &0.30$\pm$0.12 &-$\pm$- &0.3725$\pm$0.0411 \\ 
         &A4 &0.91$\pm$0.08 &0.71$\pm$0.13 &0.80$\pm$0.11 &0.85$\pm$0.13 &0.58$\pm$0.21 &0.84$\pm$0.11 &0.36$\pm$0.13 &-$\pm$- &2.1269$\pm$0.1797 \\ 
        \specialrule{1.2pt}{0.2pt}{1pt}
        \end{tabular}
        }%
\end{table}
%=====================

% SYSTEM 2 - GPU
%=====================
\begin{table}[!t]
    \centering
    \footnotesize
    \setlength{\tabcolsep}{1pt}
    \caption{Localization results per video running algorithms in \textbf{System 2} with \textbf{GPU}. KEY -- Ax: algorithm x; P: precision; R: recall; F: F1-Score.}
    \label{tab:detection_results_S2gpu}
    \resizebox{\columnwidth}{!}{
        \begin{tabular}{lc|ccc|cc|ccc|c}
        \specialrule{1.2pt}{0.2pt}{1pt}
        \multicolumn{1}{c}{\multirow{2}{*}{Video}} & \multicolumn{1}{c|}{\multirow{2}{*}{Alg.}} & \multicolumn{1}{c}{\multirow{2}{*}{P}} & \multicolumn{1}{c}{\multirow{2}{*}{R}} & \multicolumn{1}{c|}{\multirow{2}{*}{F}} & \multicolumn{2}{c|}{Recall distance} &
        \multicolumn{3}{c|}{Recall occlusion} &
        \multicolumn{1}{|c}{\multirow{2}{*}{\begin{tabular}[c]{@{}c@{}}Speed\\ {[}seconds/frame{]}\end{tabular}}} \\
         &  &  &  &  & \multicolumn{1}{c}{Close}  & \multicolumn{1}{c|}{Far} & \multicolumn{1}{c}{No}  & \multicolumn{1}{c}{Partial}  & \multicolumn{1}{c|}{Heavy} & \\
        \specialrule{1.2pt}{0.2pt}{1pt}
         \multirow{4}{*}{Airport-1} & A1 &0.56 &0.99 &0.71 &1.00 &0.99 &1.00 &0.80 &0.57 &0.1668$\pm$0.0134 \\ 
        & A2 &0.88 &0.62 &0.72 &0.77 &0.46 &0.62 &0.06 &0.00 &0.0493$\pm$0.0025 \\ 
        & A3 &1.00 &0.80 &0.89 &0.98 &0.62 &0.86 &0.30 &0.75 &0.0625$\pm$0.0134 \\ 
        & A4 &0.98 &0.85 &0.91 &0.97 &0.72 &0.92 &0.28 &0.60 &0.0817$\pm$0.0009 \\ \hline
         \multirow{4}{*}{Airport-2} & A1 &0.63 &0.99 &0.77 &0.99 &0.99 &1.00 &0.94 &0.56 &0.1669$\pm$0.0130 \\ 
        & A2 &0.99 &0.50 &0.67 &0.72 &0.29 &0.51 &0.03 &0.01 &0.0501$\pm$0.0048 \\ 
        & A3 &1.00 &0.82 &0.90 &0.97 &0.66 &0.90 &0.20 &0.64 &0.0602$\pm$0.0124 \\ 
        & A4 &0.99 &0.89 &0.93 &0.97 &0.81 &0.97 &0.55 &0.41 &0.0817$\pm$0.0010 \\ \hline
         \multirow{4}{*}{Airport-3} & A1 &0.81 &0.95 &0.87 &0.99 &0.91 &0.97 &0.93 &0.55 &0.1668$\pm$0.0123 \\ 
        & A2 &0.98 &0.47 &0.64 &0.58 &0.37 &0.51 &0.06 &0.01 &0.0492$\pm$0.0034 \\ 
        & A3 &0.99 &0.71 &0.83 &0.95 &0.48 &0.88 &0.37 &0.48 &0.0627$\pm$0.0131 \\ 
        & A4 &0.98 &0.71 &0.82 &0.96 &0.45 &0.89 &0.26 &0.36 &0.0816$\pm$0.0009 \\ \hline
         \multirow{4}{*}{Airport-4} & A1 &0.63 &0.97 &0.77 &0.98 &0.96 &0.98 &0.91 &0.66 &0.1667$\pm$0.0134 \\ 
        & A2 &0.96 &0.44 &0.61 &0.63 &0.26 &0.46 &0.06 &0.00 &0.0505$\pm$0.0057 \\ 
        & A3 &0.97 &0.77 &0.86 &0.94 &0.61 &0.92 &0.39 &0.54 &0.0590$\pm$0.0065 \\ 
        & A4 &0.94 &0.82 &0.88 &0.95 &0.68 &0.97 &0.51 &0.51 &0.0822$\pm$0.0008 \\ \hline \hline
        \multirow{4}{*}{Mall-1} & A1 &0.23 &0.97 &0.38 &0.99 &0.94 &0.98 &0.85 &- &0.1676$\pm$0.0142 \\ 
        & A2 &0.81 &0.18 &0.30 &0.35 &0.01 &0.19 &0.02 &- &0.0601$\pm$0.0034 \\ 
        & A3 &0.84 &0.38 &0.52 &0.69 &0.07 &0.54 &0.16 &- &0.0631$\pm$0.0070 \\ 
        & A4 &0.71 &0.42 &0.53 &0.72 &0.12 &0.62 &0.14 &- &0.0829$\pm$0.0008 \\ \hline
        \multirow{4}{*}{Mall-2} & A1 &0.27 &0.98 &0.43 &0.99 &0.97 &0.99 &0.89 &0.83 &0.1676$\pm$0.0159 \\ 
        & A2 &0.92 &0.15 &0.26 &0.30 &0.01 &0.16 &0.01 &0.00 &0.0612$\pm$0.0045 \\ 
        & A3 &0.86 &0.41 &0.56 &0.75 &0.09 &0.59 &0.18 &0.41 &0.0654$\pm$0.0081 \\ 
        & A4 &0.77 &0.45 &0.57 &0.80 &0.12 &0.65 &0.20 &0.22 &0.0831$\pm$0.0009 \\ \hline
        \multirow{4}{*}{Mall-3} & A1 &0.32 &0.97 &0.49 &0.99 &0.95 &0.98 &0.89 &0.63 &0.1670$\pm$0.0130 \\ 
        & A2 &0.91 &0.52 &0.66 &0.83 &0.21 &0.54 &0.07 &0.00 &0.0678$\pm$0.0127 \\ 
        & A3 &0.90 &0.68 &0.77 &0.92 &0.44 &0.82 &0.34 &0.30 &0.0584$\pm$0.0074 \\ 
        & A4 &0.91 &0.76 &0.83 &0.93 &0.58 &0.91 &0.54 &0.23 &0.0819$\pm$0.0009 \\ \hline
        \multirow{4}{*}{Mall-4} & A1 &0.44 &0.91 &0.59 &0.90 &0.92 &0.92 &0.78 &0.64 &0.1672$\pm$0.0124 \\ 
        & A2 &0.95 &0.27 &0.42 &0.38 &0.16 &0.28 &0.07 &0.00 &0.0695$\pm$0.0099 \\ 
        & A3 &0.93 &0.62 &0.74 &0.63 &0.62 &0.68 &0.28 &0.31 &0.0591$\pm$0.0077 \\ 
        & A4 &0.86 &0.68 &0.76 &0.61 &0.75 &0.75 &0.34 &0.36 &0.0822$\pm$0.0008 \\ \hline \hline
        \multirow{4}{*}{Pedestrian-1} & A1 &0.30 &0.97 &0.46 &0.99 &0.95 &0.98 &0.63 &- &0.1671$\pm$0.0126 \\ 
        & A2 &0.97 &0.38 &0.55 &0.66 &0.11 &0.40 &0.00 &- &0.0710$\pm$0.0043 \\ 
        & A3 &0.99 &0.75 &0.86 &0.92 &0.59 &0.80 &0.34 &- &0.0574$\pm$0.0073 \\ 
        & A4 &0.98 &0.74 &0.84 &0.73 &0.75 &0.79 &0.33 &- &0.0820$\pm$0.0009 \\ \hline 
        \multirow{4}{*}{Pedestrian-2} & A1 &0.29 &0.94 &0.44 &0.98 &0.91 &0.97 &0.70 &0.39 &0.1669$\pm$0.0122 \\ 
        & A2 &0.93 &0.35 &0.51 &0.58 &0.13 &0.38 &0.01 &0.00 &0.0774$\pm$0.0030 \\ 
        & A3 &0.88 &0.55 &0.68 &0.75 &0.36 &0.70 &0.23 &0.18 &0.0592$\pm$0.0061 \\ 
        & A4 &0.86 &0.66 &0.75 &0.77 &0.55 &0.84 &0.28 &0.11 &0.0823$\pm$0.0008 \\ \hline 
        \multirow{4}{*}{Pedestrian-3} & A1 &0.39 &0.95 &0.55 &0.97 &0.94 &0.96 &0.88 &0.45 &0.1687$\pm$0.0128 \\ 
        & A2 &0.93 &0.36 &0.52 &0.58 &0.14 &0.37 &0.01 &0.00 &0.0741$\pm$0.0062 \\ 
        & A3 &1.00 &0.87 &0.93 &0.97 &0.78 &0.92 &0.57 &0.63 &0.0635$\pm$0.0132 \\ 
        & A4 &0.99 &0.90 &0.94 &0.95 &0.85 &0.96 &0.53 &0.43 &0.0817$\pm$0.0009 \\ \hline 
        \multirow{4}{*}{Pedestrian-4} & A1 &0.38 &0.94 &0.54 &0.99 &0.90 &0.96 &0.84 &0.45 &0.1685$\pm$0.0144 \\ 
        & A2 &0.60 &0.55 &0.57 &0.77 &0.33 &0.58 &0.04 &0.00 &0.1035$\pm$0.0058 \\ 
        & A3 &0.87 &0.72 &0.79 &0.83 &0.63 &0.81 &0.43 &0.53 &0.0594$\pm$0.0071 \\ 
        & A4 &0.86 &0.62 &0.72 &0.58 &0.67 &0.71 &0.26 &0.13 &0.0819$\pm$0.0008 \\ \hline 
        \multirow{4}{*}{Pedestrian-5} & A1 &0.73 &0.92 &0.82 &0.98 &0.87 &0.93 &0.93 &0.73 &0.1667$\pm$0.0176 \\ 
        & A2 &0.98 &0.22 &0.36 &0.42 &0.03 &0.25 &0.00 &0.00 &0.0891$\pm$0.0074 \\ 
        & A3 &0.99 &0.72 &0.84 &0.85 &0.59 &0.78 &0.41 &0.47 &0.0575$\pm$0.0067 \\ 
        & A4 &0.99 &0.84 &0.91 &0.93 &0.75 &0.91 &0.43 &0.53 &0.0821$\pm$0.0008 \\ \hline \hline 
        \multirow{4}{*}{Subway-1} & A1 &0.64 &0.95 &0.77 &0.99 &0.91 &0.99 &0.96 &0.66 &0.1791$\pm$0.0171 \\ 
        & A2 &0.97 &0.32 &0.48 &0.42 &0.21 &0.36 &0.09 &0.00 &0.0619$\pm$0.0042 \\ 
        & A3 &0.98 &0.70 &0.82 &0.92 &0.51 &0.82 &0.40 &0.45 &0.0623$\pm$0.0084 \\ 
        & A4 &0.85 &0.74 &0.79 &0.92 &0.57 &0.89 &0.35 &0.25 &0.0823$\pm$0.0008 \\ \hline 
        \multirow{4}{*}{Subway-2} & A1 &0.55 &0.96 &0.70 &0.99 &0.94 &0.97 &0.89 &0.65 &0.1690$\pm$0.0192 \\ 
        & A2 &0.99 &0.33 &0.50 &0.45 &0.22 &0.35 &0.05 &0.01 &0.0645$\pm$0.0034 \\ 
        & A3 &0.99 &0.58 &0.73 &0.85 &0.33 &0.70 &0.20 &0.41 &0.0629$\pm$0.0059 \\ 
        & A4 &0.96 &0.64 &0.77 &0.88 &0.41 &0.78 &0.21 &0.34 &0.0826$\pm$0.0008 \\ \hline 
        \multirow{4}{*}{Subway-3} & A1 &0.56 &0.94 &0.71 &0.99 &0.90 &0.98 &0.94 &0.65 &0.1687$\pm$0.0128 \\ 
        & A2 &0.95 &0.22 &0.36 &0.25 &0.20 &0.24 &0.13 &0.08 &0.0644$\pm$0.0041 \\ 
        & A3 &0.98 &0.61 &0.75 &0.90 &0.40 &0.74 &0.48 &0.61 &0.0649$\pm$0.0083 \\ 
        & A4 &0.97 &0.68 &0.80 &0.90 &0.50 &0.84 &0.49 &0.59 &0.0825$\pm$0.0009 \\ \hline 
        \specialrule{1.2pt}{0.2pt}{1pt}
        \multirow{4}{*}{Overall} &A1 &0.48$\pm$0.17 &0.96$\pm$0.02 &0.62$\pm$0.15 &0.98$\pm$0.02 &0.93$\pm$0.03 &0.97$\pm$0.02 &0.86$\pm$0.09 &-$\pm$- &0.1682$\pm$0.0029 \\ 
         &A2 &0.92$\pm$0.10 &0.37$\pm$0.13 &0.51$\pm$0.13 &0.54$\pm$0.18 &0.20$\pm$0.12 &0.39$\pm$0.14 &0.04$\pm$0.04 &-$\pm$- &0.0665$\pm$0.0144 \\ 
         &A3 &0.95$\pm$0.06 &0.67$\pm$0.13 &0.78$\pm$0.11 &0.86$\pm$0.11 &0.49$\pm$0.19 &0.78$\pm$0.11 &0.33$\pm$0.11 &-$\pm$- &0.0611$\pm$0.0025 \\ 
         &A4 &0.91$\pm$0.08 &0.71$\pm$0.13 &0.80$\pm$0.11 &0.85$\pm$0.13 &0.58$\pm$0.21 &0.84$\pm$0.11 &0.36$\pm$0.13 &-$\pm$- &0.0822$\pm$0.0004 \\ 
        \specialrule{1.2pt}{0.2pt}{1pt}
        \end{tabular}
        }%
\end{table}
%=====================

% SYSTEM 2 - CPU
%=====================
\begin{table}[!t]
    \centering
    \footnotesize
    \setlength{\tabcolsep}{1pt}
    \caption{Localization results per video running algorithms in \textbf{System 2} with \textbf{CPU}. KEY -- Ax: algorithm x; P: precision; R: recall; F: F1-Score.}
    \label{tab:detection_results_S2cpu}
    \resizebox{\columnwidth}{!}{
        \begin{tabular}{lc|ccc|cc|ccc|c}
        \specialrule{1.2pt}{0.2pt}{1pt}
        \multicolumn{1}{c}{\multirow{2}{*}{Video}} & \multicolumn{1}{c|}{\multirow{2}{*}{Alg.}} & \multicolumn{1}{c}{\multirow{2}{*}{P}} & \multicolumn{1}{c}{\multirow{2}{*}{R}} & \multicolumn{1}{c|}{\multirow{2}{*}{F}} &
        \multicolumn{2}{c|}{Recall distance} &
        \multicolumn{3}{c|}{Recall occlusion} &
        \multicolumn{1}{|c}{\multirow{2}{*}{\begin{tabular}[c]{@{}c@{}}Speed\\ {[}seconds/frame{]}\end{tabular}}} \\
        &  &  &  &  & \multicolumn{1}{c}{Close}  & \multicolumn{1}{c|}{Far} & \multicolumn{1}{c}{No}  & \multicolumn{1}{c}{Partial}  & \multicolumn{1}{c|}{Heavy} & \\
        \specialrule{1.2pt}{0.2pt}{1pt}
        \multirow{4}{*}{Airport-1} & A1 &0.55 &0.99 &0.71 &1.00 &0.99 &1.00 &0.82 &0.57 &1.9726$\pm$0.0401 \\ 
        & A2 &0.89 &0.61 &0.72 &0.77 &0.45 &0.62 &0.09 &0.00 &0.2807$\pm$0.0095 \\ 
        & A3 &0.97 &0.77 &0.86 &0.95 &0.60 &0.83 &0.22 &0.71 &0.2718$\pm$0.0698 \\ 
        & A4 &0.98 &0.60 &0.74 &0.72 &0.48 &0.65 &0.11 &0.00 &0.7566$\pm$0.0415 \\ \hline 
        \multirow{4}{*}{Airport-2} & A1 &0.63 &0.99 &0.77 &0.99 &0.98 &1.00 &1.00 &0.48 &2.0224$\pm$0.0386 \\ 
        & A2 &1.00 &0.50 &0.67 &0.71 &0.29 &0.51 &0.08 &0.00 &0.2743$\pm$0.0136 \\ 
        & A3 &0.98 &0.81 &0.89 &0.96 &0.66 &0.90 &0.19 &0.65 &0.2685$\pm$0.0725 \\ 
        & A4 &0.99 &0.65 &0.78 &0.75 &0.55 &0.72 &0.38 &0.10 &0.7523$\pm$0.0433 \\ \hline 
        \multirow{4}{*}{Airport-3} & A1 &0.81 &0.96 &0.88 &1.00 &0.92 &0.97 &0.98 &0.61 &2.0834$\pm$0.0465 \\ 
        & A2 &0.98 &0.47 &0.63 &0.58 &0.36 &0.51 &0.05 &0.00 &0.2741$\pm$0.0112 \\ 
        & A3 &0.94 &0.67 &0.78 &0.90 &0.43 &0.82 &0.35 &0.41 &0.2747$\pm$0.0681 \\ 
        & A4 &0.99 &0.46 &0.63 &0.65 &0.28 &0.59 &0.11 &0.12 &0.7489$\pm$0.0486 \\ \hline  
        \multirow{4}{*}{Airport-4} & A1 &0.63 &0.97 &0.76 &0.98 &0.96 &0.98 &0.95 &0.51 &2.0103$\pm$0.0341 \\ 
        & A2 &0.96 &0.44 &0.60 &0.62 &0.25 &0.46 &0.05 &0.00 &0.2708$\pm$0.0135 \\ 
        & A3 &0.94 &0.76 &0.84 &0.89 &0.63 &0.90 &0.41 &0.55 &0.2976$\pm$0.0737 \\ 
        & A4 &0.93 &0.60 &0.73 &0.62 &0.58 &0.70 &0.38 &0.29 &0.7483$\pm$0.0406 \\ \hline  \hline  
        \multirow{4}{*}{Mall-1} & A1 &0.23 &0.97 &0.37 &0.99 &0.94 &0.98 &0.85 &- &2.0492$\pm$0.0460 \\ 
        & A2 &0.81 &0.18 &0.30 &0.34 &0.01 &0.19 &0.03 &- &0.2840$\pm$0.0119 \\ 
        & A3 &0.80 &0.39 &0.52 &0.70 &0.08 &0.56 &0.17 &- &0.3257$\pm$0.0754 \\ 
        & A4 &0.72 &0.34 &0.46 &0.60 &0.10 &0.52 &0.09 &- &0.7632$\pm$0.0611 \\ \hline 
        \multirow{4}{*}{Mall-2} & A1 &0.27 &0.98 &0.43 &0.99 &0.97 &0.99 &0.88 &0.83 &2.0991$\pm$0.0383 \\ 
        & A2 &0.92 &0.16 &0.27 &0.30 &0.01 &0.16 &0.02 &0.00 &0.2864$\pm$0.0139 \\ 
        & A3 &0.84 &0.43 &0.57 &0.76 &0.10 &0.60 &0.20 &0.47 &0.3290$\pm$0.0865 \\ 
        & A4 &0.77 &0.37 &0.50 &0.67 &0.08 &0.54 &0.12 &0.09 &0.7585$\pm$0.0482 \\ \hline 
        \multirow{4}{*}{Mall-3} & A1 &0.32 &0.97 &0.48 &1.00 &0.95 &0.98 &0.88 &0.53 &2.1051$\pm$0.0415 \\ 
        & A2 &0.91 &0.52 &0.66 &0.83 &0.21 &0.54 &0.04 &0.00 &0.3041$\pm$0.0253 \\ 
        & A3 &0.88 &0.68 &0.77 &0.91 &0.46 &0.82 &0.38 &0.21 &0.2849$\pm$0.0714 \\ 
        & A4 &0.95 &0.61 &0.74 &0.75 &0.47 &0.74 &0.31 &0.00 &0.7542$\pm$0.0566 \\ \hline 
        \multirow{4}{*}{Mall-4} & A1 &0.44 &0.91 &0.59 &0.89 &0.92 &0.91 &0.79 &0.65 &2.0734$\pm$0.0524 \\ 
        & A2 &0.94 &0.27 &0.42 &0.38 &0.16 &0.28 &0.08 &0.00 &0.3043$\pm$0.0206 \\ 
        & A3 &0.92 &0.61 &0.74 &0.62 &0.61 &0.67 &0.30 &0.35 &0.2903$\pm$0.0690 \\ 
        & A4 &0.90 &0.53 &0.67 &0.49 &0.58 &0.59 &0.13 &0.29 &0.7598$\pm$0.0488 \\ \hline \hline 
        \multirow{4}{*}{Pedestrian-1} & A1 &0.30 &0.97 &0.46 &0.99 &0.95 &0.98 &0.58 &- &2.0761$\pm$0.0497 \\ 
        & A2 &0.98 &0.38 &0.55 &0.66 &0.10 &0.39 &0.00 &- &0.3068$\pm$0.0119 \\ 
        & A3 &0.99 &0.76 &0.86 &0.92 &0.60 &0.81 &0.33 &- &0.2760$\pm$0.0689 \\ 
        & A4 &1.00 &0.65 &0.79 &0.59 &0.72 &0.70 &0.31 &- &0.7497$\pm$0.0423 \\ \hline 
        \multirow{4}{*}{Pedestrian-2} & A1 &0.29 &0.94 &0.44 &0.98 &0.91 &0.97 &0.70 &0.37 &2.0263$\pm$0.0409 \\ 
        & A2 &0.95 &0.36 &0.52 &0.59 &0.13 &0.39 &0.01 &0.00 &0.3125$\pm$0.0112 \\ 
        & A3 &0.86 &0.56 &0.68 &0.74 &0.38 &0.71 &0.23 &0.08 &0.2918$\pm$0.0686 \\ 
        & A4 &0.88 &0.54 &0.67 &0.61 &0.48 &0.71 &0.17 &0.23 &0.7516$\pm$0.0399 \\ \hline 
        \multirow{4}{*}{Pedestrian-3} & A1 &0.39 &0.95 &0.55 &0.97 &0.94 &0.96 &0.97 &0.33 &2.0515$\pm$0.0372 \\ 
        & A2 &0.94 &0.36 &0.52 &0.58 &0.14 &0.37 &0.00 &0.00 &0.3047$\pm$0.0161 \\ 
        & A3 &0.98 &0.87 &0.92 &0.95 &0.79 &0.91 &0.65 &0.50 &0.2779$\pm$0.0698 \\ 
        & A4 &0.99 &0.74 &0.85 &0.78 &0.70 &0.80 &0.23 &0.25 &0.7573$\pm$0.0506 \\ \hline 
        \multirow{4}{*}{Pedestrian-4} & A1 &0.38 &0.94 &0.54 &1.00 &0.89 &0.96 &0.85 &0.49 &2.0454$\pm$0.0484 \\ 
        & A2 &0.60 &0.55 &0.57 &0.77 &0.33 &0.58 &0.02 &0.00 &0.3767$\pm$0.0185 \\ 
        & A3 &0.84 &0.73 &0.78 &0.84 &0.64 &0.82 &0.43 &0.55 &0.2909$\pm$0.0743 \\ 
        & A4 &0.85 &0.49 &0.62 &0.42 &0.56 &0.57 &0.14 &0.08 &0.7528$\pm$0.0507 \\ 
        \multirow{4}{*}{Pedestrian-5} & A1 &0.74 &0.92 &0.82 &0.97 &0.88 &0.93 &0.92 &0.76 &1.9857$\pm$0.0388 \\ 
        & A2 &0.96 &0.22 &0.36 &0.41 &0.03 &0.24 &0.00 &0.00 &0.3319$\pm$0.0187 \\ 
        & A3 &0.99 &0.74 &0.84 &0.85 &0.61 &0.79 &0.42 &0.39 &0.2868$\pm$0.0877 \\ 
        & A4 &0.99 &0.76 &0.86 &0.83 &0.69 &0.83 &0.36 &0.33 &0.7582$\pm$0.0509 \\ \hline \hline 
        \multirow{4}{*}{Subway-1} & A1 &0.64 &0.95 &0.76 &0.99 &0.91 &0.99 &0.97 &0.65 &2.0417$\pm$0.0676 \\ 
        & A2 &0.98 &0.32 &0.48 &0.42 &0.21 &0.36 &0.08 &0.01 &0.2954$\pm$0.0126 \\ 
        & A3 &0.97 &0.70 &0.82 &0.92 &0.52 &0.83 &0.43 &0.46 &0.2996$\pm$0.0838 \\ 
        & A4 &0.85 &0.65 &0.74 &0.84 &0.47 &0.80 &0.25 &0.15 &0.7517$\pm$0.0463 \\ \hline 
        \multirow{4}{*}{Subway-2} & A1 &0.55 &0.97 &0.70 &1.00 &0.94 &0.97 &0.95 &0.67 &2.0307$\pm$0.0458 \\ 
        & A2 &0.99 &0.33 &0.50 &0.45 &0.22 &0.35 &0.03 &0.00 &0.2995$\pm$0.0121 \\ 
        & A3 &0.99 &0.58 &0.73 &0.86 &0.33 &0.71 &0.20 &0.45 &0.3192$\pm$0.0971 \\ 
        & A4 &0.97 &0.57 &0.72 &0.81 &0.35 &0.71 &0.13 &0.33 &0.7510$\pm$0.0319 \\ \hline 
        \multirow{4}{*}{Subway-3} & A1 &0.57 &0.94 &0.71 &0.99 &0.90 &0.97 &0.98 &0.65 &2.0106$\pm$0.0330 \\ 
        & A2 &0.94 &0.22 &0.36 &0.24 &0.20 &0.24 &0.14 &0.09 &0.3006$\pm$0.0114 \\ 
        & A3 &0.98 &0.62 &0.76 &0.90 &0.41 &0.75 &0.50 &0.64 &0.3106$\pm$0.0714 \\ 
        & A4 &0.97 &0.61 &0.75 &0.83 &0.43 &0.76 &0.41 &0.53 &0.7586$\pm$0.0461 \\ 
        \specialrule{1.2pt}{0.2pt}{1pt}
        \multirow{4}{*}{Overall} &A1 &0.48$\pm$0.17 &0.96$\pm$0.02 &0.62$\pm$0.15 &0.98$\pm$0.02 &0.93$\pm$0.03 &0.97$\pm$0.02 &0.88$\pm$0.11 &-$\pm$- &2.0427$\pm$0.0371 \\ 
         &A2 &0.92$\pm$0.09 &0.37$\pm$0.13 &0.51$\pm$0.13 &0.54$\pm$0.18 &0.19$\pm$0.12 &0.39$\pm$0.14 &0.04$\pm$0.04 &-$\pm$- &0.3004$\pm$0.0252 \\ 
         &A3 &0.93$\pm$0.06 &0.67$\pm$0.13 &0.77$\pm$0.11 &0.85$\pm$0.10 &0.49$\pm$0.19 &0.78$\pm$0.10 &0.34$\pm$0.13 &-$\pm$- &0.2935$\pm$0.0184 \\ 
         &A4 &0.92$\pm$0.08 &0.57$\pm$0.11 &0.70$\pm$0.11 &0.68$\pm$0.12 &0.47$\pm$0.18 &0.68$\pm$0.09 &0.23$\pm$0.11 &-$\pm$- &0.7545$\pm$0.0043 \\ 
        \specialrule{1.2pt}{0.2pt}{1pt}
        \end{tabular}
        }%
\end{table}
%=====================

% SYSTEM 3 - CPU
%=====================
\begin{table}[!t]
    \centering
    \footnotesize
    \setlength{\tabcolsep}{1pt}
    \caption{Localization results per video running algorithms in \textbf{System 3} with \textbf{CPU}. KEY -- Ax: algorithm x; P: precision; R: recall; F: F1-Score.}
    \label{tab:detection_results_S3}
    \resizebox{\columnwidth}{!}{
        \begin{tabular}{lc|ccc|cc|ccc|c}
        \specialrule{1.2pt}{0.2pt}{1pt}
        \multicolumn{1}{c}{\multirow{2}{*}{Video}} & \multicolumn{1}{c|}{\multirow{2}{*}{Alg.}} & \multicolumn{1}{c}{\multirow{2}{*}{P}} & \multicolumn{1}{c}{\multirow{2}{*}{R}} & \multicolumn{1}{c|}{\multirow{2}{*}{F}} & \multicolumn{2}{c|}{Recall distance} &
        \multicolumn{3}{c|}{Recall occlusion} &
        \multicolumn{1}{|c}{\multirow{2}{*}{\begin{tabular}[c]{@{}c@{}}Speed\\ {[}seconds/frame{]}\end{tabular}}} \\
         &  &  &  &  & \multicolumn{1}{c}{Close}  & \multicolumn{1}{c|}{Far} & \multicolumn{1}{c}{No}  & \multicolumn{1}{c}{Partial}  & \multicolumn{1}{c|}{Heavy} & \\
        \specialrule{1.2pt}{0.2pt}{1pt}
        \multirow{4}{*}{Airport-1} & A1 &0.50 &0.87 &0.63 &0.99 &0.76 &0.88 &0.64 &0.14 &3.1211$\pm$0.0916 \\ 
        & A2 &0.89 &0.61 &0.72 &0.77 &0.45 &0.62 &0.09 &0.00 &0.6828$\pm$0.0444 \\ 
        & A3 &0.97 &0.77 &0.86 &0.95 &0.59 &0.82 &0.28 &0.71 &2.4976$\pm$0.2327 \\ 
        & A4 &0.98 &0.60 &0.74 &0.72 &0.48 &0.65 &0.11 &0.00 &10.1951$\pm$0.3866 \\ \hline 
        \multirow{4}{*}{Airport-2} & A1 &0.67 &0.83 &0.74 &0.99 &0.68 &0.85 &0.38 &0.13 &2.7811$\pm$0.1235 \\ 
        & A2 &1.00 &0.50 &0.67 &0.71 &0.29 &0.51 &0.08 &0.00 &0.6643$\pm$0.0762 \\ 
        & A3 &0.98 &0.80 &0.88 &0.95 &0.64 &0.88 &0.15 &0.61 &2.5249$\pm$0.2743 \\ 
        & A4 &0.99 &0.65 &0.78 &0.75 &0.55 &0.72 &0.38 &0.10 &9.3575$\pm$0.2061 \\ \hline 
        \multirow{4}{*}{Airport-3} & A1 &0.76 &0.84 &0.80 &0.97 &0.72 &0.88 &0.66 &0.21 &3.1335$\pm$0.1700 \\ 
        & A2 &0.98 &0.47 &0.63 &0.58 &0.36 &0.51 &0.05 &0.00 &0.6864$\pm$0.0883 \\ 
        & A3 &0.96 &0.66 &0.78 &0.91 &0.40 &0.81 &0.33 &0.42 &2.5088$\pm$0.2729 \\ 
        & A4 &0.99 &0.46 &0.63 &0.65 &0.28 &0.59 &0.11 &0.12 &9.3513$\pm$0.2682 \\ \hline 
        \multirow{4}{*}{Airport-4} & A1 &0.59 &0.83 &0.69 &0.93 &0.73 &0.86 &0.29 &0.24 &3.1468$\pm$0.2181 \\ 
        & A2 &0.96 &0.44 &0.60 &0.62 &0.25 &0.46 &0.05 &0.00 &0.6835$\pm$0.0719 \\ 
        & A3 &0.96 &0.73 &0.83 &0.87 &0.59 &0.88 &0.36 &0.38 &2.8266$\pm$0.3600 \\ 
        & A4 &0.93 &0.60 &0.73 &0.62 &0.58 &0.70 &0.38 &0.29 &10.1273$\pm$0.2235 \\ \hline \hline 
        \multirow{4}{*}{Mall-1} & A1 &0.45 &0.39 &0.42 &0.68 &0.08 &0.41 &0.12 &- &3.1209$\pm$0.0989 \\ 
        & A2 &0.81 &0.18 &0.30 &0.34 &0.01 &0.19 &0.03 &- &0.7677$\pm$0.1023 \\ 
        & A3 &0.84 &0.34 &0.48 &0.65 &0.03 &0.50 &0.11 &- &2.9135$\pm$0.2794 \\ 
        & A4 &0.72 &0.34 &0.46 &0.60 &0.10 &0.52 &0.09 &- &10.1540$\pm$0.2828 \\ \hline 
        \multirow{4}{*}{Mall-2} & A1 &0.35 &0.36 &0.36 &0.60 &0.12 &0.37 &0.13 &0.09 &2.7740$\pm$0.1025 \\ 
        & A2 &0.92 &0.16 &0.27 &0.30 &0.01 &0.16 &0.02 &0.00 &0.7604$\pm$0.0542 \\ 
        & A3 &0.86 &0.38 &0.53 &0.72 &0.06 &0.55 &0.14 &0.38 &3.0588$\pm$0.4127 \\ 
        & A4 &0.77 &0.37 &0.50 &0.67 &0.08 &0.54 &0.12 &0.09 &10.1212$\pm$0.1426 \\ \hline 
        \multirow{4}{*}{Mall-3} & A1 &0.74 &0.61 &0.67 &0.96 &0.26 &0.62 &0.16 &0.05 &2.7840$\pm$0.1521 \\ 
        & A2 &0.91 &0.52 &0.66 &0.83 &0.21 &0.54 &0.04 &0.00 &0.8176$\pm$0.1507 \\ 
        & A3 &0.97 &0.67 &0.79 &0.90 &0.43 &0.81 &0.31 &0.19 &2.6653$\pm$0.3049 \\ 
        & A4 &0.95 &0.61 &0.74 &0.75 &0.47 &0.74 &0.31 &0.00 &10.1575$\pm$0.2829 \\ \hline 
        \multirow{4}{*}{Mall-4} & A1 &0.66 &0.43 &0.52 &0.55 &0.31 &0.44 &0.26 &0.08 &2.7724$\pm$0.0874 \\ 
        & A2 &0.94 &0.27 &0.42 &0.38 &0.16 &0.28 &0.08 &0.00 &0.8281$\pm$0.1137 \\ 
        & A3 &0.97 &0.58 &0.73 &0.59 &0.57 &0.64 &0.22 &0.34 &2.6152$\pm$0.2583 \\ 
        & A4 &0.90 &0.53 &0.67 &0.49 &0.58 &0.59 &0.13 &0.29 &9.6167$\pm$0.6254 \\ \hline \hline 
        \multirow{4}{*}{Pedestrian-1} & A1 &0.51 &0.61 &0.55 &0.93 &0.27 &0.62 &0.17 &- &3.1590$\pm$0.2639 \\ 
        & A2 &0.98 &0.38 &0.55 &0.66 &0.10 &0.39 &0.00 &- &0.8501$\pm$0.0585 \\ 
        & A3 &0.99 &0.72 &0.83 &0.89 &0.55 &0.76 &0.31 &- &2.5926$\pm$0.2751 \\ 
        & A4 &1.00 &0.65 &0.79 &0.59 &0.72 &0.70 &0.31 &- &9.4000$\pm$0.2214 \\ \hline 
        \multirow{4}{*}{Pedestrian-2} & A1 &0.42 &0.57 &0.49 &0.84 &0.30 &0.62 &0.05 &0.10 &3.1205$\pm$0.0994 \\ 
        & A2 &0.95 &0.36 &0.52 &0.59 &0.13 &0.39 &0.01 &0.00 &0.9135$\pm$0.0479 \\ 
        & A3 &0.95 &0.55 &0.70 &0.75 &0.35 &0.71 &0.21 &0.12 &2.7351$\pm$0.2915 \\ 
        & A4 &0.88 &0.54 &0.67 &0.61 &0.48 &0.71 &0.17 &0.23 &9.4902$\pm$0.2433 \\ \hline 
        \multirow{4}{*}{Pedestrian-3} & A1 &0.55 &0.64 &0.59 &0.84 &0.45 &0.66 &0.28 &0.07 &2.7755$\pm$0.0917 \\ 
        & A2 &0.94 &0.36 &0.52 &0.58 &0.14 &0.37 &0.00 &0.00 &0.8593$\pm$0.1070 \\ 
        & A3 &0.98 &0.86 &0.92 &0.93 &0.79 &0.91 &0.60 &0.50 &2.5791$\pm$0.2412 \\ 
        & A4 &0.99 &0.74 &0.85 &0.78 &0.70 &0.80 &0.23 &0.25 &9.3863$\pm$0.2083 \\ 
        \multirow{4}{*}{Pedestrian-4} & A1 &0.56 &0.75 &0.64 &0.95 &0.54 &0.77 &0.42 &0.30 &2.7990$\pm$0.2282 \\ 
        & A2 &0.60 &0.55 &0.57 &0.77 &0.33 &0.58 &0.02 &0.00 &1.1712$\pm$0.0743 \\ 
        & A3 &0.93 &0.63 &0.75 &0.68 &0.60 &0.72 &0.33 &0.20 &2.6934$\pm$0.2544 \\ 
        & A4 &0.85 &0.49 &0.62 &0.42 &0.56 &0.57 &0.14 &0.08 &9.3856$\pm$0.2142 \\ \hline 
        \multirow{4}{*}{Pedestrian-5} & A1 &0.59 &0.48 &0.53 &0.82 &0.12 &0.49 &0.34 &0.22 &3.1169$\pm$0.0680 \\ 
        & A2 &0.96 &0.22 &0.36 &0.41 &0.03 &0.24 &0.00 &0.00 &1.0555$\pm$0.1597 \\ 
        & A3 &1.00 &0.69 &0.81 &0.79 &0.58 &0.74 &0.37 &0.37 &2.6714$\pm$0.2789 \\ 
        & A4 &0.99 &0.76 &0.86 &0.83 &0.69 &0.83 &0.36 &0.33 &10.1009$\pm$0.2464 \\ \hline \hline 
        \multirow{4}{*}{Subway-1} & A1 &0.66 &0.79 &0.72 &0.95 &0.62 &0.81 &0.77 &0.53 &3.1159$\pm$0.0648 \\ 
        & A2 &0.98 &0.32 &0.48 &0.42 &0.21 &0.36 &0.08 &0.01 &0.7848$\pm$0.0499 \\ 
        & A3 &0.98 &0.71 &0.82 &0.92 &0.53 &0.83 &0.44 &0.52 &3.1649$\pm$0.5909 \\ 
        & A4 &0.85 &0.65 &0.74 &0.84 &0.47 &0.80 &0.25 &0.15 &10.0857$\pm$0.1356 \\ \hline 
        \multirow{4}{*}{Subway-2} & A1 &0.63 &0.60 &0.61 &0.87 &0.33 &0.62 &0.29 &0.22 &2.7722$\pm$0.0578 \\ 
        & A2 &0.99 &0.33 &0.50 &0.45 &0.22 &0.35 &0.03 &0.00 &0.7965$\pm$0.0458 \\ 
        & A3 &0.99 &0.59 &0.74 &0.88 &0.34 &0.72 &0.23 &0.49 &3.3488$\pm$0.4837 \\ 
        & A4 &0.97 &0.57 &0.72 &0.81 &0.35 &0.71 &0.13 &0.33 &10.1006$\pm$0.2826 \\ \hline 
        \multirow{4}{*}{Subway-3} & A1 &0.50 &0.77 &0.60 &0.89 &0.64 &0.81 &0.62 &0.38 &3.1218$\pm$0.0892 \\ 
        & A2 &0.94 &0.22 &0.36 &0.24 &0.20 &0.24 &0.14 &0.09 &0.7953$\pm$0.0445 \\ 
        & A3 &0.97 &0.63 &0.76 &0.90 &0.42 &0.75 &0.50 &0.68 &3.3771$\pm$0.5461 \\ 
        & A4 &0.97 &0.61 &0.75 &0.83 &0.43 &0.76 &0.41 &0.53 &10.1176$\pm$0.2464 \\ 
        \specialrule{1.2pt}{0.2pt}{1pt}
        \multirow{4}{*}{Overall} &A1 &0.57$\pm$0.11 &0.65$\pm$0.17 &0.60$\pm$0.11 &0.86$\pm$0.13 &0.43$\pm$0.23 &0.67$\pm$0.17 &0.35$\pm$0.21 &-$\pm$- &2.9759$\pm$0.1734 \\ 
         &A2 &0.92$\pm$0.09 &0.37$\pm$0.13 &0.51$\pm$0.13 &0.54$\pm$0.18 &0.19$\pm$0.12 &0.39$\pm$0.14 &0.04$\pm$0.04 &-$\pm$- &0.8198$\pm$0.1319 \\ 
         &A3 &0.96$\pm$0.04 &0.64$\pm$0.13 &0.76$\pm$0.11 &0.83$\pm$0.11 &0.47$\pm$0.19 &0.75$\pm$0.11 &0.30$\pm$0.13 &-$\pm$- &2.7983$\pm$0.2824 \\ 
         &A4 &0.92$\pm$0.08 &0.57$\pm$0.11 &0.70$\pm$0.11 &0.68$\pm$0.12 &0.47$\pm$0.18 &0.68$\pm$0.09 &0.23$\pm$0.11 &-$\pm$- &9.8217$\pm$0.3540 \\ 
        \specialrule{1.2pt}{0.2pt}{1pt}
        \end{tabular}
        }
\end{table}
%=====================

% SYSTEM 4 - GPU
%=====================
\begin{table}[!t]
    \centering
    \footnotesize
    \setlength{\tabcolsep}{1pt}
    \caption{Localization results per video running algorithms in \textbf{System 4} with \textbf{GPU}. KEY -- Ax: algorithm x; P: precision; R: recall; F: F1-Score.}
    \label{tab:detection_results_S4}
    \resizebox{\columnwidth}{!}{
        \begin{tabular}{lc|ccc|cc|ccc|c}
        \specialrule{1.2pt}{0.2pt}{1pt}
        \multicolumn{1}{c}{\multirow{2}{*}{Video}} & \multicolumn{1}{c|}{\multirow{2}{*}{Alg.}} & \multicolumn{1}{c}{\multirow{2}{*}{P}} & \multicolumn{1}{c}{\multirow{2}{*}{R}} & \multicolumn{1}{c|}{\multirow{2}{*}{F}} & \multicolumn{2}{c|}{Recall distance} &
        \multicolumn{3}{c|}{Recall occlusion} &
        \multicolumn{1}{|c}{\multirow{2}{*}{\begin{tabular}[c]{@{}c@{}}Speed\\ {[}seconds/frame{]}\end{tabular}}} \\
         &  &  &  &  & \multicolumn{1}{c}{Close}  & \multicolumn{1}{c|}{Far} & \multicolumn{1}{c}{No}  & \multicolumn{1}{c}{Partial}  & \multicolumn{1}{c|}{Heavy} & \\
        \specialrule{1.2pt}{0.2pt}{1pt}
        \multirow{4}{*}{Airport-1} & A1 &0.53 &0.78 &0.61 &0.53 &0.46 &0.78 &0.01 &0.00 &3.4423$\pm$0.9443 \\ 
        & A2 &0.57 &0.49 &0.51 &0.42 &0.22 &0.50 &0.00 &0.00 &1.2229$\pm$0.3766 \\ 
        & A3 &0.87 &0.72 &0.77 &0.67 &0.39 &0.77 &0.01 &0.01 &0.9566$\pm$0.3283 \\ 
        & A4 &0.75 &0.54 &0.61 &0.49 &0.32 &0.58 &0.01 &0.00 &2.9253$\pm$1.9335 \\ \hline 
        \multirow{4}{*}{Airport-2} & A1 &0.55 &0.73 &0.60 &0.51 &0.46 &0.73 &0.01 &0.01 &3.4354$\pm$1.0196 \\ 
        & A2 &0.47 &0.35 &0.38 &0.35 &0.12 &0.35 &0.00 &0.00 &1.2442$\pm$0.4019 \\ 
        & A3 &0.81 &0.73 &0.76 &0.68 &0.42 &0.77 &0.01 &0.01 &0.9788$\pm$0.3120 \\ 
        & A4 &0.78 &0.58 &0.65 &0.53 &0.35 &0.62 &0.03 &0.00 &2.8992$\pm$1.8115 \\ \hline 
        \multirow{4}{*}{Airport-3} & A1 &0.75 &0.82 &0.77 &0.55 &0.45 &0.79 &0.07 &0.04 &3.4276$\pm$0.8300 \\ 
        & A2 &0.55 &0.41 &0.45 &0.31 &0.18 &0.43 &0.00 &0.00 &1.2157$\pm$0.3349 \\ 
        & A3 &0.82 &0.67 &0.72 &0.67 &0.27 &0.74 &0.06 &0.03 &0.9712$\pm$0.2993 \\ 
        & A4 &0.70 &0.47 &0.54 &0.48 &0.17 &0.54 &0.02 &0.01 &2.8869$\pm$1.8187 \\ \hline 
        \multirow{4}{*}{Airport-4} & A1 &0.66 &0.90 &0.74 &0.64 &0.62 &0.89 &0.04 &0.02 &3.4382$\pm$0.9419 \\ 
        & A2 &0.60 &0.43 &0.48 &0.41 &0.18 &0.44 &0.00 &0.00 &1.2526$\pm$0.5385 \\ 
        & A3 &0.94 &0.78 &0.84 &0.84 &0.63 &0.91 &0.18 &0.02 &1.0241$\pm$0.4227 \\ 
        & A4 &0.91 &0.62 &0.71 &0.58 &0.59 &0.73 &0.16 &0.01 &2.9123$\pm$1.6898 \\ \hline \hline 
        \multirow{4}{*}{Mall-1} & A1 &0.24 &0.97 &0.37 &0.94 &0.90 &0.98 &0.18 &0.00 &3.4630$\pm$0.9921 \\ 
        & A2 &0.55 &0.18 &0.26 &0.31 &0.01 &0.19 &0.01 &0.00 &1.3272$\pm$0.2915 \\ 
        & A3 &0.82 &0.39 &0.52 &0.71 &0.08 &0.57 &0.15 &0.00 &1.0578$\pm$0.3567 \\ 
        & A4 &0.72 &0.35 &0.46 &0.60 &0.10 &0.53 &0.07 &0.00 &2.9760$\pm$2.2249 \\ \hline 
        \multirow{4}{*}{Mall-2} & A1 &0.28 &0.98 &0.43 &0.95 &0.92 &0.99 &0.17 &0.04 &3.4954$\pm$1.3750 \\ 
        & A2 &0.52 &0.14 &0.21 &0.25 &0.01 &0.15 &0.00 &0.00 &1.3812$\pm$0.6119 \\ 
        & A3 &0.86 &0.43 &0.56 &0.77 &0.10 &0.60 &0.15 &0.03 &1.1008$\pm$0.4643 \\ 
        & A4 &0.79 &0.37 &0.49 &0.68 &0.08 &0.54 &0.10 &0.00 &2.9914$\pm$2.2837 \\ \hline 
        \multirow{4}{*}{Mall-3} & A1 &0.32 &0.84 &0.44 &0.54 &0.56 &0.83 &0.02 &0.02 &3.4587$\pm$1.1315 \\ 
        & A2 &0.57 &0.44 &0.48 &0.44 &0.12 &0.44 &0.00 &0.00 &1.4139$\pm$0.5515 \\ 
        & A3 &0.88 &0.71 &0.76 &0.76 &0.36 &0.83 &0.04 &0.01 &0.9957$\pm$0.3764 \\ 
        & A4 &0.89 &0.62 &0.71 &0.60 &0.36 &0.74 &0.04 &0.00 &2.9337$\pm$2.0965 \\ \hline 
        \multirow{4}{*}{Mall-4} & A1 &0.43 &0.89 &0.56 &0.74 &0.70 &0.90 &0.06 &0.03 &3.4572$\pm$1.1774 \\ 
        & A2 &0.52 &0.25 &0.32 &0.24 &0.11 &0.26 &0.01 &0.00 &0.8281$\pm$0.1137 \\ 
        & A3 &0.89 &0.60 &0.70 &0.53 &0.58 &0.65 &0.05 &0.02 &1.0162$\pm$0.3507 \\ 
        & A4 &0.88 &0.52 &0.63 &0.43 &0.53 &0.57 &0.02 &0.02 &2.8868$\pm$1.5658 \\ \hline \hline 
        \multirow{4}{*}{Pedestrian-1} & A1 &0.29 &0.79 &0.40 &0.60 &0.56 &0.80 &0.02 &0.00 &3.4504$\pm$1.1230 \\ 
        & A2 &0.58 &0.33 &0.40 &0.45 &0.06 &0.33 &0.00 &0.00 &1.4107$\pm$0.3994 \\ 
        & A3 &0.90 &0.73 &0.80 &0.76 &0.50 &0.76 &0.05 &0.00 &1.0002$\pm$0.2560 \\ 
        & A4 &0.93 &0.67 &0.76 &0.46 &0.60 &0.72 &0.04 &0.00 &2.8819$\pm$1.4628 \\ \hline 
        \multirow{4}{*}{Pedestrian-2} & A1 &0.28 &0.79 &0.39 &0.65 &0.49 &0.81 &0.09 &0.01 &3.4347$\pm$0.8917 \\ 
        & A2 &0.51 &0.31 &0.37 &0.37 &0.07 &0.33 &0.00 &0.00 &1.4599$\pm$0.3652 \\ 
        & A3 &0.86 &0.60 &0.69 &0.73 &0.32 &0.75 &0.13 &0.00 &1.0152$\pm$0.2832 \\ 
        & A4 &0.87 &0.59 &0.67 &0.62 &0.42 &0.75 &0.11 &0.00 &2.8786$\pm$1.4857 \\ \hline 
        \multirow{4}{*}{Pedestrian-3} & A1 &0.36 &0.76 &0.48 &0.48 &0.45 &0.75 &0.03 &0.00 &3.4541$\pm$0.8684 \\ 
        & A2 &0.35 &0.27 &0.30 &0.28 &0.07 &0.28 &0.00 &0.00 &1.4534$\pm$0.4563 \\ 
        & A3 &0.93 &0.85 &0.88 &0.67 &0.48 &0.87 &0.05 &0.01 &0.9787$\pm$0.3153 \\ 
        & A4 &0.84 &0.70 &0.75 &0.52 &0.41 &0.74 &0.01 &0.00 &2.8852$\pm$1.7364 \\ \hline 
        \multirow{4}{*}{Pedestrian-4} & A1 &0.39 &0.88 &0.52 &0.69 &0.54 &0.88 &0.04 &0.02 &3.4375$\pm$1.0487 \\ 
        & A2 &0.54 &0.54 &0.51 &0.53 &0.22 &0.56 &0.00 &0.00 &1.1712$\pm$0.0743 \\ 
        & A3 &0.87 &0.76 &0.79 &0.72 &0.58 &0.85 &0.08 &0.03 &1.0109$\pm$0.3944 \\ 
        & A4 &0.83 &0.51 &0.61 &0.37 &0.49 &0.60 &0.03 &0.00 &2.8920$\pm$1.6072 \\ \hline 
        \multirow{4}{*}{Pedestrian-5} & A1 &0.62 &0.71 &0.64 &0.59 &0.44 &0.72 &0.13 &0.06 &3.4851$\pm$1.4734 \\ 
        & A2 &0.37 &0.17 &0.22 &0.24 &0.01 &0.18 &0.00 &0.00 &1.0555$\pm$0.1597 \\ 
        & A3 &0.99 &0.76 &0.85 &0.81 &0.44 &0.82 &0.11 &0.03 &0.9906$\pm$0.5171 \\ 
        & A4 &0.97 &0.78 &0.85 &0.80 &0.49 &0.85 &0.11 &0.02 &2.9470$\pm$1.9560 \\ \hline \hline 
        \multirow{4}{*}{Subway-1} & A1 &0.62 &0.85 &0.70 &0.69 &0.69 &0.87 &0.11 &0.25 &3.4661$\pm$1.3278 \\ 
        & A2 &0.73 &0.31 &0.41 &0.32 &0.18 &0.34 &0.01 &0.01 &1.3494$\pm$0.4645 \\ 
        & A3 &0.93 &0.71 &0.79 &0.70 &0.51 &0.82 &0.11 &0.17 &1.0066$\pm$0.4529 \\ 
        & A4 &0.81 &0.64 &0.70 &0.63 &0.46 &0.76 &0.06 &0.06 &2.9775$\pm$2.3249 \\ \hline 
        \multirow{4}{*}{Subway-2} & A1 &0.59 &0.97 &0.70 &0.81 &0.81 &0.97 &0.16 &0.06 &3.4841$\pm$1.4000 \\ 
        & A2 &0.81 &0.32 &0.44 &0.37 &0.18 &0.34 &0.00 &0.00 &1.4148$\pm$0.6504 \\ 
        & A3 &0.98 &0.60 &0.74 &0.75 &0.33 &0.73 &0.11 &0.04 &1.0673$\pm$0.5259 \\ 
        & A4 &0.96 &0.58 &0.72 &0.69 &0.34 &0.72 &0.06 &0.03 &3.0648$\pm$2.8867 \\ \hline 
        \multirow{4}{*}{Subway-3} & A1 &0.57 &0.89 &0.67 &0.80 &0.69 &0.90 &0.11 &0.18 &3.4864$\pm$1.1692 \\ 
        & A2 &0.53 &0.20 &0.28 &0.17 &0.14 &0.21 &0.02 &0.02 &21.9446$\pm$506.1390 \\ 
        & A3 &0.94 &0.63 &0.74 &0.87 &0.38 &0.75 &0.23 &0.17 &1.1062$\pm$0.3517 \\ 
        & A4 &0.93 &0.61 &0.72 &0.80 &0.42 &0.75 &0.19 &0.14 &2.8948$\pm$1.6968 \\ 
        \specialrule{1.2pt}{0.2pt}{1pt}
        \multirow{4}{*}{Overall} &A1 &0.47$\pm$0.16 &0.85$\pm$0.08 &0.56$\pm$0.13 &0.67$\pm$0.14 &0.67$\pm$0.14 &0.85$\pm$0.08 &0.08$\pm$0.06 &0.05$\pm$0.07 &3.4573$\pm$0.0206 \\ 
        &A2 &0.55$\pm$0.11 &0.32$\pm$0.11 &0.38$\pm$0.10 &0.34$\pm$0.09 &0.34$\pm$0.09 &0.33$\pm$0.12 &0.00$\pm$0.00 &0.00$\pm$0.00 &2.5716$\pm$5.0047 \\ 
        &A3 &0.89$\pm$0.05 &0.67$\pm$0.12 &0.74$\pm$0.09 &0.73$\pm$0.08 &0.73$\pm$0.08 &0.76$\pm$0.09 &0.10$\pm$0.06 &0.04$\pm$0.05 &1.0173$\pm$0.0429 \\ 
        &A4 &0.85$\pm$0.08 &0.57$\pm$0.11 &0.66$\pm$0.10 &0.58$\pm$0.12 &0.58$\pm$0.12 &0.67$\pm$0.10 &0.07$\pm$0.05 &0.02$\pm$0.03 &2.9271$\pm$0.0507 \\ 
        \specialrule{1.2pt}{0.2pt}{1pt}
        \end{tabular}
        }%
\end{table}
%=====================

\section*{Appendix B: People counting results per video}
\label{appendix:counting_results}
People counting results per video in
System 1-GPU in Table~\ref{tab:count_S1gpu},
System 1-CPU in Table~\ref{tab:count_S1cpu},
System 2-GPU in Table~\ref{tab:count_S2gpu},
System 2-CPU in Table~\ref{tab:count_S2cpu},
System 3 in Table~\ref{tab:count_S3}, and 
System 4 in Table~\ref{tab:count_S4}.

% SYSTEM 1 - GPU
%=====================
\begin{table}[!t]
    \centering
    \small
    \setlength{\tabcolsep}{1pt}
    \caption{People counting results per video running algorithms in \textbf{System 1} with \textbf{GPU}. KEY -- Ax: algorithm x; MOE: mean opportunity error of people with OTS; COE: cumulative opportunity error of people with OTS; MPE: mean opportunity error all people.
    \label{tab:count_S1gpu}
    }
    \resizebox{\columnwidth}{!}{
    \begin{tabular}{ll|rrr|rr|c}
    \specialrule{1.2pt}{0.2pt}{1pt}
    \multicolumn{1}{c}{\multirow{2}{*}{Video}} & \multicolumn{1}{c|}{\multirow{2}{*}{Alg.}} & \multicolumn{1}{c}{\multirow{2}{*}{MOE}} & \multicolumn{1}{c}{\multirow{2}{*}{COE}} & \multicolumn{1}{c|}{\multirow{2}{*}{MPE}} & \multicolumn{2}{c|}{MOE} & \multicolumn{1}{|c}{\multirow{2}{*}{\begin{tabular}[c]{@{}c@{}}Speed\\ {[}seconds/frame{]}\end{tabular}}} \\
     &  &  &  &  & \multicolumn{1}{c}{Close}  & \multicolumn{1}{c|}{Far} & \\
    \specialrule{1.2pt}{0.2pt}{1pt}
    \multirow{4}{*}{Airport-1} & A1 &0.55 &503.52 &0.89 &0.19 &0.47 &0.0414$\pm$0.0129 \\ 
    & A2 &0.58 &310.28 &1.37 &0.27 &0.43 &0.0277$\pm$0.0030 \\ 
    & A3 &0.64 &0.79 &0.47 &0.15 &0.56 &0.0629$\pm$0.0097 \\ 
    & A4 &0.72 &1.66 &0.33 &0.36 &0.64 &0.0798$\pm$0.0006 \\  \hline 
    \multirow{4}{*}{Airport-2} & A1 &0.92 &783.55 &0.67 &0.15 &0.76 &0.1728$\pm$0.0195 \\ 
    & A2 &0.79 &248.07 &1.63 &0.25 &0.51 &0.0274$\pm$0.0049 \\ 
    & A3 &0.66 &0.34 &0.44 &0.16 &0.52 &0.0823$\pm$0.0129 \\ 
    & A4 &0.74 &1.07 &0.25 &0.50 &0.69 &0.0806$\pm$0.0008 \\ \hline 
    \multirow{4}{*}{Airport-3} & A1 &0.71 &377.20 &0.96 &0.20 &0.38 &0.0408$\pm$0.0099 \\ 
    & A2 &1.16 &194.36 &1.57 &0.39 &0.51 &0.0279$\pm$0.0037 \\ 
    & A3 &0.71 &0.36 &0.68 &0.25 &0.81 &0.0663$\pm$0.0123 \\ 
    & A4 &0.70 &1.73 &0.67 &0.48 &1.06 &0.0795$\pm$0.0006 \\ \hline 
    \multirow{4}{*}{Airport-4} & A1 &0.85 &354.39 &2.58 &0.23 &0.62 &0.0416$\pm$0.0129 \\ 
    & A2 &1.33 &145.71 &3.84 &0.40 &0.71 &0.0282$\pm$0.0057 \\ 
    & A3 &1.68 &0.66 &1.07 &0.30 &1.08 &0.0667$\pm$0.0131 \\ 
    & A4 &1.96 &2.25 &0.81 &0.61 &1.25 &0.0803$\pm$0.0005 \\ \hline \hline 
    \multirow{4}{*}{Mall-1} & A1 &4.19 &224.14 &10.09 &1.35 &2.68 &0.0413$\pm$0.0134 \\
    & A2 &5.86 &92.34 &11.84 &1.78 &2.62 &0.0393$\pm$0.0036 \\ 
    & A3 &2.23 &0.62 &7.42 &1.57 &6.18 &0.0756$\pm$0.0166 \\ 
    & A4 &1.98 &4.89 &5.57 &1.40 &6.03 &0.0810$\pm$0.0005 \\ \hline 
    \multirow{4}{*}{Mall-2} & A1 &27.25 &2278.65 &21.71 &8.64 &21.02 &0.1735$\pm$0.0235 \\ 
    & A2 &7.78 &67.48 &13.31 &2.20 &3.18 &0.0391$\pm$0.0047 \\ 
    & A3 &3.09 &0.63 &7.64 &1.46 &6.98 &0.0938$\pm$0.0152 \\ 
    & A4 &2.76 &3.92 &6.02 &1.73 &7.08 &0.0823$\pm$0.0008 \\ \hline 
    \multirow{4}{*}{Mall-3} & A1 &7.76 &3278.23 &6.20 &2.45 &5.58 &0.1739$\pm$0.0192 \\
    & A2 &1.15 &378.17 &2.65 &0.24 &0.78 &0.0446$\pm$0.0128 \\ 
    & A3 &1.47 &2.97 &1.26 &0.38 &1.23 &0.0829$\pm$0.0127 \\ 
    & A4 &1.27 &6.00 &0.96 &0.57 &1.30 &0.0810$\pm$0.0006 \\ \hline 
    \multirow{4}{*}{Mall-4} & A1 &8.13 &2499.30 &7.13 &2.37 &6.13 &0.1728$\pm$0.0183 \\
    & A2 &2.44 &190.66 &3.43 &0.91 &1.22 &0.0465$\pm$0.0101 \\ 
    & A3 &1.35 &1.72 &1.39 &0.76 &1.01 &0.0831$\pm$0.0125 \\ 
    & A4 &1.46 &5.12 &1.15 &0.80 &1.00 &0.0812$\pm$0.0006 \\ \hline \hline 
    \multirow{4}{*}{Pedestrian-1} & A1 &1.19 &957.29 &2.40 &0.46 &0.86 &0.0419$\pm$0.0122 \\ 
    & A2 &1.67 &474.53 &3.06 &0.36 &0.86 &0.0505$\pm$0.0047 \\ 
    & A3 &1.01 &1.12 &0.98 &0.37 &1.06 &0.0635$\pm$0.0095 \\ 
    & A4 &0.84 &4.47 &1.02 &0.60 &1.08 &0.0797$\pm$0.0005 \\ \hline 
    \multirow{4}{*}{Pedestrian-2} & A1 &1.56 &568.58 &3.25 &0.66 &1.01 &0.0421$\pm$0.0108 \\ 
    & A2 &1.64 &255.97 &4.28 &0.54 &0.95 &0.0571$\pm$0.0032 \\ 
    & A3 &1.77 &2.10 &2.05 &0.69 &1.55 &0.0647$\pm$0.0103 \\ 
    & A4 &2.00 &8.38 &1.72 &0.72 &1.56 &0.0801$\pm$0.0004 \\ \hline 
    \multirow{4}{*}{Pedestrian-3} & A1 &5.60 &2791.24 &4.57 &1.79 &3.63 &0.1736$\pm$0.0187 \\ 
    & A2 &0.66 &248.40 &1.64 &0.34 &0.61 &0.0522$\pm$0.0067 \\ 
    & A3 &0.92 &0.76 &0.30 &0.18 &0.40 &0.0844$\pm$0.0130 \\ 
    & A4 &0.97 &2.60 &0.21 &0.45 &0.57 &0.0808$\pm$0.0007 \\ \hline 
    \multirow{4}{*}{Pedestrian-4} & A1 &3.74 &2073.16 &2.58 &0.58 &3.82 &0.1755$\pm$0.0203 \\ 
    & A2 &1.14 &628.08 &2.24 &0.62 &0.72 &0.0837$\pm$0.0059 \\ 
    & A3 &1.19 &2.00 &1.08 &0.59 &0.88 &0.0828$\pm$0.0123 \\ 
    & A4 &1.09 &3.84 &1.16 &0.90 &0.85 &0.0810$\pm$0.0006 \\ \hline 
    \multirow{4}{*}{Pedestrian-5} & A1 &1.90 &685.45 &3.22 &0.49 &1.26 &0.0401$\pm$0.0162 \\ 
    & A2 &2.09 &435.27 &3.70 &0.75 &1.20 &0.0699$\pm$0.0076 \\ 
    & A3 &1.74 &2.36 &1.32 &0.39 &1.03 &0.0646$\pm$0.0101 \\ 
    & A4 &1.70 &5.00 &0.87 &0.52 &1.05 &0.0801$\pm$0.0005 \\ \hline \hline 
    \multirow{4}{*}{Subway-1} & A1 &1.60 &1404.76 &2.29 &0.47 &0.97 &0.0414$\pm$0.0160 \\ 
    & A2 &4.09 &496.18 &4.90 &1.37 &1.69 &0.0416$\pm$0.0045 \\ 
    & A3 &1.80 &1.53 &2.27 &0.67 &2.06 &0.0735$\pm$0.0174 \\ 
    & A4 &1.23 &7.53 &1.24 &1.01 &1.83 &0.0804$\pm$0.0006 \\ \hline 
    \multirow{4}{*}{Subway-2} & A1 &2.56 &1738.14 &2.11 &2.23 &3.24 &0.1753$\pm$0.0278 \\ 
    & A2 &6.54 &297.75 &8.08 &1.48 &2.06 &0.0428$\pm$0.0034 \\ 
    & A3 &3.15 &0.93 &4.49 &1.21 &3.61 &0.0920$\pm$0.0150 \\ 
    & A4 &2.34 &3.54 &3.55 &1.21 &3.54 &0.0816$\pm$0.0007 \\ \hline 
    \multirow{4}{*}{Subway-3} & A1 &3.11 &1376.45 &4.42 &0.57 &0.99 &0.0459$\pm$0.0128 \\ 
    & A2 &6.07 &295.72 &7.42 &1.32 &1.37 &0.0435$\pm$0.0049 \\ 
    & A3 &2.40 &3.24 &3.62 &0.99 &2.70 &0.0751$\pm$0.0170 \\ 
    & A4 &1.83 &10.69 &2.93 &0.79 &2.56 &0.0806$\pm$0.0007 \\ 
     \specialrule{1.2pt}{0.2pt}{1pt}
    \multirow{4}{*}{Overall} &A1 &4.48$\pm$6.32 &1368.38$\pm$938.73 &4.69$\pm$5.02 &1.43$\pm$2.02 &3.34$\pm$4.90 &0.0996$\pm$0.0655 \\ 
    &A2 &2.81$\pm$2.34 &297.44$\pm$148.41 &4.69$\pm$3.54 &0.83$\pm$0.60 &1.21$\pm$0.78 &0.0451$\pm$0.0150 \\ 
    &A3 &1.61$\pm$0.77 &1.38$\pm$0.89 &2.28$\pm$2.27 &0.63$\pm$0.44 &1.98$\pm$1.93 &0.0759$\pm$0.0100 \\ 
    &A4 &1.48$\pm$0.61 &4.54$\pm$2.54 &1.78$\pm$1.75 &0.79$\pm$0.37 &2.01$\pm$1.88 &0.0806$\pm$0.0007 \\
    \specialrule{1.2pt}{0.2pt}{1pt}
    \end{tabular}
    }%
\end{table}
%=====================

% SYSTEM 1 - CPU
%=====================
\begin{table}[!t]
    \centering
    \small
    \setlength{\tabcolsep}{1pt}
    \caption{People counting results per video running algorithms in \textbf{System 1} with \textbf{CPU}. KEY -- Ax: algorithm x; MOE: mean opportunity error of people with OTS; COE: cumulative opportunity error of people with OTS; MPE: mean opportunity error all people.}
    \label{tab:count_S1cpu}
    \resizebox{\columnwidth}{!}{
    \begin{tabular}{ll|rrr|rr|c}
        \specialrule{1.2pt}{0.2pt}{1pt}
         \multicolumn{1}{c}{\multirow{2}{*}{Video}} & \multicolumn{1}{c|}{\multirow{2}{*}{Alg.}} & \multicolumn{1}{c}{\multirow{2}{*}{MOE}} & \multicolumn{1}{c}{\multirow{2}{*}{COE}} & \multicolumn{1}{c|}{\multirow{2}{*}{MPE}} & \multicolumn{2}{c|}{MOE} & \multicolumn{1}{|c}{\multirow{2}{*}{\begin{tabular}[c]{@{}c@{}}Speed\\ {[}seconds/frame{]}\end{tabular}}} \\
         &  &  &  &  & \multicolumn{1}{c}{Close}  & \multicolumn{1}{c|}{Far} & \\
        \specialrule{1.2pt}{0.2pt}{1pt}
        \multirow{4}{*}{Airport-1} & A1 &1.17 &811.97 &0.87 &0.74 &0.73 &0.3925$\pm$0.1227 \\ 
        & A2 &0.59 &306.93 &1.38 &0.27 &0.42 &0.1663$\pm$0.0160 \\ 
        & A3 &0.63 &0.62 &0.49 &0.14 &0.56 &0.3878$\pm$0.0831 \\ 
        & A4 &0.72 &1.66 &0.33 &0.36 &0.64 &1.1629$\pm$0.0656 \\ \hline 
        \multirow{4}{*}{Airport-2} & A1 &0.72 &641.83 &0.98 &0.16 &0.55 &0.3637$\pm$0.0636 \\ 
        & A2 &0.79 &246.97 &1.64 &0.25 &0.51 &0.1738$\pm$0.0218 \\ 
        & A3 &0.63 &0.31 &0.46 &0.15 &0.53 &0.3367$\pm$0.0739 \\ 
        & A4 &0.74 &1.07 &0.25 &0.50 &0.69 &1.9775$\pm$0.2558 \\ \hline 
        \multirow{4}{*}{Airport-3} & A1 &0.78 &465.93 &0.89 &0.25 &0.48 &0.3457$\pm$0.0636 \\ 
        & A2 &1.16 &194.14 &1.57 &0.39 &0.51 &0.1657$\pm$0.0208 \\ 
        & A3 &0.74 &0.14 &0.73 &0.21 &0.82 &0.3981$\pm$0.0905 \\ 
        & A4 &0.70 &1.73 &0.67 &0.48 &1.06 &1.1860$\pm$0.0436 \\ \hline 
        \multirow{4}{*}{Airport-4} & A1 &1.42 &519.66 &1.82 &0.41 &1.19 &0.3759$\pm$0.0717 \\ 
        & A2 &1.34 &145.11 &3.84 &0.40 &0.72 &0.1655$\pm$0.0191 \\ 
        & A3 &1.56 &0.52 &1.20 &0.29 &1.19 &0.4222$\pm$0.1003 \\ 
        & A4 &1.96 &2.25 &0.81 &0.61 &1.25 &1.1253$\pm$0.0383 \\ \hline \hline 
        \multirow{4}{*}{Mall-1} & A1 &2.72 &482.31 &6.85 &3.80 &2.68 &0.3488$\pm$0.0621 \\ 
        & A2 &5.88 &91.43 &11.85 &1.79 &2.62 &0.1830$\pm$0.0168 \\ 
        & A3 &2.63 &0.52 &8.29 &1.93 &6.33 &0.4651$\pm$0.1008 \\ 
        & A4 &1.98 &4.89 &5.57 &1.40 &6.03 &1.1585$\pm$0.1737 \\ \hline 
        \multirow{4}{*}{Mall-2} & A1 &3.54 &579.91 &5.75 &6.02 &3.23 &0.3499$\pm$0.0618 \\ 
        & A2 &7.78 &67.30 &13.32 &2.20 &3.18 &0.2113$\pm$0.0169 \\ 
        & A3 &3.56 &0.30 &8.54 &1.72 &7.08 &0.4092$\pm$0.0982 \\ 
        & A4 &2.76 &3.92 &6.02 &1.73 &7.08 &2.0015$\pm$0.2615 \\ \hline 
        \multirow{4}{*}{Mall-3} & A1 &1.50 &937.60 &1.74 &0.64 &1.06 &0.3507$\pm$0.0621 \\ 
        & A2 &1.12 &386.03 &2.62 &0.26 &0.77 &0.2292$\pm$0.0341 \\ 
        & A3 &1.02 &1.93 &1.27 &0.40 &1.37 &0.3465$\pm$0.0720 \\ 
        & A4 &1.27 &6.03 &0.96 &0.57 &1.30 &1.9413$\pm$0.2814 \\ \hline 
        \multirow{4}{*}{Mall-4} & A1 &1.44 &607.06 &1.91 &0.75 &1.19 &0.3500$\pm$0.0622 \\ 
        & A2 &2.32 &217.12 &3.31 &0.91 &1.16 &0.2354$\pm$0.0281 \\ 
        & A3 &1.29 &1.14 &1.69 &0.78 &1.08 &0.3379$\pm$0.0693 \\ 
        & A4 &1.46 &5.12 &1.15 &0.80 &1.00 &1.9979$\pm$0.2431 \\ \hline \hline 
        \multirow{4}{*}{Pedestrian-1} & A1 &1.72 &2220.94 &1.71 &1.52 &1.00 &0.3639$\pm$0.0640 \\ 
        & A2 &1.68 &464.18 &3.08 &0.36 &0.86 &0.2038$\pm$0.0194 \\ 
        & A3 &0.96 &1.06 &1.18 &0.44 &1.17 &0.4010$\pm$0.0939 \\ 
        & A4 &0.84 &4.47 &1.02 &0.60 &1.08 &1.1893$\pm$0.0464 \\ \hline 
        \multirow{4}{*}{Pedestrian-2} & A1 &2.67 &1170.47 &2.67 &1.39 &1.69 &0.3584$\pm$0.0642 \\ 
        & A2 &1.65 &253.65 &4.29 &0.54 &0.95 &0.2135$\pm$0.0177 \\ 
        & A3 &1.61 &1.65 &2.35 &0.69 &1.77 &0.4284$\pm$0.0980 \\ 
        & A4 &2.00 &8.38 &1.72 &0.72 &1.56 &1.1892$\pm$0.0455 \\ \hline 
        \multirow{4}{*}{Pedestrian-3} & A1 &2.98 &1664.56 &2.27 &0.60 &2.37 &0.3518$\pm$0.0622 \\ 
        & A2 &0.66 &247.76 &1.64 &0.34 &0.61 &0.2386$\pm$0.0158 \\ 
        & A3 &0.92 &0.72 &0.29 &0.17 &0.39 &0.3512$\pm$0.0661 \\ 
        & A4 &0.97 &2.60 &0.21 &0.45 &0.57 &1.9764$\pm$0.2614 \\ \hline 
        \multirow{4}{*}{Pedestrian-4} & A1 &1.73 &1214.40 &1.73 &0.53 &1.62 &0.3464$\pm$0.0623 \\ 
        & A2 &1.15 &616.84 &2.27 &0.62 &0.72 &0.3219$\pm$0.0184 \\ 
        & A3 &1.05 &1.16 &1.40 &0.74 &0.91 &0.3526$\pm$0.0695 \\ 
        & A4 &1.09 &3.84 &1.16 &0.90 &0.85 &1.9013$\pm$0.2761 \\ \hline 
        \multirow{4}{*}{Pedestrian-5} & A1 &2.54 &1874.91 &2.17 &1.08 &1.70 &0.4089$\pm$0.0741 \\ 
        & A2 &2.10 &430.45 &3.71 &0.75 &1.20 &0.2371$\pm$0.0231 \\ 
        & A3 &1.94 &1.82 &1.59 &0.47 &1.17 &0.3482$\pm$0.0709 \\ 
        & A4 &1.70 &5.00 &0.87 &0.52 &1.05 &1.1471$\pm$0.0446 \\ \hline \hline 
        \multirow{4}{*}{Subway-1} & A1 &1.54 &2007.47 &1.66 &0.92 &1.30 &0.3444$\pm$0.0625 \\ 
        & A2 &4.09 &495.53 &4.90 &1.37 &1.69 &0.1887$\pm$0.0144 \\ 
        & A3 &1.82 &1.71 &2.30 &0.65 &1.99 &0.4940$\pm$0.1369 \\ 
        & A4 &1.23 &7.53 &1.24 &1.01 &1.83 &1.1886$\pm$0.0703 \\ \hline 
        \multirow{4}{*}{Subway-2} & A1 &2.83 &951.25 &4.15 &2.13 &1.77 &0.3437$\pm$0.0626 \\ 
        & A2 &6.56 &294.93 &8.10 &1.48 &2.08 &0.2219$\pm$0.0112 \\ 
        & A3 &3.12 &0.75 &4.47 &1.14 &3.62 &0.4523$\pm$0.1068 \\ 
        & A4 &2.34 &3.54 &3.55 &1.21 &3.54 &1.9831$\pm$0.2577 \\ \hline 
        \multirow{4}{*}{Subway-3} & A1 &2.07 &2110.97 &2.84 &0.95 &1.98 &0.4373$\pm$0.0795 \\ 
        & A2 &6.07 &295.45 &7.42 &1.32 &1.37 &0.1914$\pm$0.0176 \\ 
        & A3 &2.41 &2.76 &3.64 &0.97 &2.71 &0.4892$\pm$0.1144 \\ 
        & A4 &1.83 &10.69 &2.93 &0.79 &2.56 &1.1456$\pm$0.0356 \\ 
        \specialrule{1.2pt}{0.2pt}{1pt}
        \multirow{4}{*}{Overall} &A1 &1.96$\pm$0.80 &1141.33$\pm$611.72 &2.50$\pm$1.65 &1.37$\pm$1.48 &1.53$\pm$0.74 &0.3645$\pm$0.0259 \\ 
        &A2 &2.81$\pm$2.34 &297.11$\pm$145.21 &4.68$\pm$3.54 &0.83$\pm$0.60 &1.21$\pm$0.78 &0.2092$\pm$0.0387 \\ 
        &A3 &1.62$\pm$0.88 &1.07$\pm$0.71 &2.49$\pm$2.49 &0.68$\pm$0.52 &2.04$\pm$1.94 &0.4013$\pm$0.0520 \\ 
        &A4 &1.48$\pm$0.61 &4.54$\pm$2.54 &1.78$\pm$1.75 &0.79$\pm$0.37 &2.01$\pm$1.88 &1.5170$\pm$0.3991 \\ 
        \specialrule{1.2pt}{0.2pt}{1pt}
        \end{tabular}
        }%
\end{table}
%=====================

% SYSTEM 2 - GPU
%=====================
\begin{table}[!t]
    \centering
    \footnotesize
    \setlength{\tabcolsep}{1pt}
    \caption{People counting results per video running algorithms in \textbf{System 2} with \textbf{GPU}. KEY -- Ax: algorithm x; MOE: mean opportunity error of people with OTS; COE: cumulative opportunity error of people with OTS; MPE: mean opportunity error all people.
    \label{tab:count_S2gpu}
    }
    \resizebox{\columnwidth}{!}{
    \begin{tabular}{ll|rrr|rr|c}
        \specialrule{1.2pt}{0.2pt}{1pt}
        \multicolumn{1}{c}{\multirow{2}{*}{Video}} & \multicolumn{1}{c|}{\multirow{2}{*}{Alg.}} & \multicolumn{1}{c}{\multirow{2}{*}{MOE}} & \multicolumn{1}{c}{\multirow{2}{*}{COE}} & \multicolumn{1}{c|}{\multirow{2}{*}{MPE}} & \multicolumn{2}{c|}{MOE} & \multicolumn{1}{|c}{\multirow{2}{*}{\begin{tabular}[c]{@{}c@{}}Speed\\ {[}seconds/frame{]}\end{tabular}}} \\
         &  &  &  &  & \multicolumn{1}{c}{Close}  & \multicolumn{1}{c|}{Far} & \\
        \specialrule{1.2pt}{0.2pt}{1pt}
        \multirow{4}{*}{Airport-1} & A1 &1.05 &794.52 &0.73 &0.30 &0.86 &0.1668$\pm$0.0134 \\ 
        & A2 &0.58 &310.28 &1.37 &0.27 &0.43 &0.0493$\pm$0.0025 \\ 
        & A3 &0.64 &0.79 &0.47 &0.15 &0.56 &0.0625$\pm$0.0134 \\ 
        & A4 &0.72 &1.66 &0.33 &0.36 &0.64 &0.0817$\pm$0.0009 \\ \hline 
        \multirow{4}{*}{Airport-2} & A1 &0.92 &783.55 &0.67 &0.15 &0.76 &0.1669$\pm$0.0130 \\ 
        & A2 &0.79 &248.07 &1.63 &0.25 &0.51 &0.0501$\pm$0.0048 \\ 
        & A3 &0.66 &0.34 &0.44 &0.16 &0.52 &0.0602$\pm$0.0124 \\ 
        & A4 &0.74 &1.07 &0.25 &0.50 &0.69 &0.0817$\pm$0.0010 \\ \hline 
        \multirow{4}{*}{Airport-3} & A1 &0.61 &479.05 &0.72 &0.15 &0.33 &0.1668$\pm$0.0123 \\ 
        & A2 &1.16 &194.36 &1.57 &0.39 &0.51 &0.0492$\pm$0.0034 \\ 
        & A3 &0.71 &0.36 &0.68 &0.25 &0.81 &0.0627$\pm$0.0131 \\ 
        & A4 &0.70 &1.73 &0.67 &0.48 &1.06 &0.0816$\pm$0.0009 \\ 
        \multirow{4}{*}{Airport-4} & A1 &2.33 &730.05 &1.23 &0.39 &2.17 &0.1667$\pm$0.0134 \\ 
        & A2 &1.33 &145.71 &3.84 &0.40 &0.71 &0.0505$\pm$0.0057 \\ 
        & A3 &1.68 &0.66 &1.07 &0.30 &1.08 &0.0590$\pm$0.0065 \\ 
        & A4 &1.96 &2.25 &0.81 &0.61 &1.25 &0.0822$\pm$0.0008 \\ \hline \hline 
        \multirow{4}{*}{Mall-1} & A1 &25.95 &2483.86 &19.97 &7.30 &20.26 &0.1676$\pm$0.0142 \\ 
        & A2 &5.86 &92.34 &11.84 &1.78 &2.62 &0.0601$\pm$0.0034 \\ 
        & A3 &2.23 &0.62 &7.42 &1.57 &6.18 &0.0631$\pm$0.0070 \\ 
        & A4 &1.98 &4.89 &5.57 &1.40 &6.03 &0.0829$\pm$0.0008 \\ \hline 
        \multirow{4}{*}{Mall-2} & A1 &27.25 &2278.65 &21.71 &8.64 &21.02 &0.1676$\pm$0.0159 \\ 
        & A2 &7.78 &67.48 &13.31 &2.20 &3.18 &0.0612$\pm$0.0045 \\ 
        & A3 &3.09 &0.63 &7.64 &1.46 &6.98 &0.0654$\pm$0.0081 \\ 
        & A4 &2.76 &3.92 &6.02 &1.73 &7.08 &0.0831$\pm$0.0009 \\ \hline 
        \multirow{4}{*}{Mall-3} & A1 &7.76 &3278.23 &6.20 &2.45 &5.58 &0.1670$\pm$0.0130 \\ 
        & A2 &1.15 &378.17 &2.65 &0.24 &0.78 &0.0678$\pm$0.0127 \\ 
        & A3 &1.47 &2.97 &1.26 &0.38 &1.23 &0.0584$\pm$0.0074 \\ \hline 
        & A4 &1.27 &6.00 &0.96 &0.57 &1.30 &0.0819$\pm$0.0009 \\ 
        \multirow{4}{*}{Mall-4} & A1 &8.13 &2499.30 &7.13 &2.37 &6.13 &0.1672$\pm$0.0124 \\ 
        & A2 &2.44 &190.66 &3.43 &0.91 &1.22 &0.0695$\pm$0.0099 \\ 
        & A3 &1.35 &1.72 &1.39 &0.76 &1.01 &0.0591$\pm$0.0077 \\ 
        & A4 &1.46 &5.12 &1.15 &0.80 &1.00 &0.0822$\pm$0.0008 \\ \hline \hline 
        \multirow{4}{*}{Pedestrian-1} & A1 &8.84 &6844.65 &7.43 &1.11 &8.24 &0.1671$\pm$0.0126 \\ 
        & A2 &1.67 &474.53 &3.06 &0.36 &0.86 &0.0710$\pm$0.0043 \\ 
        & A3 &1.01 &1.12 &0.98 &0.37 &1.06 &0.0574$\pm$0.0073 \\ 
        & A4 &0.84 &4.47 &1.02 &0.60 &1.08 &0.0820$\pm$0.0009 \\ \hline 
        \multirow{4}{*}{Pedestrian-2} & A1 &9.97 &3511.00 &7.34 &1.55 &8.73 &0.1669$\pm$0.0122 \\ 
        & A2 &1.64 &255.97 &4.28 &0.54 &0.95 &0.0774$\pm$0.0030 \\ 
        & A3 &1.77 &2.10 &2.05 &0.69 &1.55 &0.0592$\pm$0.0061 \\ 
        & A4 &2.00 &8.38 &1.72 &0.72 &1.56 &0.0823$\pm$0.0008 \\ \hline 
        \multirow{4}{*}{Pedestrian-3} & A1 &5.60 &2791.24 &4.57 &1.79 &3.63 &0.1687$\pm$0.0128 \\ 
        & A2 &0.66 &248.40 &1.64 &0.34 &0.61 &0.0741$\pm$0.0062 \\ 
        & A3 &0.92 &0.76 &0.30 &0.18 &0.40 &0.0635$\pm$0.0132 \\ 
        & A4 &0.97 &2.60 &0.21 &0.45 &0.57 &0.0817$\pm$0.0009 \\ \hline 
        \multirow{4}{*}{Pedestrian-4} & A1 &3.74 &2073.16 &2.58 &0.58 &3.82 &0.1685$\pm$0.0144 \\ 
        & A2 &1.14 &628.08 &2.24 &0.62 &0.72 &0.1035$\pm$0.0058 \\ 
        & A3 &1.19 &2.00 &1.08 &0.59 &0.88 &0.0594$\pm$0.0071 \\ 
        & A4 &1.09 &3.84 &1.16 &0.90 &0.85 &0.0819$\pm$0.0008 \\ \hline
        \multirow{4}{*}{Pedestrian-5} & A1 &3.83 &3198.18 &2.44 &1.02 &3.10 &0.1667$\pm$0.0176 \\ 
        & A2 &2.09 &435.27 &3.70 &0.75 &1.20 &0.0891$\pm$0.0074 \\ 
        & A3 &1.74 &2.36 &1.32 &0.39 &1.03 &0.0575$\pm$0.0067 \\ 
        & A4 &1.70 &5.00 &0.87 &0.52 &1.05 &0.0821$\pm$0.0008 \\ \hline \hline 
        \multirow{4}{*}{Subway-1} & A1 &2.15 &2511.53 &1.72 &0.64 &2.36 &0.1791$\pm$0.0171 \\ 
        & A2 &4.09 &496.18 &4.90 &1.37 &1.69 &0.0619$\pm$0.0042 \\ 
        & A3 &1.80 &1.53 &2.27 &0.67 &2.06 &0.0623$\pm$0.0084 \\ 
        & A4 &1.23 &7.53 &1.24 &1.01 &1.83 &0.0823$\pm$0.0008 \\ \hline 
        \multirow{4}{*}{Subway-2} & A1 &2.56 &1738.14 &2.11 &2.23 &3.24 &0.1690$\pm$0.0192 \\ 
        & A2 &6.54 &297.75 &8.08 &1.48 &2.06 &0.0645$\pm$0.0034 \\ 
        & A3 &3.15 &0.93 &4.49 &1.21 &3.61 &0.0629$\pm$0.0059 \\ 
        & A4 &2.34 &3.54 &3.55 &1.21 &3.54 &0.0826$\pm$0.0008 \\ \hline 
        \multirow{4}{*}{Subway-3} & A1 &1.88 &2647.24 &1.96 &0.69 &3.36 &0.1687$\pm$0.0128 \\ 
        & A2 &6.07 &295.72 &7.42 &1.32 &1.37 &0.0644$\pm$0.0041 \\ 
        & A3 &2.40 &3.24 &3.62 &0.99 &2.70 &0.0649$\pm$0.0083 \\ 
        & A4 &1.83 &10.69 &2.93 &0.79 &2.56 &0.0825$\pm$0.0009 \\ 
        \specialrule{1.2pt}{0.2pt}{1pt}
        \multirow{4}{*}{Overall} &PC1 &7.04$\pm$7.95 &2415.15$\pm$1476.19 &5.53$\pm$6.26 &1.96$\pm$2.40 &5.85$\pm$6.07 &0.1682$\pm$0.0029 \\ 
        &PC2 &2.81$\pm$2.34 &297.44$\pm$148.41 &4.69$\pm$3.54 &0.83$\pm$0.60 &1.21$\pm$0.78 &0.0665$\pm$0.0144 \\ 
        &PC3 &1.61$\pm$0.77 &1.38$\pm$0.89 &2.28$\pm$2.27 &0.63$\pm$0.44 &1.98$\pm$1.93 &0.0611$\pm$0.0025 \\ 
        &PC4 &1.48$\pm$0.61 &4.54$\pm$2.54 &1.78$\pm$1.75 &0.79$\pm$0.37 &2.01$\pm$1.88 &0.0822$\pm$0.0004 \\ 
        \specialrule{1.2pt}{0.2pt}{1pt}
        \end{tabular}
        }%
\end{table}
%=====================

% SYSTEM 2 - CPU
%=====================
\begin{table}[!t]
    \centering
    \footnotesize
    \setlength{\tabcolsep}{1pt}
    \caption{People counting results per video running algorithms in \textbf{System 2} with \textbf{CPU}. KEY -- Ax: algorithm x; MOE: mean opportunity error of people with OTS; COE: cumulative opportunity error of people with OTS; MPE: mean opportunity error all people.
    \label{tab:count_S2cpu}
    }
    \resizebox{\columnwidth}{!}{
    \begin{tabular}{ll|rrr|rr|c}
        \specialrule{1.2pt}{0.2pt}{1pt}
        \multicolumn{1}{c}{\multirow{2}{*}{Video}} & \multicolumn{1}{c|}{\multirow{2}{*}{Alg.}} & \multicolumn{1}{c}{\multirow{2}{*}{MOE}} & \multicolumn{1}{c}{\multirow{2}{*}{COE}} & \multicolumn{1}{c|}{\multirow{2}{*}{MPE}} & \multicolumn{2}{c|}{MOE} & \multicolumn{1}{|c}{\multirow{2}{*}{\begin{tabular}[c]{@{}c@{}}Speed\\ {[}seconds/frame{]}\end{tabular}}} \\
         &  &  &  &  & \multicolumn{1}{c}{Close}  & \multicolumn{1}{c|}{Far} & \\
        \specialrule{1.2pt}{0.2pt}{1pt}
        \multirow{4}{*}{Airport-1} & A1 &1.08 &79.62 &0.73 &0.32 &0.86 &1.9726$\pm$0.0401 \\ 
        & A2 &0.60 &29.72 &1.37 &0.27 &0.42 &0.2807$\pm$0.0095 \\ 
        & A3 &0.63 &0.03 &0.50 &0.17 &0.54 &0.2718$\pm$0.0698 \\ 
        & A4 &0.68 &1.45 &0.91 &0.53 &0.82 &0.7566$\pm$0.0415 \\ \hline 
        \multirow{4}{*}{Airport-2} & A1 &0.93 &77.76 &0.68 &0.16 &0.76 &2.0224$\pm$0.0386 \\ 
        & A2 &0.80 &23.62 &1.65 &0.25 &0.52 &0.2743$\pm$0.0136 \\ 
        & A3 &0.66 &0.10 &0.44 &0.18 &0.52 &0.2685$\pm$0.0725 \\ 
        & A4 &0.67 &1.69 &0.82 &0.51 &0.87 &0.7523$\pm$0.0433 \\ \hline 
        \multirow{4}{*}{Airport-3} & A1 &0.58 &47.30 &0.71 &0.15 &0.32 &2.0834$\pm$0.0465 \\ 
        & A2 &1.16 &18.30 &1.57 &0.40 &0.52 &0.2741$\pm$0.0112 \\ 
        & A3 &0.74 &0.09 &0.74 &0.27 &0.80 &0.2747$\pm$0.0681 \\ 
        & A4 &1.01 &0.82 &1.24 &0.54 &1.14 &0.7489$\pm$0.0486 \\ \hline 
        \multirow{4}{*}{Airport-4} & A1 &2.39 &73.14 &1.27 &0.39 &2.22 &2.0103$\pm$0.0341 \\ 
        & A2 &1.34 &13.59 &3.83 &0.40 &0.73 &0.2708$\pm$0.0135 \\ 
        & A3 &1.76 &0.36 &1.05 &0.39 &1.02 &0.2976$\pm$0.0737 \\ 
        & A4 &1.32 &1.43 &1.77 &0.89 &1.36 &0.7483$\pm$0.0406 \\ \hline \hline 
        \multirow{4}{*}{Mall-1} & A1 &25.96 &247.78 &19.98 &7.27 &20.32 &2.0492$\pm$0.0460 \\ 
        & A2 &5.89 &8.22 &11.86 &1.80 &2.61 &0.2840$\pm$0.0119 \\ 
        & A3 &2.10 &0.59 &6.98 &1.48 &6.12 &0.3257$\pm$0.0754 \\ 
        & A4 &2.24 &0.68 &7.00 &1.45 &6.19 &0.7632$\pm$0.0611 \\ \hline 
        \multirow{4}{*}{Mall-2} & A1 &27.15 &226.33 &21.60 &8.52 &21.02 &2.0991$\pm$0.0383 \\ 
        & A2 &7.76 &5.88 &13.32 &2.20 &3.18 &0.2864$\pm$0.0139 \\ 
        & A3 &2.89 &0.50 &7.24 &1.35 &6.86 &0.3290$\pm$0.0865 \\ 
        & A4 &3.29 &0.63 &7.59 &1.52 &7.17 &0.7585$\pm$0.0482 \\ \hline 
        \multirow{4}{*}{Mall-3} & A1 &7.79 &328.03 &6.23 &2.45 &5.61 &2.1051$\pm$0.0415 \\ 
        & A2 &1.12 &37.47 &2.64 &0.25 &0.75 &0.3041$\pm$0.0253 \\ 
        & A3 &1.56 &0.07 &1.22 &0.40 &1.20 &0.2849$\pm$0.0714 \\ 
        & A4 &1.06 &2.60 &1.40 &0.68 &1.40 &0.7542$\pm$0.0566 \\ \hline 
        \multirow{4}{*}{Mall-4} & A1 &8.13 &249.18 &7.14 &2.40 &6.11 &2.0734$\pm$0.0524 \\ 
        & A2 &2.32 &20.98 &3.31 &0.90 &1.16 &0.3043$\pm$0.0206 \\ 
        & A3 &1.33 &0.10 &1.36 &0.77 &1.00 &0.2903$\pm$0.0690 \\ 
        & A4 &1.45 &1.96 &1.75 &1.03 &1.13 &0.7598$\pm$0.0488 \\ \hline \hline 
        \multirow{4}{*}{Pedestrian-1} & A1 &8.83 &683.47 &7.42 &1.11 &8.24 &2.0761$\pm$0.0497 \\ 
        & A2 &1.69 &44.65 &3.09 &0.35 &0.87 &0.3068$\pm$0.0119 \\ 
        & A3 &1.01 &0.18 &0.93 &0.37 &1.02 &0.2760$\pm$0.0689 \\ 
        & A4 &0.88 &2.76 &1.35 &0.68 &1.13 &0.7497$\pm$0.0423 \\ \hline 
        \multirow{4}{*}{Pedestrian-2} & A1 &9.96 &350.30 &7.33 &1.54 &8.73 &2.0263$\pm$0.0409 \\ 
        & A2 &1.63 &24.43 &4.30 &0.53 &0.94 &0.3125$\pm$0.0112 \\ 
        & A3 &1.82 &0.17 &1.95 &0.70 &1.50 &0.2918$\pm$0.0686 \\ 
        & A4 &1.77 &2.00 &2.28 &1.02 &1.72 &0.7516$\pm$0.0399 \\ \hline 
        \multirow{4}{*}{Pedestrian-3} & A1 &5.54 &275.72 &4.51 &1.81 &3.55 &2.0515$\pm$0.0372 \\ 
        & A2 &0.66 &24.08 &1.64 &0.34 &0.61 &0.3047$\pm$0.0161 \\ 
        & A3 &0.93 &0.12 &0.29 &0.19 &0.37 &0.2779$\pm$0.0698 \\ 
        & A4 &0.95 &1.28 &0.53 &0.52 &0.69 &0.7573$\pm$0.0506 \\ \hline 
        \multirow{4}{*}{Pedestrian-4} & A1 &3.70 &204.88 &2.54 &0.57 &3.78 &2.0454$\pm$0.0484 \\ 
        & A2 &1.16 &59.96 &2.29 &0.61 &0.74 &0.3767$\pm$0.0185 \\ 
        & A3 &1.25 &0.20 &1.04 &0.62 &0.89 &0.2909$\pm$0.0743 \\ 
        & A4 &1.08 &2.04 &1.74 &1.14 &1.04 &0.7528$\pm$0.0507 \\ \hline 
        \multirow{4}{*}{Pedestrian-5} & A1 &3.78 &316.91 &2.39 &0.97 &3.13 &1.9857$\pm$0.0388 \\ 
        & A2 &2.13 &43.45 &3.69 &0.79 &1.20 &0.3319$\pm$0.0187 \\ 
        & A3 &1.71 &0.09 &1.25 &0.35 &0.96 &0.2868$\pm$0.0877 \\ 
        & A4 &1.70 &1.73 &1.18 &0.63 &1.15 &0.7582$\pm$0.0509 \\ \hline \hline 
        \multirow{4}{*}{Subway-1} & A1 &2.20 &251.53 &1.77 &0.63 &2.40 &2.0417$\pm$0.0676 \\ 
        & A2 &4.09 &48.35 &4.90 &1.37 &1.70 &0.2954$\pm$0.0126 \\ 
        & A3 &1.75 &0.06 &2.19 &0.73 &2.02 &0.2996$\pm$0.0838 \\ 
        & A4 &1.34 &2.53 &1.68 &1.05 &1.98 &0.7517$\pm$0.0463 \\ \hline 
        \multirow{4}{*}{Subway-2} & A1 &2.61 &173.71 &2.20 &2.28 &3.22 &2.0307$\pm$0.0458 \\ 
        & A2 &6.53 &28.89 &8.07 &1.48 &2.09 &0.2995$\pm$0.0121 \\ 
        & A3 &2.97 &0.39 &4.34 &1.10 &3.57 &0.3192$\pm$0.0971 \\ 
        & A4 &2.85 &0.89 &4.19 &1.25 &3.78 &0.7510$\pm$0.0319 \\ \hline 
        \multirow{4}{*}{Subway-3} & A1 &1.85 &263.14 &1.97 &0.69 &3.33 &2.0106$\pm$0.0330 \\ 
        & A2 &6.05 &28.55 &7.41 &1.31 &1.37 &0.3006$\pm$0.0114 \\ 
        & A3 &2.26 &0.10 &3.50 &0.94 &2.66 &0.3106$\pm$0.0714 \\ 
        & A4 &2.18 &2.28 &3.46 &0.92 &2.77 &0.7586$\pm$0.0461 \\ 
        \specialrule{1.2pt}{0.2pt}{1pt}
        \multirow{4}{*}{Overall} &PC1 &7.03$\pm$7.93 &240.55$\pm$147.35 &5.53$\pm$6.24 &1.95$\pm$2.38 &5.85$\pm$6.07 &2.0427$\pm$0.0371 \\ 
        &PC2 &2.81$\pm$2.34 &28.76$\pm$14.40 &4.69$\pm$3.54 &0.83$\pm$0.60 &1.21$\pm$0.78 &0.3004$\pm$0.0252 \\ 
        &PC3 &1.58$\pm$0.70 &0.20$\pm$0.16 &2.19$\pm$2.14 &0.63$\pm$0.40 &1.94$\pm$1.90 &0.2935$\pm$0.0184 \\ 
        &PC4 &1.53$\pm$0.74 &1.67$\pm$0.67 &2.43$\pm$2.05 &0.90$\pm$0.32 &2.15$\pm$1.88 &0.7545$\pm$0.0043 \\ 
        \specialrule{1.2pt}{0.2pt}{1pt}
        \end{tabular}
        }%
\end{table}
%=====================

% SYSTEM 3 - CPU
%=====================
\begin{table}[!t]
    \centering
    \small
    \setlength{\tabcolsep}{1pt}
    \caption{People counting results per video running algorithms in \textbf{System 3} (\textbf{CPU}). KEY -- Ax: algorithm x; MOE: mean opportunity error of people with OTS; COE: cumulative opportunity error of people with OTS; MPE: mean opportunity error all people.}
    \label{tab:count_S3}
    \resizebox{\columnwidth}{!}{
    \begin{tabular}{ll|rrr|rr|c}
    \specialrule{1.2pt}{0.2pt}{1pt}
    \multicolumn{1}{c}{\multirow{2}{*}{Video}} & \multicolumn{1}{c|}{\multirow{2}{*}{Alg.}} & \multicolumn{1}{c}{\multirow{2}{*}{MOE}} & \multicolumn{1}{c}{\multirow{2}{*}{COE}} & \multicolumn{1}{c|}{\multirow{2}{*}{MPE}} & \multicolumn{2}{c|}{MOE} & \multicolumn{1}{|c}{\multirow{2}{*}{\begin{tabular}[c]{@{}c@{}}Speed\\ {[}seconds/frame{]}\end{tabular}}} \\
     &  &  &  &  & \multicolumn{1}{c}{Close}  & \multicolumn{1}{c|}{Far} & \\
    \specialrule{1.2pt}{0.2pt}{1pt}
    \multirow{4}{*}{Airport-1} & A1 &1.18 &80.59 &0.86 &0.73 &0.73 &3.1211$\pm$0.0916 \\ 
    & A2 &0.60 &29.72 &1.37 &0.27 &0.42 &0.6828$\pm$0.0444 \\ 
    & A3 &0.63 &0.17 &0.51 &0.16 &0.54 &2.6135$\pm$0.2484 \\ 
    & A4 &0.68 &1.45 &0.91 &0.53 &0.82 &9.2307$\pm$0.2637 \\ \hline 
    \multirow{4}{*}{Airport-2} & A1 &0.72 &63.21 &0.99 &0.16 &0.55 &2.7811$\pm$0.1235 \\ 
    & A2 &0.80 &23.62 &1.65 &0.25 &0.52 &0.6643$\pm$0.0762 \\ 
    & A3 &0.65 &0.17 &0.48 &0.19 &0.53 &2.2832$\pm$0.3388 \\ 
    & A4 &0.67 &1.69 &0.82 &0.51 &0.87 &9.1608$\pm$0.2413 \\ \hline 
    \multirow{4}{*}{Airport-3} & A1 &0.77 &45.93 &0.89 &0.24 &0.48 &3.1335$\pm$0.1700 \\ 
    & A2 &1.16 &18.30 &1.57 &0.40 &0.52 &0.6864$\pm$0.0883 \\ 
    & A3 &0.77 &0.20 &0.77 &0.25 &0.80 &2.6241$\pm$0.2687 \\ 
    & A4 &1.01 &0.82 &1.24 &0.54 &1.14 &9.2028$\pm$0.2565 \\ \hline 
    \multirow{4}{*}{Airport-4} & A1 &1.44 &51.36 &1.81 &0.41 &1.19 &3.1468$\pm$0.2181 \\ 
    & A2 &1.34 &13.59 &3.83 &0.40 &0.73 &0.6835$\pm$0.0719 \\ 
    & A3 &1.62 &0.34 &1.21 &0.41 &1.12 &2.9254$\pm$0.3752 \\ 
    & A4 &1.32 &1.43 &1.77 &0.89 &1.36 &9.5805$\pm$0.5325 \\ \hline \hline 
    \multirow{4}{*}{Mall-1} & A1 &2.72 &47.68 &6.85 &3.85 &2.68 &3.1209$\pm$0.0989 \\ 
    & A2 &5.89 &8.22 &11.86 &1.80 &2.61 &0.7677$\pm$0.1023 \\ 
    & A3 &2.49 &0.61 &7.96 &1.78 &6.32 &3.0050$\pm$0.2875 \\ 
    & A4 &2.24 &0.68 &7.00 &1.45 &6.19 &9.2565$\pm$0.3312 \\ \hline 
    \multirow{4}{*}{Mall-2} & A1 &3.50 &57.29 &5.68 &6.03 &3.23 &2.7740$\pm$0.1025 \\ 
    & A2 &7.76 &5.88 &13.32 &2.20 &3.18 &0.7604$\pm$0.0542 \\ 
    & A3 &3.30 &0.61 &8.14 &1.51 &7.02 &2.7213$\pm$0.3596 \\ 
    & A4 &3.29 &0.63 &7.59 &1.52 &7.17 &9.2638$\pm$0.4218 \\ \hline 
    \multirow{4}{*}{Mall-3} & A1 &1.51 &92.20 &1.75 &0.63 &1.05 &2.7840$\pm$0.1521 \\ 
    & A2 &1.12 &37.47 &2.64 &0.25 &0.75 &0.8176$\pm$0.1507 \\ 
    & A3 &1.03 &0.23 &1.25 &0.42 &1.33 &2.3666$\pm$0.2388 \\ 
    & A4 &1.06 &2.60 &1.40 &0.68 &1.40 &9.2656$\pm$0.3036 \\ \hline 
    \multirow{4}{*}{Mall-4} & A1 &1.44 &60.04 &1.89 &0.76 &1.18 &2.7724$\pm$0.0874 \\ 
    & A2 &2.32 &20.98 &3.31 &0.90 &1.16 &0.8281$\pm$0.1137 \\ 
    & A3 &1.28 &0.30 &1.72 &0.81 &1.05 &2.3343$\pm$0.2259 \\ 
    & A4 &1.45 &1.96 &1.75 &1.03 &1.13 &9.2329$\pm$0.2718 \\ \hline \hline 
    \multirow{4}{*}{Pedestrian-1} & A1 &1.74 &223.88 &1.71 &1.54 &1.03 &3.1590$\pm$0.2639 \\ 
    & A2 &1.69 &44.65 &3.09 &0.35 &0.87 &0.8501$\pm$0.0585 \\ 
    & A3 &0.97 &0.18 &1.11 &0.43 &1.11 &2.6965$\pm$0.2829 \\ 
    & A4 &0.88 &2.76 &1.35 &0.68 &1.13 &9.2648$\pm$0.3023 \\ \hline 
    \multirow{4}{*}{Pedestrian-2} & A1 &2.66 &115.03 &2.64 &1.40 &1.66 &3.1205$\pm$0.0994 \\ 
    & A2 &1.63 &24.43 &4.30 &0.53 &0.94 &0.9135$\pm$0.0479 \\ 
    & A3 &1.68 &0.20 &2.27 &0.69 &1.72 &2.8511$\pm$0.3266 \\ 
    & A4 &1.77 &2.00 &2.28 &1.02 &1.72 &9.3215$\pm$0.2994 \\ \hline 
    \multirow{4}{*}{Pedestrian-3} & A1 &3.01 &167.68 &2.29 &0.59 &2.40 &2.7755$\pm$0.0917 \\ 
    & A2 &0.66 &24.08 &1.64 &0.34 &0.61 &0.8593$\pm$0.1070 \\ 
    & A3 &0.91 &0.04 &0.31 &0.20 &0.37 &2.3097$\pm$0.2178 \\ 
    & A4 &0.95 &1.28 &0.53 &0.52 &0.69 &9.2629$\pm$0.2010 \\ \hline 
    \multirow{4}{*}{Pedestrian-4} & A1 &1.75 &122.28 &1.76 &0.53 &1.65 &2.7990$\pm$0.2282 \\ 
    & A2 &1.16 &59.96 &2.29 &0.61 &0.74 &1.1712$\pm$0.0743 \\ 
    & A3 &1.05 &0.20 &1.38 &0.77 &0.90 &2.4043$\pm$0.2237 \\ 
    & A4 &1.08 &2.04 &1.74 &1.14 &1.04 &9.1818$\pm$0.2202 \\ \hline \hline 
    \multirow{4}{*}{Pedestrian-5} & A1 &2.56 &187.00 &2.14 &1.07 &1.73 &3.1169$\pm$0.0680 \\ 
    & A2 &2.13 &43.45 &3.69 &0.79 &1.20 &1.0555$\pm$0.1597 \\ 
    & A3 &1.94 &0.27 &1.53 &0.46 &1.11 &2.7614$\pm$0.2753 \\ 
    & A4 &1.70 &1.73 &1.18 &0.63 &1.15 &10.3829$\pm$0.3096 \\ \hline 
    \multirow{4}{*}{Subway-1} & A1 &1.54 &201.24 &1.64 &0.94 &1.35 &3.1159$\pm$0.0648 \\ 
    & A2 &4.09 &48.35 &4.90 &1.37 &1.70 &0.7848$\pm$0.0499 \\ 
    & A3 &1.76 &0.00 &2.21 &0.67 &1.97 &3.2397$\pm$0.5878 \\ 
    & A4 &1.34 &2.53 &1.68 &1.05 &1.98 &9.2658$\pm$0.1809 \\ \hline 
    \multirow{4}{*}{Subway-2} & A1 &2.82 &93.71 &4.14 &2.10 &1.79 &2.7722$\pm$0.0578 \\ 
    & A2 &6.53 &28.89 &8.07 &1.48 &2.09 &0.7965$\pm$0.0458 \\ 
    & A3 &2.91 &0.46 &4.27 &1.07 &3.58 &2.9767$\pm$0.4330 \\ 
    & A4 &2.85 &0.89 &4.19 &1.25 &3.78 &9.1634$\pm$0.1038 \\ \hline 
    \multirow{4}{*}{Subway-3} & A1 &2.01 &209.83 &2.79 &0.96 &1.96 &3.1218$\pm$0.0892 \\ 
    & A2 &6.05 &28.55 &7.41 &1.31 &1.37 &0.7953$\pm$0.0445 \\ 
    & A3 &2.21 &0.03 &3.43 &0.87 &2.67 &3.4676$\pm$0.5441 \\ 
    & A4 &2.18 &2.28 &3.46 &0.92 &2.77 &11.2567$\pm$1.6378 \\ 
     \specialrule{1.2pt}{0.2pt}{1pt}
    \multirow{4}{*}{Overall} &A1 &1.96$\pm$0.80 &113.68$\pm$61.65 &2.49$\pm$1.64 &1.37$\pm$1.48 &1.54$\pm$0.74 &2.9759$\pm$0.1734 \\ 
    &A2 &2.81$\pm$2.34 &28.76$\pm$14.40 &4.69$\pm$3.54 &0.83$\pm$0.60 &1.21$\pm$0.78 &0.8198$\pm$0.1319 \\
    &A3 &1.57$\pm$0.79 &0.25$\pm$0.18 &2.41$\pm$2.36 &0.67$\pm$0.45 &2.01$\pm$1.94 &2.7238$\pm$0.3345 \\ 
    &A4 &1.53$\pm$0.74 &1.67$\pm$0.67 &2.43$\pm$2.05 &0.90$\pm$0.32 &2.15$\pm$1.88 &9.4558$\pm$0.5461 \\ 
    \specialrule{1.2pt}{0.2pt}{1pt}
    \end{tabular}
    }%
\end{table}
%=====================

% SYSTEM 4 - GPU
%=====================
\begin{table}[!t]
    \centering
    \small
    \setlength{\tabcolsep}{1pt}
    \caption{People counting results per video running algorithms in \textbf{System 4} (\textbf{GPU}). KEY -- Ax: algorithm x; MOE: mean opportunity error of people with OTS; COE: cumulative opportunity error of people with OTS; MPE: mean opportunity error all people.}
    \label{tab:count_S4}
    \resizebox{\columnwidth}{!}{
    \begin{tabular}{ll|rrr|rr|c}
    \specialrule{1.2pt}{0.2pt}{1pt}
    \multicolumn{1}{c}{\multirow{2}{*}{Video}} & \multicolumn{1}{c|}{\multirow{2}{*}{Alg.}} & \multicolumn{1}{c}{\multirow{2}{*}{MOE}} & \multicolumn{1}{c}{\multirow{2}{*}{COE}} & \multicolumn{1}{c|}{\multirow{2}{*}{MPE}} & \multicolumn{2}{c|}{MOE} & \multicolumn{1}{|c}{\multirow{2}{*}{\begin{tabular}[c]{@{}c@{}}Speed\\ {[}seconds/frame{]}\end{tabular}}} \\
     &  &  &  &  & \multicolumn{1}{c}{Close}  & \multicolumn{1}{c|}{Far} & \\
    \specialrule{1.2pt}{0.2pt}{1pt}
    \multirow{4}{*}{Airport-1} & A1 &1.07 &79.07 &0.73 &0.31 &0.86 &3.4423$\pm$0.9443 \\ 
    & A2 &0.60 &30.21 &1.37 &0.27 &0.44 &1.2229$\pm$0.3766 \\ 
    & A3 &0.64 &0.00 &0.50 &0.17 &0.53 &0.9952$\pm$0.3738 \\ 
    & A4 &0.67 &1.48 &0.91 &0.52 &0.82 &2.9256$\pm$1.7384 \\ \hline 
    \multirow{4}{*}{Airport-2} & A1 &0.91 &76.93 &0.67 &0.14 &0.75 &3.4354$\pm$1.0196 \\ 
    & A2 &0.81 &23.66 &1.65 &0.25 &0.52 &1.2442$\pm$0.4019 \\ 
    & A3 &0.66 &0.10 &0.45 &0.17 &0.52 &0.9794$\pm$0.2883 \\ 
    & A4 &0.67 &1.76 &0.82 &0.49 &0.88 &2.8904$\pm$1.4831 \\ \hline 
    \multirow{4}{*}{Airport-3} & A1 &0.58 &47.07 &0.71 &0.15 &0.32 &3.4276$\pm$0.8300 \\ 
    & A2 &1.16 &18.45 &1.57 &0.40 &0.51 &1.2157$\pm$0.3349 \\ 
    & A3 &0.75 &0.05 &0.74 &0.26 &0.79 &0.9624$\pm$0.3050 \\ 
    & A4 &1.02 &0.86 &1.23 &0.54 &1.15 &2.9042$\pm$1.5228 \\ \hline 
    \multirow{4}{*}{Airport-4} & A1 &2.37 &72.98 &1.24 &0.40 &2.20 &3.4382$\pm$0.9419 \\ 
    & A2 &1.34 &13.62 &3.83 &0.40 &0.73 &1.2526$\pm$0.5385 \\ 
    & A3 &1.77 &0.32 &1.04 &0.38 &1.00 &1.0445$\pm$0.4132 \\ 
    & A4 &1.33 &1.38 &1.74 &0.87 &1.34 &2.9489$\pm$1.9642 \\ \hline \hline 
    \multirow{4}{*}{Mall-1} & A1 &25.72 &246.01 &19.75 &7.12 &20.23 &3.4630$\pm$0.9921 \\ 
    & A2 &5.87 &8.37 &11.84 &1.78 &2.61 &1.3272$\pm$0.2915 \\ 
    & A3 &2.15 &0.55 &7.05 &1.49 &6.12 &1.1008$\pm$0.4174 \\ 
    & A4 &2.24 &0.69 &7.02 &1.48 &6.20 &2.9410$\pm$1.7516 \\ \hline 
    \multirow{4}{*}{Mall-2} & A1 &26.95 &225.06 &21.40 &8.38 &20.95 &3.4954$\pm$1.3750 \\ 
    & A2 &7.76 &5.86 &13.32 &2.21 &3.18 &1.3812$\pm$0.6119 \\ 
    & A3 &2.86 &0.58 &7.24 &1.41 &6.87 &1.1307$\pm$0.3119 \\ 
    & A4 &3.24 &0.62 &7.61 &1.51 &7.17 &2.9592$\pm$1.8616 \\ \hline 
    \multirow{4}{*}{Mall-3} & A1 &8.04 &336.27 &6.48 &2.48 &5.83 &3.4587$\pm$1.1315 \\ 
    & A2 &1.14 &36.20 &2.66 &0.23 &0.76 &1.4139$\pm$0.5515 \\ 
    & A3 &1.56 &0.13 &1.25 &0.40 &1.22 &1.0205$\pm$0.3668 \\ 
    & A4 &1.05 &2.50 &1.39 &0.67 &1.38 &2.9122$\pm$1.2880 \\ \hline 
    \multirow{4}{*}{Mall-4} & A1 &8.24 &251.66 &7.25 &2.33 &6.29 &3.4572$\pm$1.1774 \\ 
    & A2 &2.32 &20.98 &3.31 &0.90 &1.16 &0.8281$\pm$0.1137 \\ 
    & A3 &1.31 &0.08 &1.38 &0.78 &1.02 &1.0196$\pm$0.2916 \\ 
    & A4 &1.42 &1.84 &1.74 &1.03 &1.13 &2.8956$\pm$1.5219 \\ \hline \hline 
    \multirow{4}{*}{Pedestrian-1} & A1 &8.80 &681.59 &7.39 &1.20 &8.11 &3.4504$\pm$1.1230 \\ 
    & A2 &1.67 &46.29 &3.06 &0.36 &0.86 &1.4107$\pm$0.3994 \\ 
    & A3 &1.01 &0.12 &0.94 &0.37 &1.02 &0.9975$\pm$0.3210 \\ 
    & A4 &0.91 &2.76 &1.30 &0.71 &1.14 &2.9077$\pm$1.5529 \\ \hline 
    \multirow{4}{*}{Pedestrian-2} & A1 &9.87 &347.65 &7.24 &1.45 &8.73 &3.4347$\pm$0.8917 \\ 
    & A2 &1.63 &24.57 &4.29 &0.54 &0.95 &1.4599$\pm$0.3652 \\ 
    & A3 &1.84 &0.33 &1.91 &0.68 &1.47 &1.0363$\pm$0.3373 \\ 
    & A4 &1.79 &2.10 &2.19 &1.01 &1.67 &2.9221$\pm$1.6302 \\ \hline 
    \multirow{4}{*}{Pedestrian-3} & A1 &5.54 &276.00 &4.51 &1.69 &3.67 &3.4541$\pm$0.8684 \\ 
    & A2 &0.66 &24.36 &1.63 &0.32 &0.60 &1.4534$\pm$0.4563 \\ 
    & A3 &0.92 &0.16 &0.29 &0.19 &0.37 &0.9797$\pm$0.2537 \\ 
    & A4 &0.93 &1.32 &0.55 &0.53 &0.70 &2.8981$\pm$1.6012 \\ \hline 
    \multirow{4}{*}{Pedestrian-4} & A1 &3.68 &204.32 &2.53 &0.63 &3.71 &3.4375$\pm$1.0487 \\ 
    & A2 &1.16 &59.96 &2.29 &0.61 &0.74 &1.1712$\pm$0.0743 \\ 
    & A3 &1.23 &0.16 &1.05 &0.62 &0.89 &1.0046$\pm$0.3547 \\ 
    & A4 &1.08 &1.96 &1.73 &1.13 &1.04 &2.9194$\pm$1.6676 \\ \hline 
    \multirow{4}{*}{Pedestrian-5} & A1 &3.72 &313.45 &2.38 &1.00 &3.07 &3.4851$\pm$1.4734 \\ 
    & A2 &2.13 &43.45 &3.69 &0.79 &1.20 &1.0555$\pm$0.1597 \\ 
    & A3 &1.70 &0.09 &1.27 &0.33 &0.98 &1.0331$\pm$0.6007 \\ 
    & A4 &1.70 &1.36 &1.19 &0.62 &1.15 &3.0618$\pm$2.9069 \\ \hline \hline 
    \multirow{4}{*}{Subway-1} & A1 &2.28 &254.76 &1.81 &0.64 &2.47 &3.4661$\pm$1.3278 \\ 
    & A2 &4.11 &47.82 &4.92 &1.39 &1.69 &1.3494$\pm$0.4645 \\ 
    & A3 &1.74 &0.06 &2.18 &0.72 &2.02 &1.0657$\pm$0.4566 \\ 
    & A4 &1.29 &2.53 &1.67 &1.04 &1.95 &2.9754$\pm$2.0026 \\ \hline 
    \multirow{4}{*}{Subway-2} & A1 &2.72 &175.57 &2.27 &2.35 &3.23 &3.4841$\pm$1.4000 \\ 
    & A2 &6.49 &29.46 &8.04 &1.49 &2.07 &1.4148$\pm$0.6504 \\ 
    & A3 &2.94 &0.32 &4.31 &1.11 &3.57 &1.1146$\pm$0.4399 \\ 
    & A4 &2.86 &1.00 &4.22 &1.28 &3.77 &2.9906$\pm$1.9275 \\ \hline 
    \multirow{4}{*}{Subway-3} & A1 &1.84 &262.93 &1.93 &0.69 &3.32 &3.4864$\pm$1.1692 \\ 
    & A2 &6.06 &28.31 &7.42 &1.31 &1.38 &1.9446$\pm$0.1390 \\ 
    & A3 &2.24 &0.28 &3.49 &0.94 &2.66 &1.1066$\pm$0.3553 \\ 
    & A4 &2.14 &2.21 &3.43 &0.90 &2.73 &2.9359$\pm$1.5218 \\ 
    \specialrule{1.2pt}{0.2pt}{1pt}
    \multirow{4}{*}{Overall} &A1 &7.02$\pm$7.86 &240.71$\pm$147.21 &5.52$\pm$6.17 &1.94$\pm$2.33 &5.86$\pm$6.05 &3.4573$\pm$0.0206 \\ 
    &A2 &2.81$\pm$2.33 &28.85$\pm$14.40 &4.68$\pm$3.54 &0.83$\pm$0.60 &1.21$\pm$0.78 &2.5716$\pm$5.0047 \\
    &A3 &1.58$\pm$0.70 &0.21$\pm$0.17 &2.19$\pm$2.15 &0.63$\pm$0.41 &1.94$\pm$1.91 &1.0369$\pm$0.0511 \\ 
    &A4 &1.52$\pm$0.74 &1.65$\pm$0.65 &2.42$\pm$2.06 &0.90$\pm$0.32 &2.14$\pm$1.88 &2.9368$\pm$0.0427 \\ 
    \specialrule{1.2pt}{0.2pt}{1pt}
    \end{tabular}
    }%
\end{table}
%=====================

% Commercial detection
%=====================
\begin{table}[!t]
    \centering
    \small
    \setlength{\tabcolsep}{1pt}
    \caption{Localization results per video running algorithms with \textbf{commercial solutions} (C1 and C2).  KEY -- Ax: algorithm x; P: precision; R: recall; F: F1-Score. A1-4 were run in System 1 with GPU. C1-2 were run in two other systems with Intel i7 CPU.}
    \label{tab:detection_results_commercial}
    \resizebox{\columnwidth}{!}{
    \begin{tabular}{lc|ccc|cc|ccc|c}
    \specialrule{1.2pt}{0.2pt}{1pt}
    \multicolumn{1}{c}{\multirow{2}{*}{Video}} & \multicolumn{1}{c|}{\multirow{2}{*}{Alg.}} & \multicolumn{1}{c}{\multirow{2}{*}{P}} & \multicolumn{1}{c}{\multirow{2}{*}{R}} & \multicolumn{1}{c|}{\multirow{2}{*}{F}} & \multicolumn{2}{c|}{Recall distance} &
    \multicolumn{3}{c|}{Recall occlusion} &
    \multicolumn{1}{|c}{\multirow{2}{*}{\begin{tabular}[c]{@{}c@{}}Speed\\ {[}seconds/frame{]}\end{tabular}}} \\
     &  &  &  &  & \multicolumn{1}{c}{Close}  & \multicolumn{1}{c|}{Far} & \multicolumn{1}{c}{No}  & \multicolumn{1}{c}{Partial}  & \multicolumn{1}{c|}{Heavy} & \\
    \specialrule{1.2pt}{0.2pt}{1pt}
    \multirow{6}{*}{Airport-1} & A1 &0.61 &0.66 &0.62 &0.53 &0.32 &0.67 &0.01 &0.00 &0.0414$\pm$0.0129 \\ 
    & A2 &0.57 &0.49 &0.51 &0.41 &0.22 &0.50 &0.00 &0.00 &0.0277$\pm$0.0030 \\ 
    & A3 &0.89 &0.75 &0.80 &0.70 &0.40 &0.79 &0.02 &0.00 &0.0845$\pm$0.0130 \\ 
    & A4 &0.89 &0.79 &0.82 &0.69 &0.49 &0.84 &0.02 &0.00 &0.0800$\pm$0.0006 \\ 
    & C1 &0.52 &0.45 &0.47 &0.42 &0.16 &0.45 &0.01 &0.00 &0.0261$\pm$0.0358 \\ 
    & A6 &0.56 &0.49 &0.51 &0.38 &0.25 &0.49 &0.00 &0.00 &0.0620$\pm$0.0289 \\ \hline 
    \multirow{6}{*}{Airport-2} & A1 &0.55 &0.73 &0.60 &0.51 &0.46 &0.73 &0.01 &0.01 &0.1728$\pm$0.0195 \\ 
    & A2 &0.47 &0.35 &0.39 &0.36 &0.12 &0.35 &0.00 &0.00 &0.0274$\pm$0.0049 \\ 
    & A3 &0.83 &0.74 &0.77 &0.68 &0.42 &0.77 &0.01 &0.01 &0.0828$\pm$0.0128 \\ 
    & A4 &0.84 &0.78 &0.80 &0.68 &0.49 &0.83 &0.04 &0.01 &0.0805$\pm$0.0009 \\
    & C1 &0.44 &0.36 &0.38 &0.38 &0.12 &0.37 &0.00 &0.00 &0.0303$\pm$0.0363 \\ 
    & C2 &0.52 &0.43 &0.46 &0.38 &0.20 &0.43 &0.00 &0.00 &0.0541$\pm$0.0319 \\ \hline \hline 
    \multirow{6}{*}{Mall-3} & A1 &0.34 &0.84 &0.46 &0.54 &0.56 &0.82 &0.02 &0.03 &0.1739$\pm$0.0192 \\ 
    & A2 &0.57 &0.43 &0.47 &0.44 &0.11 &0.43 &0.00 &0.00 &0.0446$\pm$0.0128 \\ 
    & A3 &0.90 &0.71 &0.77 &0.77 &0.35 &0.83 &0.04 &0.01 &0.0822$\pm$0.0126 \\ 
    & A4 &0.91 &0.77 &0.81 &0.77 &0.46 &0.90 &0.07 &0.01 &0.0809$\pm$0.0009 \\ 
    & C1 &0.41 &0.32 &0.34 &0.40 &0.00 &0.32 &0.00 &0.00 &0.0331$\pm$0.0369 \\ 
    & C2 &0.46 &0.30 &0.35 &0.30 &0.08 &0.31 &0.00 &0.00 &0.0703$\pm$0.0280 \\ \hline 
    \multirow{6}{*}{Mall-4} & A1 &0.45 &0.90 &0.58 &0.74 &0.70 &0.91 &0.06 &0.04 &0.1728$\pm$0.0183 \\ 
    & A2 &0.53 &0.25 &0.32 &0.24 &0.11 &0.26 &0.01 &0.00 &0.0465$\pm$0.0101 \\ 
    & A3 &0.91 &0.61 &0.71 &0.55 &0.58 &0.66 &0.05 &0.02 &0.0849$\pm$0.0121 \\ 
    & A4 &0.86 &0.66 &0.73 &0.53 &0.69 &0.71 &0.06 &0.02 &0.0805$\pm$0.0005 \\ 
    & C1 &0.39 &0.19 &0.25 &0.25 &0.02 &0.20 &0.01 &0.00 &0.0318$\pm$0.0351 \\ 
    & C2 &0.47 &0.21 &0.28 &0.18 &0.14 &0.22 &0.00 &0.00 &0.0801$\pm$0.0309 \\ \hline \hline 
    \multirow{6}{*}{Pedestrian-2} & A1 &0.51 &0.44 &0.43 &0.51 &0.11 &0.46 &0.01 &0.00 &0.0421$\pm$0.0108 \\ 
    & A2 &0.51 &0.31 &0.36 &0.37 &0.07 &0.32 &0.00 &0.00 &0.0571$\pm$0.0032 \\ 
    & A3 &0.89 &0.59 &0.69 &0.73 &0.30 &0.73 &0.13 &0.01 &0.0839$\pm$0.0124 \\ 
    & A4 &0.88 &0.69 &0.75 &0.74 &0.48 &0.86 &0.16 &0.00 &0.0813$\pm$0.0007 \\ 
    & C1 &0.47 &0.34 &0.36 &0.46 &0.01 &0.35 &0.01 &0.00 &0.0435$\pm$0.0361 \\ 
    & C2 &0.51 &0.28 &0.34 &0.33 &0.06 &0.31 &0.00 &0.00 &0.0959$\pm$0.0274 \\ \hline 
    \multirow{6}{*}{Pedestrian-3} & A1 &0.35 &0.75 &0.47 &0.48 &0.44 &0.74 &0.02 &0.00 &0.1736$\pm$0.0187 \\ 
    & A2 &0.35 &0.27 &0.30 &0.28 &0.07 &0.28 &0.00 &0.00 &0.0522$\pm$0.0067 \\ 
    & A3 &0.94 &0.86 &0.89 &0.70 &0.47 &0.88 &0.05 &0.01 &0.0835$\pm$0.0138 \\ 
    & A4 &0.93 &0.87 &0.90 &0.68 &0.51 &0.90 &0.04 &0.00 &0.0808$\pm$0.0010 \\ 
    & C1 &0.36 &0.28 &0.30 &0.32 &0.04 &0.27 &0.00 &0.00 &0.0278$\pm$0.0338 \\ 
    & C2 &0.36 &0.27 &0.30 &0.24 &0.09 &0.27 &0.00 &0.00 &0.0548$\pm$0.0251 \\ 
    \specialrule{1.2pt}{0.2pt}{1pt}
    \multirow{6}{*}{Overall} &A1 &0.47$\pm$0.10 &0.72$\pm$0.15 &0.53$\pm$0.07 &0.55$\pm$0.09 &0.55$\pm$0.09 &0.72$\pm$0.14 &0.02$\pm$0.02 &0.01$\pm$0.01 &0.1294$\pm$0.0620 \\ 
    &A2 &0.50$\pm$0.07 &0.35$\pm$0.09 &0.39$\pm$0.08 &0.35$\pm$0.07 &0.35$\pm$0.07 &0.36$\pm$0.08 &0.00$\pm$0.00 &0.00$\pm$0.00 &0.0426$\pm$0.0114 \\ 
    &A3 &0.89$\pm$0.03 &0.71$\pm$0.09 &0.77$\pm$0.06 &0.69$\pm$0.07 &0.69$\pm$0.07 &0.78$\pm$0.07 &0.05$\pm$0.04 &0.01$\pm$0.00 &0.0836$\pm$0.0009 \\ 
    &A4 &0.88$\pm$0.03 &0.76$\pm$0.07 &0.80$\pm$0.05 &0.68$\pm$0.08 &0.68$\pm$0.08 &0.84$\pm$0.06 &0.06$\pm$0.04 &0.01$\pm$0.01 &0.0807$\pm$0.0004 \\ 
    &C1 &0.43$\pm$0.05 &0.32$\pm$0.08 &0.35$\pm$0.07 &0.37$\pm$0.07 &0.37$\pm$0.07 &0.33$\pm$0.08 &0.01$\pm$0.00 &0.00$\pm$0.00 &0.0321$\pm$0.0056 \\ 
    &C2 &0.48$\pm$0.06 &0.33$\pm$0.10 &0.37$\pm$0.08 &0.30$\pm$0.07 &0.30$\pm$0.07 &0.34$\pm$0.09 &0.00$\pm$0.00 &0.00$\pm$0.00 &0.0695$\pm$0.0148 \\ 
    \specialrule{1.2pt}{0.2pt}{1pt}
    \end{tabular}
    }%
\end{table}
%=====================

% Commercial counting
%=====================
\begin{table}[!t]
    \centering
    \small
    \setlength{\tabcolsep}{1pt}
    \caption{People counting results per video running algorithms with \textbf{commercial solutions} (C1 and C2).  KEY -- Ax: algorithm x; MOE: mean opportunity error of people with OTS; COE: cumulative opportunity error of people with OTS; MPE: mean opportunity error all people. A1-4 were run in System 1 with GPU. C1-2 were run in two other systems with Intel i7 CPU.}
    \label{tab:count_commercial}
    \resizebox{\columnwidth}{!}{
    \begin{tabular}{ll|rrr|rr|c}
    \specialrule{1.2pt}{0.2pt}{1pt}
    \multicolumn{1}{c}{\multirow{2}{*}{Video}} & \multicolumn{1}{c|}{\multirow{2}{*}{Alg.}} & \multicolumn{1}{c}{\multirow{2}{*}{MOE}} & \multicolumn{1}{c}{\multirow{2}{*}{COE}} & \multicolumn{1}{c|}{\multirow{2}{*}{MPE}} & \multicolumn{2}{c|}{MOE} & \multicolumn{1}{|c}{\multirow{2}{*}{\begin{tabular}[c]{@{}c@{}}Speed\\ {[}seconds/frame{]}\end{tabular}}} \\
     &  &  &  &  & \multicolumn{1}{c}{Close}  & \multicolumn{1}{c|}{Far} & \\
    \specialrule{1.2pt}{0.2pt}{1pt}
    \multirow{6}{*}{Airport-1} & A1 &0.55 &503.52 &0.89 &0.19 &0.47 &0.0414$\pm$0.0129 \\ 
    & A2 &0.58 &310.28 &1.37 &0.27 &0.43 &0.0277$\pm$0.0030 \\ 
    & A3 &0.64 &0.79 &0.47 &0.15 &0.56 &0.0845$\pm$0.0130 \\ 
    & A4 &0.72 &1.66 &0.33 &0.36 &0.64 &0.0800$\pm$0.0006 \\ 
    & C1 &0.63 &0.24 &1.44 &0.42 &0.57 &0.0261$\pm$0.0358 \\ 
    & C2 &0.58 &4.48 &1.39 &0.26 &0.40 &0.0620$\pm$0.0289 \\ \hline 
    \multirow{6}{*}{Airport-2} & A1 &0.92 &783.55 &0.67 &0.15 &0.76 &0.1728$\pm$0.0195 \\ 
    & A2 &0.79 &248.07 &1.63 &0.25 &0.51 &0.0274$\pm$0.0049 \\ 
    & A3 &0.66 &0.34 &0.44 &0.16 &0.52 &0.0828$\pm$0.0128 \\ 
    & A4 &0.74 &1.07 &0.25 &0.50 &0.69 &0.0805$\pm$0.0009 \\ 
    & C1 &0.72 &0.31 &1.48 &0.41 &0.56 &0.0303$\pm$0.0363 \\ 
    & C2 &0.71 &5.52 &1.49 &0.26 &0.46 &0.0541$\pm$0.0319 \\ \hline \hline 
    \multirow{6}{*}{Mall-3} & A1 &7.76 &3278.23 &6.20 &2.45 &5.58 &0.1739$\pm$0.0192 \\ 
    & A2 &1.15 &378.17 &2.65 &0.24 &0.78 &0.0446$\pm$0.0128 \\ 
    & A3 &1.47 &2.97 &1.26 &0.38 &1.23 &0.0822$\pm$0.0126 \\ 
    & A4 &1.27 &6.00 &0.96 &0.57 &1.30 &0.0809$\pm$0.0009 \\ 
    & C1 &1.37 &0.03 &2.82 &0.30 &0.95 &0.0331$\pm$0.0369 \\ 
    & C2 &1.49 &14.97 &3.02 &0.45 &0.88 &0.0703$\pm$0.0280 \\ \hline 
    \multirow{6}{*}{Mall-4} & A1 &8.13 &2499.30 &7.13 &2.37 &6.13 &0.1728$\pm$0.0183 \\ 
    & A2 &2.44 &190.66 &3.43 &0.91 &1.22 &0.0465$\pm$0.0101 \\ 
    & A3 &1.35 &1.72 &1.39 &0.76 &1.01 &0.0849$\pm$0.0121 \\ 
    & A4 &1.46 &5.12 &1.15 &0.80 &1.00 &0.0805$\pm$0.0005 \\ 
    & C1 &2.52 &0.36 &3.51 &0.81 &1.47 &0.0318$\pm$0.0351 \\ 
    & C2 &2.51 &11.66 &3.50 &0.97 &1.28 &0.0801$\pm$0.0309 \\ \hline \hline 
    \multirow{6}{*}{Pedestrian-2} & A1 &1.56 &568.58 &3.25 &0.66 &1.01 &0.0421$\pm$0.0108 \\ 
    & A2 &1.64 &255.97 &4.28 &0.54 &0.95 &0.0571$\pm$0.0032 \\ 
    & A3 &1.77 &2.10 &2.05 &0.69 &1.55 &0.0839$\pm$0.0124 \\ 
    & A4 &2.00 &8.38 &1.72 &0.72 &1.56 &0.0813$\pm$0.0007 \\ 
    & C1 &1.58 &0.15 &4.12 &0.39 &1.11 &0.0435$\pm$0.0361 \\ 
    & C2 &1.79 &14.12 &4.46 &0.54 &1.03 &0.0959$\pm$0.0274 \\ \hline 
    \multirow{6}{*}{Pedestrian-3} & A1 &5.60 &2791.24 &4.57 &1.79 &3.63 &0.1736$\pm$0.0187 \\ 
    & A2 &0.66 &248.40 &1.64 &0.34 &0.61 &0.0522$\pm$0.0067 \\ 
    & A3 &0.92 &0.76 &0.30 &0.18 &0.40 &0.0835$\pm$0.0138 \\ 
    & A4 &0.97 &2.60 &0.21 &0.45 &0.57 &0.0808$\pm$0.0010 \\ 
    & C1 &0.65 &0.12 &1.61 &0.37 &0.71 &0.0278$\pm$0.0338 \\ 
    & C2 &0.70 &10.44 &1.69 &0.36 &0.59 &0.0548$\pm$0.0251 \\ 
    \specialrule{1.2pt}{0.2pt}{1pt}
    \multirow{6}{*}{Overall} &A1 &4.09$\pm$3.19 &1737.40$\pm$1144.82 &3.79$\pm$2.45 &1.27$\pm$0.97 &2.93$\pm$2.32 &0.1294$\pm$0.0620 \\ 
    &A2 &1.21$\pm$0.65 &271.92$\pm$58.79 &2.50$\pm$1.07 &0.42$\pm$0.24 &0.75$\pm$0.27 &0.0426$\pm$0.0114 \\ 
    &A3 &1.13$\pm$0.43 &1.45$\pm$0.91 &0.99$\pm$0.63 &0.39$\pm$0.25 &0.88$\pm$0.42 &0.0836$\pm$0.0009 \\ 
    &A4 &1.19$\pm$0.45 &4.14$\pm$2.59 &0.77$\pm$0.56 &0.57$\pm$0.15 &0.96$\pm$0.37 &0.0807$\pm$0.0004 \\ 
    &C1 &1.24$\pm$0.68 &0.20$\pm$0.11 &2.50$\pm$1.06 &0.45$\pm$0.16 &0.90$\pm$0.32 &0.0321$\pm$0.0056 \\ 
    &C2 &1.29$\pm$0.70 &10.20$\pm$3.98 &2.59$\pm$1.15 &0.47$\pm$0.24 &0.77$\pm$0.32 &0.0695$\pm$0.0148 \\ 
    \specialrule{1.2pt}{0.2pt}{1pt}
    \end{tabular}
    }%
\end{table}
%=====================

Localization results per video with commercial solutions in Table~\ref{tab:detection_results_commercial}.

People counting results per video with commercial solutions in  Table~\ref{tab:count_commercial}.

\section*{Appendix C: Age estimation results per video}

Age estimation results per video in
System 1-GPU in Table~\ref{tab:age_results_S1gpu},
System 1-CPU in Table~\ref{tab:age_results_S1cpu},
System 2-GPU in Table~\ref{tab:age_results_S2gpu},
System 2-CPU in Table~\ref{tab:age_results_S2cpu},
System 3 in Table~\ref{tab:age_results_S3}, and
System 4 in Table~\ref{tab:age_results_S4}.

% SYSTEM 1 - GPU
%=====================
\begin{table}[!t]
    \centering
    \footnotesize
    \setlength{\tabcolsep}{1pt}
    \caption{Age estimation results per video running algorithms in \textbf{System 1} with \textbf{GPU}. KEY -- Ax: algorithm x; F: F1-Score.}
    \label{tab:age_results_S1gpu}
    %\resizebox{\columnwidth}{!}{
      \begin{tabular}{lc|cccc|c}
        \specialrule{1.2pt}{0.2pt}{1pt}
        \multicolumn{1}{c}{\multirow{2}{*}{Video}} & \multicolumn{1}{c|}{\multirow{2}{*}{Alg.}} & \multicolumn{4}{c|}{F1-Score} &
        \multicolumn{1}{|c}{\multirow{2}{*}{\begin{tabular}[c]{@{}c@{}}Speed\\ {[}seconds/frame{]}\end{tabular}}} \\
         &  & \multicolumn{1}{c}{[0,18]} & \multicolumn{1}{c}{[19,34]} & \multicolumn{1}{c}{[35,65]} & \multicolumn{1}{c|}{65+} \\
        \specialrule{1.2pt}{0.2pt}{1pt}  
        \multirow{2}{*}{Airport-1} & A5 &0.11 & 0.70 & 0.20 & - & 0.0077$\pm$0.0042 \\ 
        & A6 &0.00 & 0.46 & 0.33 & - & 0.0306$\pm$0.0272 \\ \hline 
        \multirow{2}{*}{Airport-2} & A5 &0.34 & 0.66 & 0.32 & - & 0.0104$\pm$0.0086 \\ 
        & A6 &0.00 & 0.32 & 0.25 & 0.00 & 0.0414$\pm$0.0402 \\ \hline 
        \multirow{2}{*}{Airport-3} & A5 &0.20 & 0.79 & 0.15 & 0.02 & 0.0076$\pm$0.0040 \\ 
        & A6 &0.05 & 0.56 & 0.30 & - & 0.0305$\pm$0.0263 \\ \hline 
        \multirow{2}{*}{Airport-4} & A5 &0.05 & 0.75 & 0.31 & 0.00 & 0.0096$\pm$0.0068 \\ 
        & A6 &0.01 & 0.38 & 0.43 & - & 0.0414$\pm$0.0331 \\ \hline \hline 
        \multirow{2}{*}{Mall-1} & A5 &- & 0.39 & 0.39 & 0.03 & 0.0126$\pm$0.0099 \\ 
        & A6 &- & 0.51 & 0.77 & - & 0.0531$\pm$0.0466 \\ \hline 
        \multirow{2}{*}{Mall-2} & A5 &0.03 & 0.28 & 0.64 & - & 0.0309$\pm$0.0124 \\ 
        & A6 &0.03 & 0.44 & 0.70 & - & 0.3868$\pm$0.1909 \\ \hline 
        \multirow{2}{*}{Mall-3} & A5 &0.28 & 0.59 & 0.31 & - & 0.0194$\pm$0.0121 \\ 
        & A6 &0.01 & 0.40 & 0.60 & 0.02 & 0.1279$\pm$0.0642 \\ \hline 
        \multirow{2}{*}{Mall-4} & A5 &0.07 & 0.42 & 0.28 & - & 0.0271$\pm$0.0116 \\ 
        & A6 &- & 0.48 & 0.66 & 0.02 & 0.1419$\pm$0.0690 \\ \hline \hline 
        \multirow{2}{*}{Pedestrian-1} & A5 &0.07 & 0.74 & 0.36 & 0.01 & 0.0080$\pm$0.0056 \\ 
        & A6 &0.05 & 0.32 & 0.36 & - & 0.0298$\pm$0.0352 \\ \hline 
        \multirow{2}{*}{Pedestrian-2} & A5 &0.16 & 0.55 & 0.46 & 0.13 & 0.0093$\pm$0.0070 \\ 
        & A6 &- & 0.40 & 0.38 & 0.00 & 0.0401$\pm$0.0322 \\ \hline 
        \multirow{2}{*}{Pedestrian-3} & A5 &0.07 & 0.66 & 0.62 & 0.03 & 0.0234$\pm$0.0125 \\ 
        & A6 &- & 0.37 & 0.51 & - & 0.1008$\pm$0.0536 \\ \hline 
        \multirow{2}{*}{Pedestrian-4} & A5 &0.18 & 0.40 & 0.37 & 0.02 & 0.0234$\pm$0.0127 \\ 
        & A6 &- & 0.40 & 0.58 & 0.02 & 0.0987$\pm$0.0630 \\ \hline 
        \multirow{2}{*}{Pedestrian-5} & A5 &0.05 & 0.76 & 0.78 & 0.01 & 0.0073$\pm$0.0056 \\ 
        & A6 &0.02 & 0.49 & 0.56 & - & 0.0287$\pm$0.0334 \\ \hline \hline 
        \multirow{2}{*}{Subway-1} & A5 &0.01 & 0.77 & 0.10 & 0.03 & 0.0175$\pm$0.0133 \\ 
        & A6 &- & 0.63 & 0.18 & - & 0.0674$\pm$0.0522 \\ \hline 
        \multirow{2}{*}{Subway-2} & A5 &0.05 & 0.74 & 0.38 & 0.03 & 0.0271$\pm$0.0122 \\ 
        & A6 &- & 0.64 & 0.33 & - & 0.1367$\pm$0.0918 \\ \hline 
        \multirow{2}{*}{Subway-3} & A5 &0.11 & 0.53 & 0.22 & 0.00 & 0.0212$\pm$0.0150 \\ 
        & A6 &0.00 & 0.64 & 0.66 & - & 0.0650$\pm$0.0366 \\ 
        \specialrule{1.2pt}{0.2pt}{1pt}
        \multirow{2}{*}{Overall} &A5 &0.12$\pm$0.09 &0.61$\pm$0.16 &0.37$\pm$0.18 &0.03$\pm$0.03 &0.0164$\pm$0.0080 \\ 
        & A6 &0.02$\pm$0.02 &0.47$\pm$0.10 &0.47$\pm$0.17 &0.02$\pm$0.01 &0.0888$\pm$0.0861 \\ 
        \specialrule{1.2pt}{0.2pt}{1pt}
    \end{tabular}
        %}%
\end{table}
%=====================

% SYSTEM 1 - CPU
%=====================
\begin{table}[!t]
    \centering
    \footnotesize
    \setlength{\tabcolsep}{1pt}
    \caption{Age estimation results per video running algorithms in \textbf{System 1} with \textbf{CPU}. KEY -- Ax: algorithm x; F: F1-Score.}
    \label{tab:age_results_S1cpu}
    %\resizebox{\columnwidth}{!}{
        \begin{tabular}{lc|cccc|c}
        \specialrule{1.2pt}{0.2pt}{1pt}
        \multicolumn{1}{c}{\multirow{2}{*}{Video}} & \multicolumn{1}{c|}{\multirow{2}{*}{Alg.}} & \multicolumn{4}{c|}{F1-Score} &
        \multicolumn{1}{|c}{\multirow{2}{*}{\begin{tabular}[c]{@{}c@{}}Speed\\ {[}seconds/frame{]}\end{tabular}}} \\
         &  & \multicolumn{1}{c}{[0,18]} & \multicolumn{1}{c}{[19,34]} & \multicolumn{1}{c}{[35,65]} & \multicolumn{1}{c|}{65+} \\
        \specialrule{1.2pt}{0.2pt}{1pt}
        \multirow{2}{*}{Airport-1}   & A5 &0.10 & 0.70 & 0.21 & - & 0.1638$\pm$0.0392 \\ 
        & A6 &0.00 & 0.46 & 0.32 & - & 1.2388$\pm$0.4503 \\ \hline 
        \multirow{2}{*}{Airport-2}   & A5 &0.20 & 0.59 & 0.23 & - & 0.1363$\pm$0.0739 \\ 
        & A6 &0.03 & 0.37 & 0.23 & - & 1.0245$\pm$0.6295 \\ \hline 
        \multirow{2}{*}{Airport-3}   & A5 &0.19 & 0.78 & 0.16 & 0.02 & 0.1410$\pm$0.0658 \\ 
        & A6 &0.05 & 0.55 & 0.31 & - & 1.1198$\pm$0.6068 \\ \hline 
        \multirow{2}{*}{Airport-4}   & A5 &0.05 & 0.75 & 0.34 & 0.00 & 0.1719$\pm$0.0369 \\ 
        & A6 &0.01 & 0.38 & 0.44 & - & 1.3792$\pm$0.5134 \\ \hline \hline 
        \multirow{2}{*}{Mall-1}   & A5 &- & 0.37 & 0.38 & 0.02 & 0.1737$\pm$0.0174 \\ 
        & A6 &- & 0.50 & 0.78 & - & 2.0464$\pm$0.7904 \\ \hline 
        \multirow{2}{*}{Mall-2} & A5 &0.01 & 0.36 & 0.43 & 0.01 & 0.1769$\pm$0.0145 \\ 
        & A6 &0.06 & 0.53 & 0.72 & - & 2.6070$\pm$1.1557 \\ \hline 
        \multirow{2}{*}{Mall-3} & A5 &0.12 & 0.56 & 0.22 & 0.00 & 0.1615$\pm$0.0431 \\ 
        & A6 &0.02 & 0.46 & 0.57 & - & 1.3027$\pm$0.5113 \\ \hline 
        \multirow{2}{*}{Mall-4} & A5 &0.02 & 0.49 & 0.27 & - & 0.1600$\pm$0.0463 \\ 
        & A6 &- & 0.51 & 0.60 & - & 1.2904$\pm$0.5385 \\ \hline \hline 
        \multirow{2}{*}{Pedestrian-1} & A5 &0.07 & 0.72 & 0.37 & 0.01 & 0.1701$\pm$0.0255 \\ 
        & A6 &0.04 & 0.34 & 0.40 & - & 1.5363$\pm$0.5966 \\ \hline 
        \multirow{2}{*}{Pedestrian-2} & A5 &0.14 & 0.55 & 0.46 & 0.12 & 0.1597$\pm$0.0487 \\ 
        & A6 &- & 0.40 & 0.40 & 0.00 & 1.6718$\pm$0.7984 \\ \hline 
        \multirow{2}{*}{Pedestrian-3} & A5 &0.01 & 0.71 & 0.64 & 0.14 & 0.1659$\pm$0.0368 \\ 
        & A6 &- & 0.50 & 0.47 & - & 1.6515$\pm$0.6932 \\ \hline 
        \multirow{2}{*}{Pedestrian-4} & A5 &0.07 & 0.38 & 0.35 & 0.05 & 0.1667$\pm$0.0317 \\ 
        & A6 &- & 0.47 & 0.58 & 0.01 & 1.6602$\pm$0.6433 \\ \hline 
        \multirow{2}{*}{Pedestrian-5} & A5 &0.04 & 0.77 & 0.78 & 0.01 & 0.1685$\pm$0.0287 \\ 
        & A6 &0.01 & 0.48 & 0.56 & - & 1.5458$\pm$0.5273 \\ \hline \hline 
        \multirow{2}{*}{Subway-1} & A5 &0.01 & 0.77 & 0.14 & 0.03 & 0.1524$\pm$0.0582 \\ 
        & A6 &- & 0.62 & 0.18 & - & 1.8670$\pm$1.0221 \\ \hline 
        \multirow{2}{*}{Subway-2} & A5 &0.00 & 0.78 & 0.06 & 0.09 & 0.1695$\pm$0.0381 \\ 
        & A6 &- & 0.68 & 0.19 & - & 1.9276$\pm$0.7464 \\ \hline 
        \multirow{2}{*}{Subway-3} & A5 &0.10 & 0.53 & 0.28 & 0.00 & 0.1684$\pm$0.0359 \\ 
        & A6 &0.00 & 0.64 & 0.67 & - & 1.9310$\pm$0.7390 \\ 
        \specialrule{1.2pt}{0.2pt}{1pt}
        \multirow{2}{*}{Overall} &A5 &0.08$\pm$0.06 &0.61$\pm$0.15 &0.33$\pm$0.18 &0.04$\pm$0.05 &0.1629$\pm$0.0109 \\ 
        & A6 &0.03$\pm$0.02 &0.49$\pm$0.09 &0.46$\pm$0.18 &0.01$\pm$0.01 &1.6125$\pm$0.3907 \\
        \specialrule{1.2pt}{0.2pt}{1pt}
        \end{tabular}
        %}%
\end{table}
%=====================

% SYSTEM 2 - GPU
%=====================
\begin{table}[!t]
    \centering
    \footnotesize
    \setlength{\tabcolsep}{1pt}
    \caption{Age estimation results per video running algorithms in \textbf{System 2} with \textbf{GPU}. KEY -- Ax: algorithm x; F: F1-Score.}
    \label{tab:age_results_S2gpu}
    %\resizebox{\columnwidth}{!}{
        \begin{tabular}{lc|cccc|c}
        \specialrule{1.2pt}{0.2pt}{1pt}
        \multicolumn{1}{c}{\multirow{2}{*}{Video}} & \multicolumn{1}{c|}{\multirow{2}{*}{Alg.}} & \multicolumn{4}{c|}{F1-Score} &
        \multicolumn{1}{|c}{\multirow{2}{*}{\begin{tabular}[c]{@{}c@{}}Speed\\ {[}seconds/frame{]}\end{tabular}}} \\
         &  & \multicolumn{1}{c}{[0,18]} & \multicolumn{1}{c}{[19,34]} & \multicolumn{1}{c}{[35,65]} & \multicolumn{1}{c|}{65+} \\
        \specialrule{1.2pt}{0.2pt}{1pt}
        \multirow{2}{*}{Airport-1}   & A5 &0.33 & 0.70 & 0.32 & - & 0.0083$\pm$0.0021 \\ 
        & A6 &- & 0.55 & 0.33 & - & 0.0389$\pm$0.0246 \\ \hline 
        \multirow{2}{*}{Airport-2}   & A5 &0.34 & 0.66 & 0.32 & - & 0.0077$\pm$0.0027 \\ 
        & A6 &0.00 & 0.32 & 0.25 & 0.00 & 0.0369$\pm$0.0301 \\ \hline 
        \multirow{2}{*}{Airport-3}   & A5 &0.26 & 0.75 & 0.19 & - & 0.0082$\pm$0.0022 \\ 
        & A6 &0.05 & 0.54 & 0.34 & 0.00 & 0.0314$\pm$0.0196 \\ \hline 
        \multirow{2}{*}{Airport-4}   & A5 &0.14 & 0.75 & 0.44 & - & 0.0089$\pm$0.0016 \\ 
        & A6 &0.01 & 0.35 & 0.44 & - & 0.0644$\pm$0.0333 \\ \hline \hline 
        \multirow{2}{*}{Mall-1}   & A5 &- & 0.39 & 0.53 & 0.00 & 0.0121$\pm$0.0032 \\ 
        & A6 &- & 0.30 & 0.78 & - & 0.3342$\pm$0.1210 \\ \hline 
        \multirow{2}{*}{Mall-2} & A5 &0.03 & 0.28 & 0.64 & - & 0.0128$\pm$0.0042 \\ 
        & A6 &0.03 & 0.44 & 0.70 & - & 0.3672$\pm$0.1664 \\ \hline 
        \multirow{2}{*}{Mall-3} & A5 &0.28 & 0.59 & 0.31 & - & 0.0096$\pm$0.0018 \\ 
        & A6 &0.01 & 0.40 & 0.60 & 0.02 & 0.1202$\pm$0.0450 \\ \hline 
        \multirow{2}{*}{Mall-4} & A5 &0.07 & 0.42 & 0.28 & - & 0.0097$\pm$0.0018 \\ 
        & A6 &- & 0.48 & 0.66 & 0.02 & 0.1325$\pm$0.0517 \\ \hline \hline 
        \multirow{2}{*}{Pedestrian-1} & A5 &0.11 & 0.70 & 0.44 & - & 0.0098$\pm$0.0018 \\ 
        & A6 &- & 0.38 & 0.41 & - & 0.1318$\pm$0.0540 \\ \hline 
        \multirow{2}{*}{Pedestrian-2} & A5 &0.26 & 0.50 & 0.40 & 0.02 & 0.0102$\pm$0.0020 \\ 
        & A6 &- & 0.34 & 0.48 & 0.13 & 0.1435$\pm$0.0677 \\ \hline 
        \multirow{2}{*}{Pedestrian-3} & A5 &0.07 & 0.66 & 0.62 & 0.03 & 0.0094$\pm$0.0015 \\ 
        & A6 &- & 0.37 & 0.51 & - & 0.0910$\pm$0.0381 \\ \hline 
        \multirow{2}{*}{Pedestrian-4} & A5 &0.18 & 0.40 & 0.37 & 0.02 & 0.0092$\pm$0.0018 \\ 
        & A6 &- & 0.40 & 0.58 & 0.02 & 0.0875$\pm$0.0444 \\ \hline 
        \multirow{2}{*}{Pedestrian-5} & A5 &0.02 & 0.65 & 0.74 & - & 0.0092$\pm$0.0020 \\ 
        & A6 &- & 0.44 & 0.51 & - & 0.0886$\pm$0.0460 \\ \hline \hline 
        \multirow{2}{*}{Subway-1} & A5 &0.04 & 0.76 & 0.27 & 0.01 & 0.0094$\pm$0.0020 \\ 
        & A6 &- & 0.59 & 0.17 & - & 0.0928$\pm$0.0501 \\ \hline 
        \multirow{2}{*}{Subway-2} & A5 &0.05 & 0.74 & 0.38 & 0.03 & 0.0100$\pm$0.0025 \\ 
        & A6 &- & 0.64 & 0.33 & - & 0.1262$\pm$0.0623 \\ \hline 
        \multirow{2}{*}{Subway-3} & A5 &0.20 & 0.55 & 0.11 & - & 0.0093$\pm$0.0020 \\ 
        & A6 &- & 0.67 & 0.66 & - & 0.0953$\pm$0.0503 \\ 
        \specialrule{1.2pt}{0.2pt}{1pt}
        \multirow{2}{*}{Overall} & A5 &0.16$\pm$0.11 &0.59$\pm$0.15 &0.40$\pm$0.16 &0.02$\pm$0.01 &0.0096$\pm$0.0013 \\ 
         & A6 &0.02$\pm$0.02 &0.45$\pm$0.11 &0.48$\pm$0.17 &0.03$\pm$0.05 &0.1239$\pm$0.0923 \\ 
        \specialrule{1.2pt}{0.2pt}{1pt}
        \end{tabular}
        %}%
\end{table}
%=====================

% SYSTEM 2 - CPU
%=====================
\begin{table}[!t]
    \centering
    \footnotesize
    \setlength{\tabcolsep}{1pt}
    \caption{Age estimation results per video running algorithms in \textbf{System 2} with \textbf{CPU}. KEY -- Ax: algorithm x; F: F1-Score.}
    \label{tab:age_results_S2cpu}
    %\resizebox{\columnwidth}{!}{
        \begin{tabular}{lc|cccc|c}
        \specialrule{1.2pt}{0.2pt}{1pt}
        \multicolumn{1}{c}{\multirow{2}{*}{Video}} & \multicolumn{1}{c|}{\multirow{2}{*}{Alg.}} & \multicolumn{4}{c|}{F1-Score} &
        \multicolumn{1}{|c}{\multirow{2}{*}{\begin{tabular}[c]{@{}c@{}}Speed\\ {[}seconds/frame{]}\end{tabular}}} \\
         &  & \multicolumn{1}{c}{[0,18]} & \multicolumn{1}{c}{[19,34]} & \multicolumn{1}{c}{[35,65]} & \multicolumn{1}{c|}{65+} \\
        \specialrule{1.2pt}{0.2pt}{1pt}
        \multirow{2}{*}{Airport-1}   & A5 &0.33 & 0.70 & 0.31 & - & 0.0149$\pm$0.0045 \\ 
        & A6 &- & 0.56 & 0.33 & - & 0.3990$\pm$0.2348 \\ \hline 
        \multirow{2}{*}{Airport-2}   & A5 &0.36 & 0.66 & 0.30 & - & 0.0140$\pm$0.0060 \\ 
        & A6 &- & 0.31 & 0.24 & - & 0.3745$\pm$0.2805 \\ \hline 
        \multirow{2}{*}{Airport-3}   & A5 &0.28 & 0.75 & 0.19 & - & 0.0138$\pm$0.0045 \\ 
        & A6 &0.05 & 0.54 & 0.34 & 0.01 & 0.3248$\pm$0.1970 \\ \hline 
        \multirow{2}{*}{Airport-4}   & A5 &0.18 & 0.75 & 0.42 & - & 0.0185$\pm$0.0038 \\ 
        & A6 &0.02 & 0.35 & 0.43 & - & 0.6903$\pm$0.3353 \\ \hline \hline 
        \multirow{2}{*}{Mall-1}   & A5 &- & 0.39 & 0.54 & 0.00 & 0.0485$\pm$0.0079 \\ 
        & A6 &- & 0.30 & 0.78 & - & 4.5413$\pm$0.9187 \\ \hline 
        \multirow{2}{*}{Mall-2} & A5 &0.02 & 0.28 & 0.63 & - & 0.0519$\pm$0.0092 \\ 
        & A6 &0.03 & 0.45 & 0.70 & - & 4.9023$\pm$1.1083 \\ \hline 
        \multirow{2}{*}{Mall-3} & A5 &0.25 & 0.58 & 0.31 & - & 0.0248$\pm$0.0039 \\ 
        & A6 &0.01 & 0.41 & 0.60 & 0.02 & 1.3990$\pm$0.4074 \\ \hline 
        \multirow{2}{*}{Mall-4} & A5 &0.06 & 0.42 & 0.29 & - & 0.0262$\pm$0.0046 \\ 
        & A6 &- & 0.48 & 0.66 & 0.03 & 1.5869$\pm$0.4928 \\ \hline \hline 
        \multirow{2}{*}{Pedestrian-1} & A5 &0.11 & 0.70 & 0.45 & - & 0.0262$\pm$0.0049 \\ 
        & A6 &- & 0.36 & 0.41 & - & 1.5863$\pm$0.5587 \\ \hline 
        \multirow{2}{*}{Pedestrian-2} & A5 &0.26 & 0.50 & 0.41 & 0.02 & 0.0278$\pm$0.0059 \\ 
        & A6 &- & 0.32 & 0.48 & 0.13 & 1.7533$\pm$0.6561 \\ \hline 
        \multirow{2}{*}{Pedestrian-3} & A5 &0.07 & 0.66 & 0.63 & 0.03 & 0.0214$\pm$0.0036 \\ 
        & A6 &- & 0.35 & 0.50 & - & 0.9879$\pm$0.3604 \\ \hline 
        \multirow{2}{*}{Pedestrian-4} & A5 &0.16 & 0.39 & 0.36 & 0.01 & 0.0205$\pm$0.0038 \\ 
        & A6 &- & 0.40 & 0.58 & 0.02 & 0.9375$\pm$0.3629 \\ \hline 
        \multirow{2}{*}{Pedestrian-5} & A5 &0.03 & 0.66 & 0.75 & - & 0.0209$\pm$0.0041 \\ 
        & A6 &- & 0.45 & 0.50 & - & 0.9538$\pm$0.3963 \\ \hline \hline 
        \multirow{2}{*}{Subway-1} & A5 &0.04 & 0.76 & 0.27 & 0.02 & 0.0218$\pm$0.0052 \\ 
        & A6 &- & 0.59 & 0.18 & - & 1.0687$\pm$0.5277 \\ \hline 
        \multirow{2}{*}{Subway-2} & A5 &0.05 & 0.74 & 0.39 & 0.02 & 0.0256$\pm$0.0053 \\ 
        & A6 &- & 0.63 & 0.33 & - & 1.5076$\pm$0.5511 \\ \hline 
        \multirow{2}{*}{Subway-3} & A5 &0.20 & 0.55 & 0.10 & - & 0.0218$\pm$0.0055 \\ 
        & A6 &- & 0.68 & 0.66 & - & 1.0611$\pm$0.4969 \\ 
        \specialrule{1.2pt}{0.2pt}{1pt}
        \multirow{2}{*}{Overall} &A5 &0.16$\pm$0.11 &0.59$\pm$0.15 &0.40$\pm$0.17 &0.02$\pm$0.01 &0.0249$\pm$0.0105 \\ 
        & A6 &0.03$\pm$0.02 &0.45$\pm$0.12 &0.48$\pm$0.17 &0.04$\pm$0.05 &1.5046$\pm$1.2915 \\ 
        \specialrule{1.2pt}{0.2pt}{1pt}
        \end{tabular}
        %}%
\end{table}
%=====================

% SYSTEM 3 - GPU
%=====================
\begin{table}[!t]
    \centering
    \footnotesize
    \setlength{\tabcolsep}{1pt}
    \caption{Age estimation results per video running algorithms in \textbf{System 3} with \textbf{GPU}. KEY -- Ax: algorithm x; F: F1-Score.}
    \label{tab:age_results_S3}
    %\resizebox{\columnwidth}{!}{
        \begin{tabular}{lc|cccc|c}
        \specialrule{1.2pt}{0.2pt}{1pt}
        \multicolumn{1}{c}{\multirow{2}{*}{Video}} & \multicolumn{1}{c|}{\multirow{2}{*}{Alg.}} & \multicolumn{4}{c|}{F1-Score} &
        \multicolumn{1}{|c}{\multirow{2}{*}{\begin{tabular}[c]{@{}c@{}}Speed\\ {[}seconds/frame{]}\end{tabular}}} \\
         &  & \multicolumn{1}{c}{[0,18]} & \multicolumn{1}{c}{[19,34]} & \multicolumn{1}{c}{[35,65]} & \multicolumn{1}{c|}{65+} \\
        \specialrule{1.2pt}{0.2pt}{1pt}
        \multirow{2}{*}{Airport-1}   & A5 &0.10 & 0.70 & 0.20 & - & 0.3712$\pm$0.0888 \\ 
        & A6 &0.02 & 0.47 & 0.32 & - & 6.2763$\pm$3.0372 \\ \hline 
        \multirow{2}{*}{Airport-2}   & A5 &0.22 & 0.59 & 0.21 & - & 0.2993$\pm$0.1638 \\ 
        & A6 &0.02 & 0.39 & 0.23 & - & 4.8429$\pm$3.4963 \\ \hline 
        \multirow{2}{*}{Airport-3}   & A5 &0.24 & 0.79 & 0.17 & 0.01 & 0.3171$\pm$0.1477 \\ 
        & A6 &0.04 & 0.55 & 0.30 & - & 4.8207$\pm$3.0917 \\ \hline 
        \multirow{2}{*}{Airport-4}   & A5 &0.03 & 0.75 & 0.33 & - & 0.3824$\pm$0.0867 \\ 
        & A6 &0.02 & 0.39 & 0.43 & - & 7.4845$\pm$3.7042 \\ \hline \hline 
        \multirow{2}{*}{Mall-1}   & A5 &- & 0.37 & 0.38 & 0.04 & 0.4311$\pm$0.0587 \\ 
        & A6 &- & 0.51 & 0.78 & - & 13.0439$\pm$6.2004 \\ \hline 
        \multirow{2}{*}{Mall-2} & A5 &0.01 & 0.35 & 0.43 & - & 0.4638$\pm$0.0694 \\ 
        & A6 &0.05 & 0.52 & 0.72 & - & 17.5045$\pm$9.0727 \\ \hline 
        \multirow{2}{*}{Mall-3} & A5 &0.11 & 0.57 & 0.24 & - & 0.3664$\pm$0.1072 \\ 
        & A6 &0.02 & 0.45 & 0.56 & - & 6.8693$\pm$3.5238 \\ \hline 
        \multirow{2}{*}{Mall-4} & A5 &0.04 & 0.48 & 0.28 & - & 0.3676$\pm$0.1051 \\ 
        & A6 &- & 0.52 & 0.60 & - & 6.8015$\pm$3.5475 \\ \hline \hline 
        \multirow{2}{*}{Pedestrian-1} & A5 &0.09 & 0.72 & 0.40 & - & 0.3981$\pm$0.0635 \\ 
        & A6 &0.03 & 0.37 & 0.41 & - & 8.4344$\pm$4.5305 \\ \hline 
        \multirow{2}{*}{Pedestrian-2} & A5 &0.15 & 0.54 & 0.47 & 0.14 & 0.3827$\pm$0.1205 \\ 
        & A6 &- & 0.40 & 0.40 & 0.01 & 9.0186$\pm$5.3816 \\ \hline 
        \multirow{2}{*}{Pedestrian-3} & A5 &0.03 & 0.70 & 0.62 & 0.15 & 0.3941$\pm$0.0871 \\ 
        & A6 &- & 0.49 & 0.48 & - & 9.0293$\pm$5.0491 \\ \hline 
        \multirow{2}{*}{Pedestrian-4} & A5 &0.04 & 0.38 & 0.35 & 0.05 & 0.3958$\pm$0.0800 \\ 
        & A6 &- & 0.47 & 0.58 & 0.02 & 8.5377$\pm$4.7048 \\ \hline 
        \multirow{2}{*}{Pedestrian-5} & A5 &0.05 & 0.77 & 0.77 & - & 0.3970$\pm$0.0677 \\ 
        & A6 &- & 0.46 & 0.55 & - & 8.7285$\pm$3.7757 \\ \hline \hline 
        \multirow{2}{*}{Subway-1} & A5 &- & 0.77 & 0.13 & 0.03 & 0.3838$\pm$0.1510 \\ 
        & A6 &- & 0.62 & 0.17 & - & 11.8167$\pm$7.1642 \\ \hline 
        \multirow{2}{*}{Subway-2} & A5 &- & 0.78 & 0.05 & 0.12 & 0.4104$\pm$0.0993 \\ 
        & A6 &- & 0.69 & 0.18 & - & 11.8930$\pm$5.1045 \\ \hline 
        \multirow{2}{*}{Subway-3} & A5 &0.09 & 0.53 & 0.28 & - & 0.4132$\pm$0.0934 \\ 
        & A6 &- & 0.64 & 0.68 & - & 12.1132$\pm$5.1922 \\ 
        \specialrule{1.2pt}{0.2pt}{1pt}
        \multirow{2}{*}{Overall} &A5 &0.09$\pm$0.07 &0.61$\pm$0.15 &0.33$\pm$0.18 &0.08$\pm$0.05 &0.3859$\pm$0.0380 \\ 
        & A6 &0.03$\pm$0.01 &0.50$\pm$0.09 &0.46$\pm$0.18 &0.01$\pm$0.00 &9.2009$\pm$3.2449 \\ 
        \specialrule{1.2pt}{0.2pt}{1pt}
        \end{tabular}
        %}%
\end{table}
%=====================

% SYSTEM 4 - GPU
%=====================
\begin{table}[!t]
    \centering
    \footnotesize
    \setlength{\tabcolsep}{1pt}
    \caption{Age estimation results per video running algorithms in \textbf{System 4} with \textbf{GPU}. KEY -- Ax: algorithm x; F: F1-Score. Note that A6 cannot run in System 4 due to lack of memory.}
    \label{tab:age_results_S4}
    %\resizebox{\columnwidth}{!}{
        \begin{tabular}{lc|cccc|c}
        \specialrule{1.2pt}{0.2pt}{1pt}
        \multicolumn{1}{c}{\multirow{2}{*}{Video}} & \multicolumn{1}{c|}{\multirow{2}{*}{Alg.}} & \multicolumn{4}{c|}{F1-Score} &
        \multicolumn{1}{|c}{\multirow{2}{*}{\begin{tabular}[c]{@{}c@{}}Speed\\ {[}seconds/frame{]}\end{tabular}}} \\
         &  & \multicolumn{1}{c}{[0,18]} & \multicolumn{1}{c}{[19,34]} & \multicolumn{1}{c}{[35,65]} & \multicolumn{1}{c|}{65+} \\
        \specialrule{1.2pt}{0.2pt}{1pt}
        \multirow{1}{*}{Airport-1}   & A5 &0.31 & 0.70 & 0.31 & - & 0.0722$\pm$0.3782 \\  
        \multirow{1}{*}{Airport-2} & A5 &0.35 & 0.66 & 0.32 & - & 0.0675$\pm$0.4078 \\  
        \multirow{1}{*}{Airport-3} & A5 &0.29 & 0.76 & 0.19 & - & 0.0695$\pm$0.4311 \\  
        \multirow{1}{*}{Airport-4} & A5 &0.18 & 0.74 & 0.42 & - & 0.0809$\pm$0.4252 \\ \hline \hline 
        \multirow{1}{*}{Mall-1} & A5 &- & 0.40 & 0.54 & 0.00 & 0.1772$\pm$0.4627 \\  
        \multirow{1}{*}{Mall-2} & A5 &0.02 & 0.28 & 0.63 & - & 0.2085$\pm$0.5110 \\  
        \multirow{1}{*}{Mall-3} & A5 &0.26 & 0.59 & 0.31 & - & 0.0958$\pm$0.5587 \\  
        \multirow{1}{*}{Mall-4} & A5 &0.06 & 0.42 & 0.29 & - & 0.0915$\pm$0.4238 \\ \hline \hline 
        \multirow{1}{*}{Pedestrian-1} & A5 &0.11 & 0.70 & 0.43 & - & 0.0907$\pm$0.4169 \\  
        \multirow{1}{*}{Pedestrian-2} & A5 &0.24 & 0.51 & 0.40 & 0.02 & 0.1007$\pm$0.4440 \\  
        \multirow{1}{*}{Pedestrian-3} & A5 &0.06 & 0.66 & 0.64 & 0.04 & 0.0824$\pm$0.4130 \\  
        \multirow{1}{*}{Pedestrian-4} & A5 &0.16 & 0.40 & 0.35 & 0.01 & 0.0874$\pm$0.4827 \\  
        \multirow{1}{*}{Pedestrian-5} & A5 &0.02 & 0.65 & 0.75 & - & 0.0977$\pm$0.5495 \\ \hline \hline 
        \multirow{1}{*}{Subway-1} & A5 &0.03 & 0.76 & 0.26 & 0.02 & 0.0949$\pm$0.4157 \\  
        \multirow{1}{*}{Subway-2} & A5 &0.05 & 0.74 & 0.39 & 0.01 & 0.1135$\pm$0.5004 \\  
        \multirow{1}{*}{Subway-3} & A5 &0.19 & 0.55 & 0.11 & 0.01 & 0.0850$\pm$0.4085 \\  
        \specialrule{1.2pt}{0.2pt}{1pt}
        \multirow{1}{*}{Overall} &A5 &0.15$\pm$0.11 &0.59$\pm$0.15 &0.40$\pm$0.16 &0.02$\pm$0.01 &0.1010$\pm$0.0370 \\ 
        \specialrule{1.2pt}{0.2pt}{1pt}
        \end{tabular}
        %}%
\end{table}
%=====================

\section*{Appendix D: Gender estimation results per video}

Gender estimation results per video in
System 1-GPU in Table~\ref{tab:gender_results_S1gpu},
System 1-CPU in Table~\ref{tab:gender_results_S1cpu},
System 2-GPU in Table~\ref{tab:gender_results_S2gpu},
System 2-CPU in Table~\ref{tab:gender_results_S2cpu},
System 3 in Table~\ref{tab:gender_results_S3}, and
System 4 in Table~\ref{tab:gender_results_S4}.

% SYSTEM 1 - GPU
%=====================
\begin{table}[!t]
    \centering
    \footnotesize
    \setlength{\tabcolsep}{1pt}
    \caption{Gender estimation results per video running algorithms in \textbf{System 1} with \textbf{GPU}. KEY -- Ax: algorithm x; F: F1-Score.}
    \label{tab:gender_results_S1gpu}
    %\resizebox{\columnwidth}{!}{
        \begin{tabular}{lc|cc|c}
        \specialrule{1.2pt}{0.2pt}{1pt}
        \multicolumn{1}{c}{\multirow{2}{*}{Video}} & \multicolumn{1}{c|}{\multirow{2}{*}{Alg.}} & \multicolumn{2}{c|}{F1-Score} &
        \multicolumn{1}{|c}{\multirow{2}{*}{\begin{tabular}[c]{@{}c@{}}Speed\\ {[}seconds/frame{]}\end{tabular}}} \\
         &  & \multicolumn{1}{c}{Male} & \multicolumn{1}{c|}{Female} \\
        \specialrule{1.2pt}{0.2pt}{1pt}
        \multirow{2}{*}{Airport-1} & A5 &0.79 &0.79 &0.0077$\pm$0.0042 \\ 
        & A6 &0.64 &0.68 &0.0306$\pm$0.0272 \\ \hline 
        \multirow{2}{*}{Airport-2} & A5 &0.62 &0.75 &0.0104$\pm$0.0086 \\ 
        & A6 &0.48 &0.49 &0.0414$\pm$0.0402 \\ \hline 
        \multirow{2}{*}{Airport-3} & A5 &0.72 &0.76 &0.0076$\pm$0.0040 \\ 
        & A6 &0.60 &0.67 &0.0305$\pm$0.0263 \\ \hline 
        \multirow{2}{*}{Airport-4} & A5 &0.69 &0.65 &0.0096$\pm$0.0068 \\ 
        & A6 &0.58 &0.63 &0.0414$\pm$0.0331 \\ \hline \hline 
        \multirow{2}{*}{Mall-1} & A5 &0.76 &0.71 &0.0126$\pm$0.0099 \\ 
        & A6 &0.63 &0.71 &0.0531$\pm$0.0466 \\ \hline 
        \multirow{2}{*}{Mall-2} & A5 &0.78 &0.41 &0.0309$\pm$0.0124 \\ 
        & A6 &0.71 &0.34 &0.3868$\pm$0.1909 \\ \hline 
        \multirow{2}{*}{Mall-3} & A5 &0.58 &0.51 &0.0194$\pm$0.0121 \\ 
        & A6 &0.57 &0.43 &0.1279$\pm$0.0642 \\ \hline 
        \multirow{2}{*}{Mall-4} & A5 &0.47 &0.32 &0.0271$\pm$0.0116 \\ 
        & A6 &0.45 &0.23 &0.1419$\pm$0.0690 \\ \hline \hline 
        \multirow{2}{*}{Pedestrian-1} & A5 &0.59 &0.83 &0.0080$\pm$0.0056 \\ 
        & A6 &0.55 &0.85 &0.0298$\pm$0.0352 \\ \hline 
        \multirow{2}{*}{Pedestrian-2} & A5 &0.76 &0.65 &0.0093$\pm$0.0070 \\ 
        & A6 &0.67 &0.60 &0.0401$\pm$0.0322 \\ \hline 
        \multirow{2}{*}{Pedestrian-3} & A5 &0.54 &0.48 &0.0234$\pm$0.0125 \\ 
        & A6 &0.49 &0.20 &0.1008$\pm$0.0536 \\ \hline 
        \multirow{2}{*}{Pedestrian-4} & A5 &0.76 &0.59 &0.0234$\pm$0.0127 \\ 
        & A6 &0.70 &0.26 &0.0987$\pm$0.0630 \\ \hline 
        \multirow{2}{*}{Pedestrian-5} & A5 &0.50 &0.45 &0.0073$\pm$0.0056 \\ 
        & A6 &0.62 &0.74 &0.0287$\pm$0.0334 \\ \hline \hline 
        \multirow{2}{*}{Subway-1} & A5 &0.66 &0.62 &0.0175$\pm$0.0133 \\ 
        & A6 &0.62 &0.63 &0.0674$\pm$0.0522 \\ \hline 
        \multirow{2}{*}{Subway-2} & A5 &0.51 &0.55 &0.0271$\pm$0.0122 \\ 
        & A6 &0.45 &0.29 &0.1367$\pm$0.0918 \\ \hline 
        \multirow{2}{*}{Subway-3} & A5 &0.64 &0.46 &0.0212$\pm$0.0150 \\ 
        & A6 &0.79 &0.53 &0.0650$\pm$0.0366 \\ 
        \specialrule{1.2pt}{0.2pt}{1pt}
        \multirow{2}{*}{Overall} &A5 &0.65$\pm$0.11 &0.60$\pm$0.14 &0.0164$\pm$0.0080 \\ 
        &A6 &0.60$\pm$0.09 &0.52$\pm$0.20 &0.0888$\pm$0.0861 \\ 
        \specialrule{1.2pt}{0.2pt}{1pt}
        \end{tabular}
        %}%
\end{table}
%=====================

% SYSTEM 1 - CPU
%=====================
\begin{table}[!t]
    \centering
    \footnotesize
    \setlength{\tabcolsep}{1pt}
    \caption{Gender estimation results per video running algorithms in \textbf{System 1} with \textbf{CPU}. KEY -- Ax: algorithm x; F: F1-Score.}
    \label{tab:gender_results_S1cpu}
    %\resizebox{\columnwidth}{!}{
        \begin{tabular}{lc|cc|c}
        \specialrule{1.2pt}{0.2pt}{1pt}
        \multicolumn{1}{c}{\multirow{2}{*}{Video}} & \multicolumn{1}{c|}{\multirow{2}{*}{Alg.}} & \multicolumn{2}{c|}{F1-Score} &
        \multicolumn{1}{|c}{\multirow{2}{*}{\begin{tabular}[c]{@{}c@{}}Speed\\ {[}seconds/frame{]}\end{tabular}}} \\
         &  & \multicolumn{1}{c}{Male} & \multicolumn{1}{c|}{Female} \\
        \specialrule{1.2pt}{0.2pt}{1pt}
        \multirow{2}{*}{Airport-1} & A5 &0.79 &0.77 &0.1638$\pm$0.0392 \\ 
        & A6 &0.63 &0.66 &1.2388$\pm$0.4503 \\ \hline 
        \multirow{2}{*}{Airport-2} & A5 &0.75 &0.84 &0.1363$\pm$0.0739 \\ 
        & A6 &0.57 &0.75 &1.0245$\pm$0.6295 \\ \hline 
        \multirow{2}{*}{Airport-3} & A5 &0.72 &0.75 &0.1410$\pm$0.0658 \\ 
        & A6 &0.59 &0.66 &1.1198$\pm$0.6068 \\ \hline 
        \multirow{2}{*}{Airport-4} & A5 &0.69 &0.63 &0.1719$\pm$0.0369 \\ 
        & A6 &0.58 &0.63 &1.3792$\pm$0.5134 \\ \hline \hline 
        \multirow{2}{*}{Mall-1} & A5 &0.72 &0.65 &0.1737$\pm$0.0174 \\ 
        & A6 &0.58 &0.69 &2.0464$\pm$0.7904 \\ \hline 
        \multirow{2}{*}{Mall-2} & A5 &0.74 &0.64 &0.1769$\pm$0.0145 \\ 
        & A6 &0.55 &0.63 &2.6070$\pm$1.1557 \\ \hline 
        \multirow{2}{*}{Mall-3} & A5 &0.64 &0.77 &0.1615$\pm$0.0431 \\ 
        & A6 &0.51 &0.73 &1.3027$\pm$0.5113 \\ \hline 
        \multirow{2}{*}{Mall-4} & A5 &0.59 &0.67 &0.1600$\pm$0.0463 \\ 
        & A6 &0.47 &0.67 &1.2904$\pm$0.5385 \\ \hline \hline 
        \multirow{2}{*}{Pedestrian-1} & A5 &0.56 &0.79 &0.1701$\pm$0.0255 \\ 
        & A6 &0.53 &0.83 &1.5363$\pm$0.5966 \\ \hline 
        \multirow{2}{*}{Pedestrian-2} & A5 &0.77 &0.63 &0.1597$\pm$0.0487 \\ 
        & A6 &0.65 &0.57 &1.6718$\pm$0.7984 \\ \hline 
        \multirow{2}{*}{Pedestrian-3} & A5 &0.58 &0.56 &0.1659$\pm$0.0368 \\ 
        & A6 &0.52 &0.50 &1.6515$\pm$0.6932 \\ \hline 
        \multirow{2}{*}{Pedestrian-4} & A5 &0.80 &0.72 &0.1667$\pm$0.0317 \\ 
        & A6 &0.75 &0.60 &1.6602$\pm$0.6433 \\ \hline 
        \multirow{2}{*}{Pedestrian-5} & A5 &0.48 &0.40 &0.1685$\pm$0.0287 \\ 
        & A6 &0.60 &0.73 &1.5458$\pm$0.5273 \\ \hline \hline 
        \multirow{2}{*}{Subway-1} & A5 &0.63 &0.60 &0.1524$\pm$0.0582 \\ 
        & A6 &0.60 &0.63 &1.8670$\pm$1.0221 \\ \hline 
        \multirow{2}{*}{Subway-2} & A5 &0.58 &0.65 &0.1695$\pm$0.0381 \\ 
        & A6 &0.56 &0.67 &1.9276$\pm$0.7464 \\ \hline 
        \multirow{2}{*}{Subway-3} & A5 &0.64 &0.46 &0.1684$\pm$0.0359 \\ 
        & A6 &0.77 &0.52 &1.9310$\pm$0.7390 \\ 
        \specialrule{1.2pt}{0.2pt}{1pt}
        \multirow{2}{*}{Overall} &A5 &0.67$\pm$0.09 &0.66$\pm$0.11 &0.1629$\pm$0.0109 \\ 
        &A6 &0.59$\pm$0.08 &0.65$\pm$0.08 &1.6125$\pm$0.3907 \\ 
        \specialrule{1.2pt}{0.2pt}{1pt}
        \end{tabular}
        %}%
\end{table}
%=====================

% SYSTEM 2 - GPU
%=====================
\begin{table}[!t]
    \centering
    \footnotesize
    \setlength{\tabcolsep}{1pt}
    \caption{Gender estimation results per video running algorithms in \textbf{System 2} with \textbf{GPU}. KEY -- Ax: algorithm x; F: F1-Score.}
    \label{tab:gender_results_S2gpu}
    %\resizebox{\columnwidth}{!}{
        \begin{tabular}{lc|cc|c}
        \specialrule{1.2pt}{0.2pt}{1pt}
        \multicolumn{1}{c}{\multirow{2}{*}{Video}} & \multicolumn{1}{c|}{\multirow{2}{*}{Alg.}} & \multicolumn{2}{c|}{F1-Score} &
        \multicolumn{1}{|c}{\multirow{2}{*}{\begin{tabular}[c]{@{}c@{}}Speed\\ {[}seconds/frame{]}\end{tabular}}} \\
         &  & \multicolumn{1}{c}{Male} & \multicolumn{1}{c|}{Female} \\
        \specialrule{1.2pt}{0.2pt}{1pt}
        \multirow{2}{*}{Airport-1} & A5 &0.81 &0.75 &0.0083$\pm$0.0021 \\ 
        & A6 &0.66 &0.38 &0.0389$\pm$0.0246 \\ \hline 
        \multirow{2}{*}{Airport-2} & A5 &0.62 &0.75 &0.0077$\pm$0.0027 \\ 
        & A6 &0.48 &0.49 &0.0369$\pm$0.0301 \\ \hline 
        \multirow{2}{*}{Airport-3} & A5 &0.66 &0.67 &0.0082$\pm$0.0022 \\ 
        & A6 &0.61 &0.51 &0.0314$\pm$0.0196 \\ \hline 
        \multirow{2}{*}{Airport-4} & A5 &0.71 &0.56 &0.0089$\pm$0.0016 \\ 
        & A6 &0.63 &0.37 &0.0644$\pm$0.0333 \\ \hline \hline 
        \multirow{2}{*}{Mall-1} & A5 &0.69 &0.42 &0.0121$\pm$0.0032 \\ 
        & A6 &0.64 &0.37 &0.3342$\pm$0.1210 \\ \hline 
        \multirow{2}{*}{Mall-2} & A5 &0.78 &0.41 &0.0128$\pm$0.0042 \\ 
        & A6 &0.71 &0.34 &0.3672$\pm$0.1664 \\ \hline 
        \multirow{2}{*}{Mall-3} & A5 &0.58 &0.51 &0.0096$\pm$0.0018 \\ 
        & A6 &0.57 &0.43 &0.1202$\pm$0.0450 \\ \hline 
        \multirow{2}{*}{Mall-4} & A5 &0.47 &0.32 &0.0097$\pm$0.0018 \\ 
        & A6 &0.45 &0.23 &0.1325$\pm$0.0517 \\ \hline \hline 
        \multirow{2}{*}{Pedestrian-1} & A5 &0.56 &0.66 &0.0098$\pm$0.0018 \\ 
        & A6 &0.59 &0.72 &0.1318$\pm$0.0540 \\ \hline 
        \multirow{2}{*}{Pedestrian-2} & A5 &0.77 &0.48 &0.0102$\pm$0.0020 \\ 
        & A6 &0.71 &0.40 &0.1435$\pm$0.0677 \\ \hline 
        \multirow{2}{*}{Pedestrian-3} & A5 &0.54 &0.48 &0.0094$\pm$0.0015 \\ 
        & A6 &0.49 &0.20 &0.0910$\pm$0.0381 \\ \hline 
        \multirow{2}{*}{Pedestrian-4} & A5 &0.76 &0.59 &0.0092$\pm$0.0018 \\ 
        & A6 &0.70 &0.26 &0.0875$\pm$0.0444 \\ \hline 
        \multirow{2}{*}{Pedestrian-5} & A5 &0.39 &0.29 &0.0092$\pm$0.0020 \\ 
        & A6 &0.38 &0.23 &0.0886$\pm$0.0460 \\ \hline \hline 
        \multirow{2}{*}{Subway-1} & A5 &0.59 &0.53 &0.0094$\pm$0.0020 \\ 
        & A6 &0.59 &0.42 &0.0928$\pm$0.0501 \\ \hline 
        \multirow{2}{*}{Subway-2} & A5 &0.51 &0.55 &0.0100$\pm$0.0025 \\ 
        & A6 &0.45 &0.29 &0.1262$\pm$0.0623 \\ \hline 
        \multirow{2}{*}{Subway-3} & A5 &0.65 &0.43 &0.0093$\pm$0.0020 \\ 
        & A6 &0.71 &0.21 &0.0953$\pm$0.0503 \\ \hline 
        \specialrule{1.2pt}{0.2pt}{1pt}
        \multirow{2}{*}{Overall} &A5 &0.63$\pm$0.12 &0.53$\pm$0.13 &0.0096$\pm$0.0013 \\ 
        &A6 &0.58$\pm$0.10 &0.36$\pm$0.13 &0.1239$\pm$0.0923 \\ 
        \specialrule{1.2pt}{0.2pt}{1pt}
        \end{tabular}
        %}%
\end{table}
%=====================

% SYSTEM 2 - CPU
%=====================
\begin{table}[!t]
    \centering
    \footnotesize
    \setlength{\tabcolsep}{1pt}
    \caption{Gender estimation results per video running algorithms in \textbf{System 2} with \textbf{CPU}. KEY -- Ax: algorithm x; F: F1-Score.}
    \label{tab:gender_results_S2cpu}
    %\resizebox{\columnwidth}{!}{
        \begin{tabular}{lc|cc|c}
        \specialrule{1.2pt}{0.2pt}{1pt}
        \multicolumn{1}{c}{\multirow{2}{*}{Video}} & \multicolumn{1}{c|}{\multirow{2}{*}{Alg.}} & \multicolumn{2}{c|}{F1-Score} &
        \multicolumn{1}{|c}{\multirow{2}{*}{\begin{tabular}[c]{@{}c@{}}Speed\\ {[}seconds/frame{]}\end{tabular}}} \\
         &  & \multicolumn{1}{c}{Male} & \multicolumn{1}{c|}{Female} \\
        \specialrule{1.2pt}{0.2pt}{1pt} 
        \multirow{2}{*}{Airport-1} & A5 &0.82 &0.76 &0.0149$\pm$0.0045 \\ 
        & A6 &0.66 &0.38 &0.3990$\pm$0.2348 \\ \hline 
        \multirow{2}{*}{Airport-2} & A5 &0.61 &0.75 &0.0140$\pm$0.0060 \\ 
        & A6 &0.46 &0.48 &0.3745$\pm$0.2805 \\ \hline 
        \multirow{2}{*}{Airport-3} & A5 &0.66 &0.68 &0.0138$\pm$0.0045 \\ 
        & A6 &0.61 &0.51 &0.3248$\pm$0.1970 \\ \hline 
        \multirow{2}{*}{Airport-4} & A5 &0.72 &0.57 &0.0185$\pm$0.0038 \\ 
        & A6 &0.63 &0.38 &0.6903$\pm$0.3353 \\ \hline \hline 
        \multirow{2}{*}{Mall-1} & A5 &0.69 &0.42 &0.0485$\pm$0.0079 \\ 
        & A6 &0.64 &0.38 &4.5413$\pm$0.9187 \\ \hline 
        \multirow{2}{*}{Mall-2} & A5 &0.79 &0.42 &0.0519$\pm$0.0092 \\ 
        & A6 &0.71 &0.36 &4.9023$\pm$1.1083 \\ \hline 
        \multirow{2}{*}{Mall-3} & A5 &0.57 &0.50 &0.0248$\pm$0.0039 \\ 
        & A6 &0.57 &0.44 &1.3990$\pm$0.4074 \\ \hline 
        \multirow{2}{*}{Mall-4} & A5 &0.47 &0.32 &0.0262$\pm$0.0046 \\ 
        & A6 &0.45 &0.23 &1.5869$\pm$0.4928 \\ \hline \hline 
        \multirow{2}{*}{Pedestrian-1} & A5 &0.56 &0.66 &0.0262$\pm$0.0049 \\ 
        & A6 &0.59 &0.72 &1.5863$\pm$0.5587 \\ \hline 
        \multirow{2}{*}{Pedestrian-2} & A5 &0.77 &0.48 &0.0278$\pm$0.0059 \\ 
        & A6 &0.71 &0.38 &1.7533$\pm$0.6561 \\ \hline 
        \multirow{2}{*}{Pedestrian-3} & A5 &0.54 &0.48 &0.0214$\pm$0.0036 \\ 
        & A6 &0.49 &0.20 &0.9879$\pm$0.3604 \\ \hline 
        \multirow{2}{*}{Pedestrian-4} & A5 &0.75 &0.59 &0.0205$\pm$0.0038 \\ 
        & A6 &0.71 &0.27 &0.9375$\pm$0.3629 \\ \hline 
        \multirow{2}{*}{Pedestrian-5} & A5 &0.39 &0.29 &0.0209$\pm$0.0041 \\ 
        & A6 &0.38 &0.22 &0.9538$\pm$0.3963 \\ \hline \hline 
        \multirow{2}{*}{Subway-1} & A5 &0.59 &0.52 &0.0218$\pm$0.0052 \\ 
        & A6 &0.59 &0.42 &1.0687$\pm$0.5277 \\ \hline 
        \multirow{2}{*}{Subway-2} & A5 &0.51 &0.55 &0.0256$\pm$0.0053 \\ 
        & A6 &0.45 &0.30 &1.5076$\pm$0.5511 \\ \hline 
        \multirow{2}{*}{Subway-3} & A5 &0.65 &0.44 &0.0218$\pm$0.0055 \\ 
        & A6 &0.71 &0.20 &1.0611$\pm$0.4969 \\ 
        \specialrule{1.2pt}{0.2pt}{1pt}
        \multirow{2}{*}{Overall} &A5 &0.63$\pm$0.12 &0.53$\pm$0.13 &0.0249$\pm$0.0105 \\ 
        &A6 &0.58$\pm$0.11 &0.37$\pm$0.13 &1.5046$\pm$1.2915 \\ 
        \specialrule{1.2pt}{0.2pt}{1pt}
        \end{tabular}
        %}%
\end{table}
%=====================

% SYSTEM 3 (CPU)
%=====================
\begin{table}[!t]
    \centering
    \footnotesize
    \setlength{\tabcolsep}{1pt}
    \caption{Gender estimation results per video running algorithms in \textbf{System 3} with \textbf{CPU}. KEY -- Ax: algorithm x; F: F1-Score.}
    \label{tab:gender_results_S3}
    %\resizebox{\columnwidth}{!}{
        \begin{tabular}{lc|cc|c}
        \specialrule{1.2pt}{0.2pt}{1pt}
        \multicolumn{1}{c}{\multirow{2}{*}{Video}} & \multicolumn{1}{c|}{\multirow{2}{*}{Alg.}} & \multicolumn{2}{c|}{F1-Score} &
        \multicolumn{1}{|c}{\multirow{2}{*}{\begin{tabular}[c]{@{}c@{}}Speed\\ {[}seconds/frame{]}\end{tabular}}} \\
         &  & \multicolumn{1}{c}{Male} & \multicolumn{1}{c|}{Female} \\
        \specialrule{1.2pt}{0.2pt}{1pt}
        \multirow{2}{*}{Airport-1} & A5 &0.78 &0.77 &0.3712$\pm$0.0888 \\ 
        & A6 &0.64 &0.66 &6.2763$\pm$3.0372 \\ \hline 
        \multirow{2}{*}{Airport-2} & A5 &0.77 &0.85 &0.2993$\pm$0.1638 \\ 
        & A6 &0.59 &0.76 &4.8429$\pm$3.4963 \\ \hline 
        \multirow{2}{*}{Airport-3} & A5 &0.72 &0.75 &0.3171$\pm$0.1477 \\ 
        & A6 &0.59 &0.65 &4.8207$\pm$3.0917 \\ \hline 
        \multirow{2}{*}{Airport-4} & A5 &0.72 &0.64 &0.3824$\pm$0.0867 \\ 
        & A6 &0.57 &0.61 &7.4845$\pm$3.7042 \\ \hline \hline 
        \multirow{2}{*}{Mall-1} & A5 &0.72 &0.66 &0.4311$\pm$0.0587 \\ 
        & A6 &0.58 &0.70 &13.0439$\pm$6.2004 \\ \hline 
        \multirow{2}{*}{Mall-2} & A5 &0.74 &0.64 &0.4638$\pm$0.0694 \\ 
        & A6 &0.53 &0.61 &17.5045$\pm$9.0727 \\ \hline 
        \multirow{2}{*}{Mall-3} & A5 &0.64 &0.76 &0.3664$\pm$0.1072 \\ 
        & A6 &0.51 &0.73 &6.8693$\pm$3.5238 \\ \hline 
        \multirow{2}{*}{Mall-4} & A5 &0.58 &0.65 &0.3676$\pm$0.1051 \\ 
        & A6 &0.48 &0.67 &6.8015$\pm$3.5475 \\ \hline \hline 
        \multirow{2}{*}{Pedestrian-1} & A5 &0.57 &0.78 &0.3981$\pm$0.0635 \\ 
        & A6 &0.52 &0.82 &8.4344$\pm$4.5305 \\ \hline 
        \multirow{2}{*}{Pedestrian-2} & A5 &0.76 &0.63 &0.3827$\pm$0.1205 \\ 
        & A6 &0.66 &0.58 &9.0186$\pm$5.3816 \\ \hline 
        \multirow{2}{*}{Pedestrian-3} & A5 &0.58 &0.56 &0.3941$\pm$0.0871 \\ 
        & A6 &0.52 &0.50 &9.0293$\pm$5.0491 \\ \hline 
        \multirow{2}{*}{Pedestrian-4} & A5 &0.79 &0.71 &0.3958$\pm$0.0800 \\ 
        & A6 &0.75 &0.60 &8.5377$\pm$4.7048 \\ \hline 
        \multirow{2}{*}{Pedestrian-5} & A5 &0.49 &0.42 &0.3970$\pm$0.0677 \\ 
        & A6 &0.60 &0.73 &8.7285$\pm$3.7757 \\ \hline \hline 
        \multirow{2}{*}{Subway-1} & A5 &0.63 &0.60 &0.3838$\pm$0.1510 \\ 
        & A6 &0.59 &0.62 &11.8167$\pm$7.1642 \\ \hline 
        \multirow{2}{*}{Subway-2} & A5 &0.58 &0.65 &0.4104$\pm$0.0993 \\ 
        & A6 &0.57 &0.68 &11.8930$\pm$5.1045 \\ \hline 
        \multirow{2}{*}{Subway-3} & A5 &0.64 &0.46 &0.4132$\pm$0.0934 \\ 
        & A6 &0.77 &0.51 &12.1132$\pm$5.1922 \\ 
        \specialrule{1.2pt}{0.2pt}{1pt}
        \multirow{2}{*}{Overall} &A5 &0.67$\pm$0.09 &0.66$\pm$0.11 &0.3859$\pm$0.0380 \\ 
        &A6 &0.59$\pm$0.08 &0.65$\pm$0.08 &9.2009$\pm$3.2449 \\ 
        \specialrule{1.2pt}{0.2pt}{1pt}
        \end{tabular}
        %}%
\end{table}
%=====================

% SYSTEM 4 (GPU)
%=====================
\begin{table}[!t]
    \centering
    \footnotesize
    \setlength{\tabcolsep}{1pt}
    \caption{Gender estimation results per video running algorithms in \textbf{System 4} with \textbf{GPU}. KEY -- Ax: algorithm x; F: F1-Score. Note that A6 cannot run in System 4 due to lack of memory.}
    \label{tab:gender_results_S4}
    %\resizebox{\columnwidth}{!}{
        \begin{tabular}{lc|cc|c}
        \specialrule{1.2pt}{0.2pt}{1pt}
        \multicolumn{1}{c}{\multirow{2}{*}{Video}} & \multicolumn{1}{c|}{\multirow{2}{*}{Alg.}} & \multicolumn{2}{c|}{F1-Score} &
        \multicolumn{1}{|c}{\multirow{2}{*}{\begin{tabular}[c]{@{}c@{}}Speed\\ {[}seconds/frame{]}\end{tabular}}} \\
         &  & \multicolumn{1}{c}{Male} & \multicolumn{1}{c|}{Female} \\
        \specialrule{1.2pt}{0.2pt}{1pt}
        \multirow{1}{*}{Airport-1}  & A5 &0.82 &0.76 &0.0722$\pm$0.3782 \\ 
        \multirow{1}{*}{Airport-2} & A5 &0.61 &0.74 &0.0675$\pm$0.4078 \\ 
        \multirow{1}{*}{Airport-3} & A5 &0.66 &0.68 &0.0695$\pm$0.4311 \\ 
        \multirow{1}{*}{Airport-4} & A5 &0.72 &0.57 &0.0809$\pm$0.4252 \\ \hline \hline
        \multirow{1}{*}{Mall-1} & A5 &0.69 &0.42 &0.1772$\pm$0.4627 \\ 
        \multirow{1}{*}{Mall-2} & A5 &0.78 &0.42 &0.2085$\pm$0.5110 \\ 
        \multirow{1}{*}{Mall-3} & A5 &0.57 &0.50 &0.0958$\pm$0.5587 \\ 
        \multirow{1}{*}{Mall-4} & A5 &0.47 &0.32 &0.0915$\pm$0.4238 \\ \hline \hline
        \multirow{1}{*}{Pedestrian-1} & A5 &0.56 &0.67 &0.0907$\pm$0.4169 \\ 
        \multirow{1}{*}{Pedestrian-2} & A5 &0.77 &0.48 &0.1007$\pm$0.4440 \\ 
        \multirow{1}{*}{Pedestrian-3} & A5 &0.55 &0.49 &0.0824$\pm$0.4130 \\ 
        \multirow{1}{*}{Pedestrian-4} & A5 &0.76 &0.60 &0.0874$\pm$0.4827 \\ 
        \multirow{1}{*}{Pedestrian-5} & A5 &0.39 &0.29 &0.0977$\pm$0.5495 \\ \hline \hline
        \multirow{1}{*}{Subway-1} & A5 &0.59 &0.53 &0.0949$\pm$0.4157 \\ 
        \multirow{1}{*}{Subway-2} & A5 &0.50 &0.55 &0.1135$\pm$0.5004 \\ 
        \multirow{1}{*}{Subway-3} & A5 &0.65 &0.42 &0.0850$\pm$0.4085 \\ 
        \specialrule{1.2pt}{0.2pt}{1pt}
        \multirow{1}{*}{Overall} &A5 &0.63$\pm$0.12 &0.53$\pm$0.14 &0.1010$\pm$0.0370 \\ 
        \specialrule{1.2pt}{0.2pt}{1pt}
        \end{tabular}
        %}%
\end{table}
%=====================

\EOD
